# Supplementary material for: AutoPrep: Natural Language Question-Aware Data Preparation with a Multi-Agent Framework
Source: arXiv:2412.10422 source file (2025-07-09)
Supplement: Supplementary file 1 [file _root.tex]

%!TEX root = ../main.tex

\clearpage
\newpage
\appendix

%!TEX root = ../../main.tex
\begin{figure}[!t]
    \centering 
    \includegraphics[width=0.99\columnwidth]{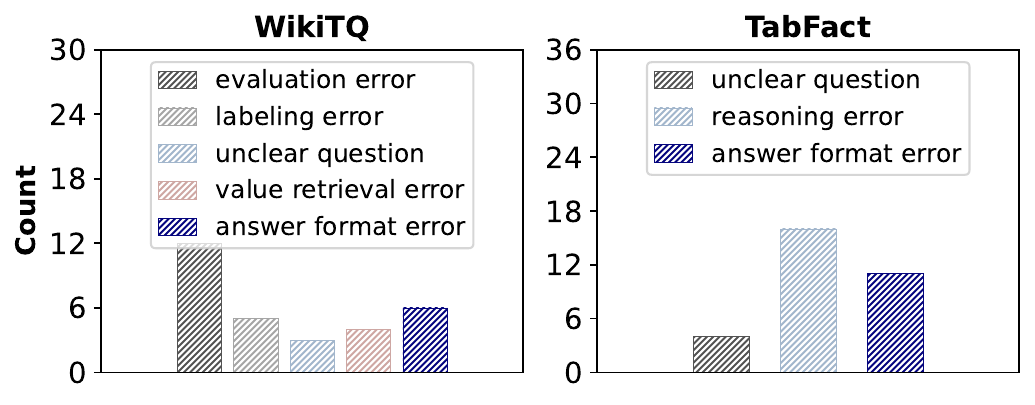}
    \vspace{-1em}
    \caption{{In-depth Analysis of the ``\term{Other}'' Category.}
    %, such as NL2SQL as shown in the figure. \sys decomposes the data prep process into three stages: \textcircled{1} The Planning stage, \textcircled{2} the Programming stage and \textcircled{3} the Executing stage.
    }
    \label{fig:subcategories_in_other}
    % \vspace{-1em}
\end{figure}

\section{Details of the Error Analysis}
\label{sec:appendix_details_of_error_analysis}

This section presents details of the error analysis shown in Figure~\ref{fig:error_instance_record}, which motivates us to study question-aware data prep.

\stitle{TQA Method: NL2SQL Based on GPT-4.}
We adopt NL2SQL~\cite{rajkumar2022evaluating}, a representative TQA baseline that does not perform data prep, as introduced in Section~\ref{subsec:exp-setup}. Specifically, given a natural language question $Q$ and a table $T$, we prompt GPT-4 to generate an SQL query $\term{SQL}$ using a few-shot in-context learning strategy. The query is then executed on $T$ to obtain the final answer $Ans$ for $Q$.

\stitle{Error Categorization.}
We recruite three graduate students from our university's database group to annotate error categories for a randomly sampled set of 500 instances from WikiTQ and TabFact. All annotators have a good understanding of the TQA task and are proficient in SQL syntax.
We instruct the annotators to first identify errors stemming from insufficient data prep, assigning any remaining errors to a default category labeled \term{Other}. For the data prep-related errors, after careful investigation, we further categorize them into the following three types:
(1) \textbf{Missing Semantics:} The table lacks necessary semantic information required to accurately answer the NL question. 
(2) \textbf{Inconsistent Values:} Values within a column are represented inconsistently across different records. 
(3) \textbf{Irrelevant Columns:} The table includes many columns, but only a small subset are actually relevant to the NL question. 

\stitle{In-depth Analysis of the ``\term{Other}'' Category}. 
We report the detailed sub-categories within the ``\term{Other}'' category in Figure~\ref{fig:subcategories_in_other}. As shown, for WikiTQ, more than half of the cases stem from issues inherent to the dataset itself. Notably, 40\% of the errors are due to limitations in the evaluation function, where semantically equivalent but non-identical responses are marked as incorrect, a problem also highlighted in~\cite{cheng2023binding}. Additionally, 20\% of the errors arise from formatting issues in the model’s responses, where the generated SQL logic is correct but the output includes extraneous values from irrelevant columns.
On the other hand, for the TabFact dataset, most errors are attributed to model reasoning failures. Over 50\% result from the model’s inability to generate logically complete and accurate SQL queries. Furthermore, more than 35\% of the errors are due to response formatting issues, where the model returns ambiguous values instead of definitive true/false answers.

\section{More Experiments}
\label{sec:statistics_of_in_depth_analysis}

\subsection{Evaluation on Various Table Sizes}

\stitle{Exp:
% \expnum\label{exp:evaluate_on_tables_with_various_sizes}
Evaluation of \sys on tables with various sizes.} 
To further investigate \sys, we analyze its performance across tables of varying sizes.
While all tables in TabFact are small, we categorize the tables in WikiTQ into Small (fewer than 2048 tokens), Medium (2048 to 4096 tokens), and Large (more than 4096 tokens), resulting in 4040 Small
tables, 200 Medium tables, and 104 Large tables.
The results are reported in Figure~\ref{fig:accuracy_on_different_size_tables}.

We observe that all baselines exhibit unstable performance, particularly on larger tables. For instance, although CoTable achieves the highest average accuracy among previous SOTA methods, it suffers an accuracy drop of {\textbf{11.78}} when reasoning over large tables. Likewise, ReAcTable shows relatively stable performance on medium tables (dropping by {\textbf{2.15}}), yet its performance on large tables remains unsatisfactory (dropping by {\textbf{17.53}}).

% %!TEX root = ../../main.tex
% % \begin{figure}[!t]
% %     \centering 
% %     \includegraphics[width=0.99\columnwidth]{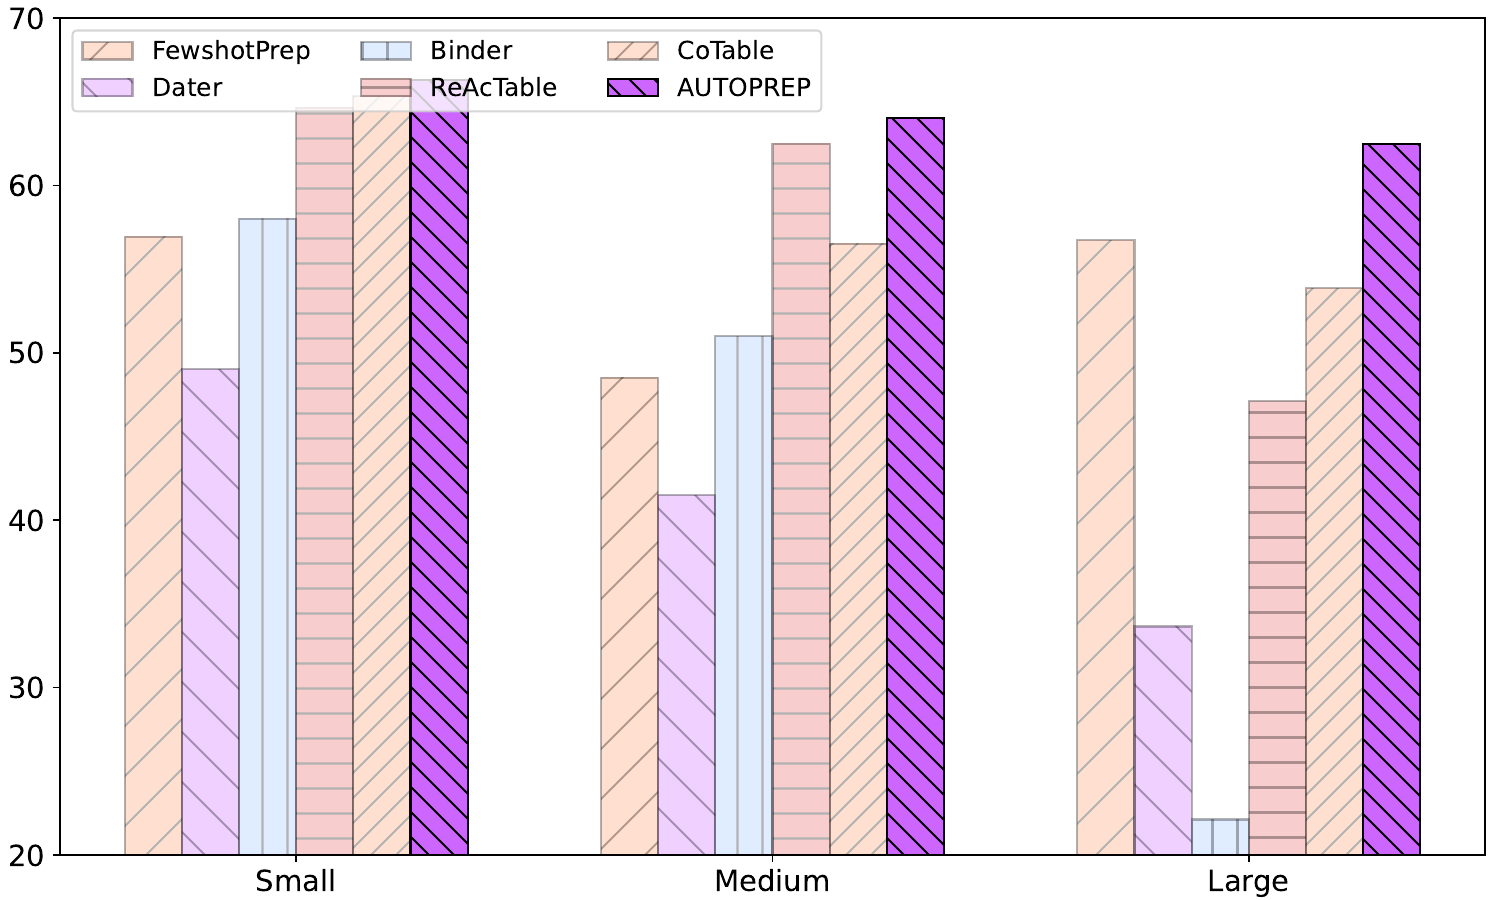}
% %     \vspace{-1em}
% %     \caption{}
% %     \label{fig:comparison_of_methods_on_table_size}
% %     \vspace{-1em}
% % \end{figure}

% \begin{figure}[!t]
%     % \vspace{-1em}
%     \centering
%     \begin{subfigure}{0.32\columnwidth}
%         \includegraphics[width=\textwidth]{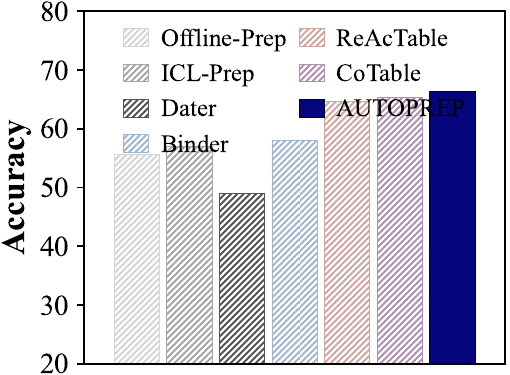}
%         \captionsetup{skip=-0.3pt}
%         \caption{Small}
%         \label{fig:accuracy_on_small_tables}
%     \end{subfigure}
%     \hspace{0.2mm}
%     % \quad
%     \begin{subfigure}{0.32\columnwidth}
%         \includegraphics[width=\textwidth]{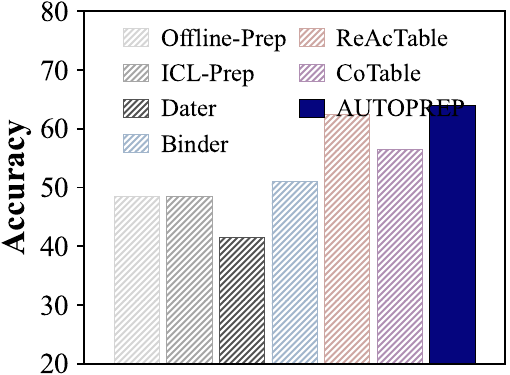}
%         \captionsetup{skip=-0.3pt}
%         \caption{Medium}
%         \label{fig:accuracy_on_medium_tables}
%     \end{subfigure}
%     \hspace{0.2mm}
%     % \quad
%     \begin{subfigure}{0.32\columnwidth}
%         \includegraphics[width=\textwidth]{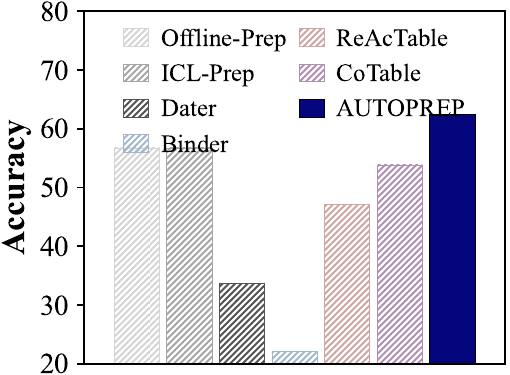}
%         \captionsetup{skip=-0.3pt}
%         \caption{Large}
%         \label{fig:accuracy_on_large_tables}
%     \end{subfigure}
%     \vspace{-2em}
%     \caption{\revise{Comparison of \sys and other data prep methods on tables with different sizes on the WikiTQ dataset.}}
%     \label{fig:comparison_of_methods_on_table_size}
%     \vspace{-1em}
% \end{figure}

%!TEX root = ../../main.tex
\begin{figure}[!t]
    \centering 
    \includegraphics[width=0.99\columnwidth]{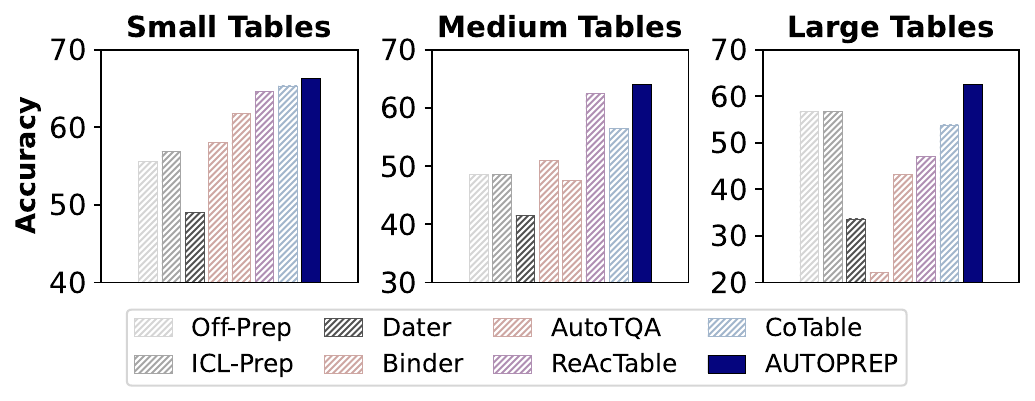}
    \vspace{-1em}
    \caption{{Accuracy on different size of tables in WikiTQ.}
    %, such as NL2SQL as shown in the figure. \sys decomposes the data prep process into three stages: \textcircled{1} The Planning stage, \textcircled{2} the Programming stage and \textcircled{3} the Executing stage.
    }
    \label{fig:accuracy_on_different_size_tables}
    % \vspace{-1em}
\end{figure}

In contrast, \sys achieves the highest and most stable performance across tables of varying sizes. When processing medium and large tables, the accuracy of \sys drops by {\textbf{2.29}} and {\textbf{3.79}}.
The key to its stability is that it employs specialized agents for each data prep task, mitigating the issue of exceeding prompt length limits. Furthermore, each agent generates program-based operators to handle data prep on the entire table, thereby avoiding information loss that occurs when large tables are cropped.

\stitle{Finding:
% \findingnum\label{finding:evaluate_on_tables_with_various_sizes}
By employing multiple agents and program-based operations, \sys maintains stable performance as table size grows, ensuring that each data prep task is handled effectively without overwhelming a single model.}

\subsection{Evaluation on Various Question Difficulties}

%!TEX root = ../main.tex
\begin{table}[t!]
  \centering
  \caption{\bf{In-depth Analysis of \sys and all baselines when varying question difficulties on WikiTQ and TabFact.}}
  \vspace{-0.5em}
  \scalebox{0.88} {
    \begin{tabular}{|c||c|c|c|c|}
      \hline
      \multirow{2}{*}{\textbf{Method}} & \multicolumn{2}{c|}{\textbf{WikiTQ}} & \multicolumn{2}{c|}{\textbf{TabFact}} \\ \cline{2-5}
                              & \textbf{Simple}                                                         & \textbf{Complex}    & \textbf{Simple}                                                         & \textbf{Complex}     \\
      \hline \hline
      End2End                 & ${57.80}$                                                    & ${55.68}$                                                               & $86.51$  & $77.07$             \\ \hline
      CoT                     & $56.85$                                                                & $55.33$                                                               & ${84.92}$                                                             & ${79.13}$            \\ \hline
      NL2Py                 & ${61.87}$                                                                & ${57.21}$                                                       & $70.83$                                                    & $65.45$  \\ \hline
      NL2SQL                  & $57.02$                                                                & $49.13$                                                               & $70.83$                                                    & $69.59$    \\
      \hline \hline
      ICL-Prep                & ${59.51}$                                                                & ${54.02}$                                                     & $82.64$                                                             & ${78.44}$     \\\hline
	  Dater                   & $51.33$                                                                & $45.77$                                                             & $88.39$ & $77.76$ 														           \\ \hline
      Binder                  & $62.02$                                                                & $52.04$                                                               & $89.29$                                                             & $76.38$                      \\ \hline
      ReAcTable               & ${66.98}$                                                                & ${61.71}$                                                   & ${90.48}$                                                 & ${79.72}$  \\ \hline
      CoTable                 & ${66.88}$                                                                & ${62.53}$                                                     & ${90.58}$                                                    & ${81.89}$     \\ 
      \hline \hline
      AP {\small + End2End}			 & $66.58$ 
								{\scriptsize \textcolor{cadmiumgreen}{($+8.78$)}}   
								& $60.23$ 
								{\scriptsize \textcolor{cadmiumgreen}{($+4.55$)}}             
								& $\underline{87.20}$ 
								{\scriptsize \textcolor{cadmiumgreen}{($+0.69$)}}           
								& $77.07$ 
								{\scriptsize \textcolor{cadmiumgreen}{($+0.00$)}}           
								\\ \hline
      {\small + CoT    }        & $64.12$ 
								{\scriptsize \textcolor{cadmiumgreen}{($+7.27$)}}   
								& $58.57$ 
								{\scriptsize \textcolor{cadmiumgreen}{($+5.24$)}}               
								& $84.52$ 
								{\scriptsize \textcolor{dropred}{($-0.40$)}}           
								& $80.02$ 
								{\scriptsize \textcolor{cadmiumgreen}{($+0.89$)}}             
								\\ \hline
      {\small + NL2Py}       		 & $\underline{68.09}$ 
								{\scriptsize \textcolor{cadmiumgreen}{($+6.22$)}}   
								& $\textbf{63.97}$ 
								{\scriptsize \textcolor{cadmiumgreen}{($+6.76$)}}     
								  & $\textbf{90.77}$ 
								  {\scriptsize \textcolor{cadmiumgreen}{($+19.94$)}} 
								  & $\underline{83.96}$ 
								  {\scriptsize \textcolor{cadmiumgreen}{($+18.51$)}}  
								  \\ \hline
      {\small + NL2SQL }         & $\textbf{69.17}$ 
								{\scriptsize \textcolor{cadmiumgreen}{($+11.97$)}}   
								& $\underline{63.50}$ 
								{\scriptsize \textcolor{cadmiumgreen}{($+14.37$)}}   
							  & $\textbf{90.77}$ 
							  {\scriptsize \textcolor{cadmiumgreen}{($+19.94$)}} 
							  & $\textbf{84.94}$ 
							  {\scriptsize \textcolor{cadmiumgreen}{($+15.35$)}}
							  \\
      \hline
    \end{tabular}
  }
   % \vspace{-1em}  
  \label{tbl:indepth_analysis_question_difficulty}
\end{table}

Also, following previous work~\cite{ye2023large,wang2024chain}, we compare \sys and all baseline models on questions with different difficulties.

\noindent
\textbf{Exp: How does \sys and other baselines perform on question with different difficulties?} We divide the TabFact dataset based on officially provided question difficulty labels. 
Since WikiTQ does not provide difficulty labels, we divide the dataset based on question length following previous work~\cite{ye2023large}.

As shown in Table~\ref{tbl:indepth_analysis_question_difficulty}, CoTable achieves the best performance among all baselines on both Simple and Complex questions, indicating its abilities of complex reasoning abilities over tables. While \sys still outperforms CoTable, especially on Complex questions. Specifically, \sys outperforms CoTable by 0.21\% on Simple questions and 3.72\% on Complex questions.

Moreover, notice that trivial performance improvement is achieved by \sys for Direct Prompting methods. Especially for CoT on Simple questions, the performance of CoT has been dropped by 0.47\% when integrated with \sys. This is because tables of TabFact are all small tables, data prep operations of \sys fail to bring obvious benefit for Direct Prompting methods. While for Code Generation methods, data quality is a critical problem. Thus, NL2Code and NL2SQL have achieved obvious performance gains on prepared tables.

\subsection{Impact of LLM-Based $\mathtt{CustomCode}$}

\begin{table}[t]
    \centering
    \caption{\bf{Analyzing LLM generated code for logical operator.}}
    \label{tbl:llm_code_for_op_analysis}
    \vspace{-0.5em}
    \resizebox{0.65\linewidth}{!}{
    \begin{tabular}{|c||c|}
        \hline
        \textbf{Method} & ~\textbf{WikiTQ}~  \\ \hline \hline
        $\mathtt{CustomCode}$ ratio & ${1.08\%}$  \\ \hline
        $\mathtt{CustomCode}$ accuracy & ${55.32\%}$ \\ \hline \hline
        
        \sys w. $\mathtt{CustomCode}$ & $\textbf{66.09}$\\ \hline
        \sys w.o. $\mathtt{CustomCode}$ & ${65.63}$  \\ 
        \hline
    \end{tabular}
    }
\end{table}

% 47 个case调用$\mathtt{CustomCode}$

\noindent
\stitle{Exp
% \expnum\label{exp:generalization_exp_new_physical_op}
: How does LLM-based $\mathtt{CustomCode}$ help \sys generalize to cases requiring new physical operations?} As discussed in Section~\ref{subsec:prog-idea}, we prompt the LLM to write code to implement the logical operation if no suitable function in the function pool can meet the requirement, which we denote as $\mathtt{CustomCode}$. We quantify the usage frequency of $\mathtt{CustomCode}$ and evaluate whether $\mathtt{CustomCode}$ produces the correct code on WikiTQ.
%its input and output using a powerful LLM DeepSeek-V3, calculating its accuracy. 
We also evaluate the performance of \sys without $\mathtt{CustomCode}$ design. 

As shown in Table~\ref{tbl:llm_code_for_op_analysis}, 
The results show that $\mathtt{CustomCode}$ is invoked in 1.08\% of cases, achieving an accuracy of 55.32\%. Notably, removing $\mathtt{CustomCode}$ leads to a performance drop of \textbf{0.46}  points (from 66.09 to 65.63). These results indicate that, despite its relatively low invocation frequency and moderate accuracy, $\mathtt{CustomCode}$ improves generalization of \sys, particularly in handling new or unforeseen physical operations.

%As shown in Table~\ref{tbl:llm_code_for_op_analysis}, \sys uses $\mathtt{CustomCode}$ with a frequency of 1.08\% and an accuracy of 55.32\% on WikiTQ. In addition, when ablating the $\mathtt{CustomCode}$, the performance of \sys on WikiTQ drops by 0.46. The experimental results show that the despite relatively low usage frequency and accuracy of $\mathtt{CustomCode}$, it still enhances the system's generalization especially in cases that require new physical operators.

\stitle{Finding 
% \findingnum\label{finding:generalization_exp_new_physical_op}
: $\mathtt{CustomCode}$ improves the generalization of \sys on cases requiring new physical operations.}

% \subsection{Evaluation on Generalizability}

% \input{tables/indepth_analysis_generalization}

\subsection{Analysis on Other Data Quality Issues}
\label{subsec_appendix:analysis_on_other_data_quality_issues}

We have conducted a \textbf{new experiment} to analyze the impact of missing values and duplication in TQA tasks on the WikiTQ dataset.
% (our main change \textbf{M\ref{modify:new-exps} (7)}). 

Specifically, for duplication, we first examine all tables containing duplicated records using a heuristic method from~\cite{fan2024cost} on the WikiTQ dataset, and only obtain 24 such instances. Then, we manually remove the duplicate records and re-evaluate \sys’s performance on the updated dataset. The results remain unchanged (accuracy: 70.83\% for both the original and de-duplicated datasets), suggesting that duplication is not a critical issue on existing TQA benchmarking datasets. Similarly, for missing values, we prompt LLMs to impute the missing entries based on the available data for all tables and then re-evaluate \sys on the imputated dataset. The results also show insignificant difference (65.00\% w/o imputation vs. 64.33\% with imputation), indicating that missing values have limited impact.

These above results suggest that such data preparation issues are uncommon and have little effect on existing TQA benchmarking datasets. This is largely due to the way of constructing the datasets. Specifically, during dataset construction~\cite{chen2019tabfact, pasupat2015compositional, wu2024tablebench}, annotators are instructed to first generate natural language questions based on a given table and then derive the corresponding answers directly from the same table. This construction paradigm implicitly ensures data completeness and consistency, as annotators tend to avoid crafting questions around missing or duplicating information. As a result, common data quality issues such as missing values and duplicate records are naturally excluded from the dataset, making them less relevant in the context of existing TQA tasks.

Nevertheless, we acknowledge that issues such as missing values and duplicates are common in real-world datasets, we leave the exploration of these broader data prep challenges to future work.

\stitle{Finding 
% \findingnum\label{finding:generalization_exp_new_physical_op}
: While issues such as missing values and duplicates are common in real-world datasets, they are significantly less prevalent than the three highlighted challenges in existing TQA benchmarks.}

\section{A Running Example of AUTOPREP}
\label{sec:appendix_a_running_example_of_autoprep}

\begin{figure*}[t]
    % \vspace{-1em}
    \centering
    \begin{subfigure}{0.48\textwidth}
        \includegraphics[width=\textwidth]{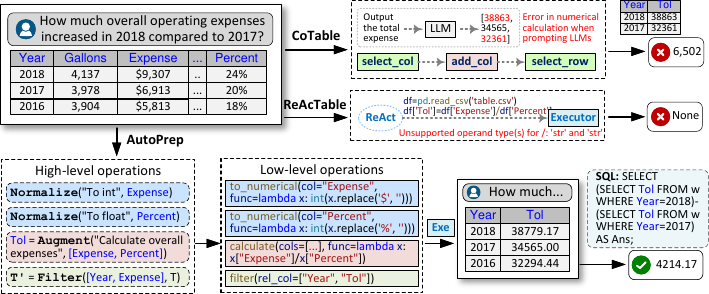}
        % \captionsetup{skip=0.5pt}
        \caption{Case one}
        \label{fig:case_study1}
    \end{subfigure}
    \hspace{-1mm}
    \quad \quad
    \begin{subfigure}{0.48\textwidth}
        \includegraphics[width=\textwidth]{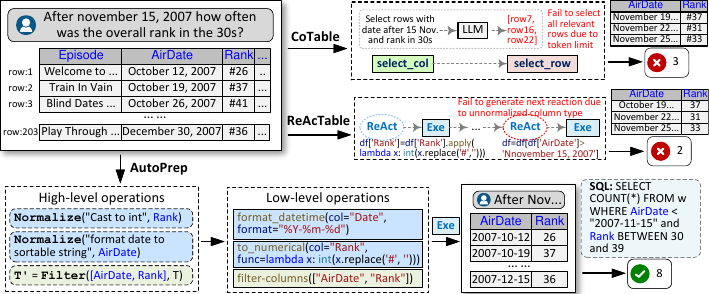}
        % \captionsetup{skip=0.5pt}
        \caption{Case two}
        \label{fig:case_study2}
    \end{subfigure}
    \vspace{-2.5em}
    \caption{{Two case studies selected from TabBench and WikiTQ to qualitatively analyze effectiveness of \sys.}}
    \label{fig:case_study}
    \vspace{-1em}
\end{figure*}

%Based on the experimental results, \sys outperforms the two most powerful TQA methods ReAcTable and CoTable. 

This section presents two illustrative examples from TabBench and WikiTQ to qualitatively analyze effectiveness of \sys. 

To answer the question in Figure~\ref{fig:case_study1}, CoTable generates an operator chain with an ``add\_col'' operator, which is used to generate a new column \term{Tol} based on the division results of two existing columns \term{Expense} and \term{Percent}. This operator directly prompts an LLM to output a list containing all values of the new column, which is a challenging task for previous LLMs. Thus, CoTable generates a new column with two wrong values which leads to a wrong answer. For ReAcTable, although it generates a logically correct Python program, it ignores the types of existing columns which do not support for numerical calculation. Thus, ReAcTable also fails to derive the \term{Tol} column.
\sys addresses this issue by first utilizing a \textsc{Planner} agent to generate logical operators specifying data prep requirements, i.e., two $\mathtt{Normalize}$ to normalize column \term{Expense} and \term{Percent}, a $\mathtt{Derive}$ to generate the overall expenses \term{Tol} and a $\mathtt{Filter}$ to select related columns \term{Year} and \term{Tol}. 
These logical operators are passed to \textsc{Programmer} agents to generate physical operators consisting of a pre-defined Python function. For example, we call $\mathtt{to\mbox{-}numerical}$ function two times to cast \term{Expense} and \term{Percent} to numerical values.
All physical operators are executed to process the original table and output a prepared table. Finally, an \textsc{Analyzer} agent based on NL2SQL method generates a SQL query to extract the correct answer ``4214.17''.

Figure~\ref{fig:case_study2} illustrates a TQA instance involving large tables and inconsistent values. 
%To answer the question, CoTable selects all relevant rows for the question. However, it loses related information due to the maximum input token limitation. Specifically, the table is cropped to include only the first 100 rows to fit within the prompt. Thus, all data in the last 103 rows is lost. Consequently, it generates a sub-table table with incomplete data, resulting in an incorrect answer ``3''. For ReAcTable, it reacts in multiple steps to process the table. When filtering records with \term{Date} after ``november 15, 2007'', it does not transform the \term{Date} into comparable format before using operator ``$>$'' to filter the records. Thus, ReAcTable also generates an error answer.
\sys solves this by splitting the TQA question into two phases, i.e., data prep and data analysis. It first generates logical operators including two $\mathtt{Normalize}$ and one $\mathtt{Filter}$. Next, the \textsc{Programmer} agents implement them with corresponding physical operators, which are executed to produce a prepared table. Based on this, the \textsc{Analyzer} agent extracts the final answer ``8''.

\section{Prompts in \sys}
\label{appendix:prompts_in_autoprep}

The representative demonstration examples and prompts used by \sys are presented. 

\subsection{Prompts in Planner Agent}

%!TEX root = ../../main.tex
\begin{figure*}[!t]
    \centering 
    \includegraphics[width=0.85\textwidth]{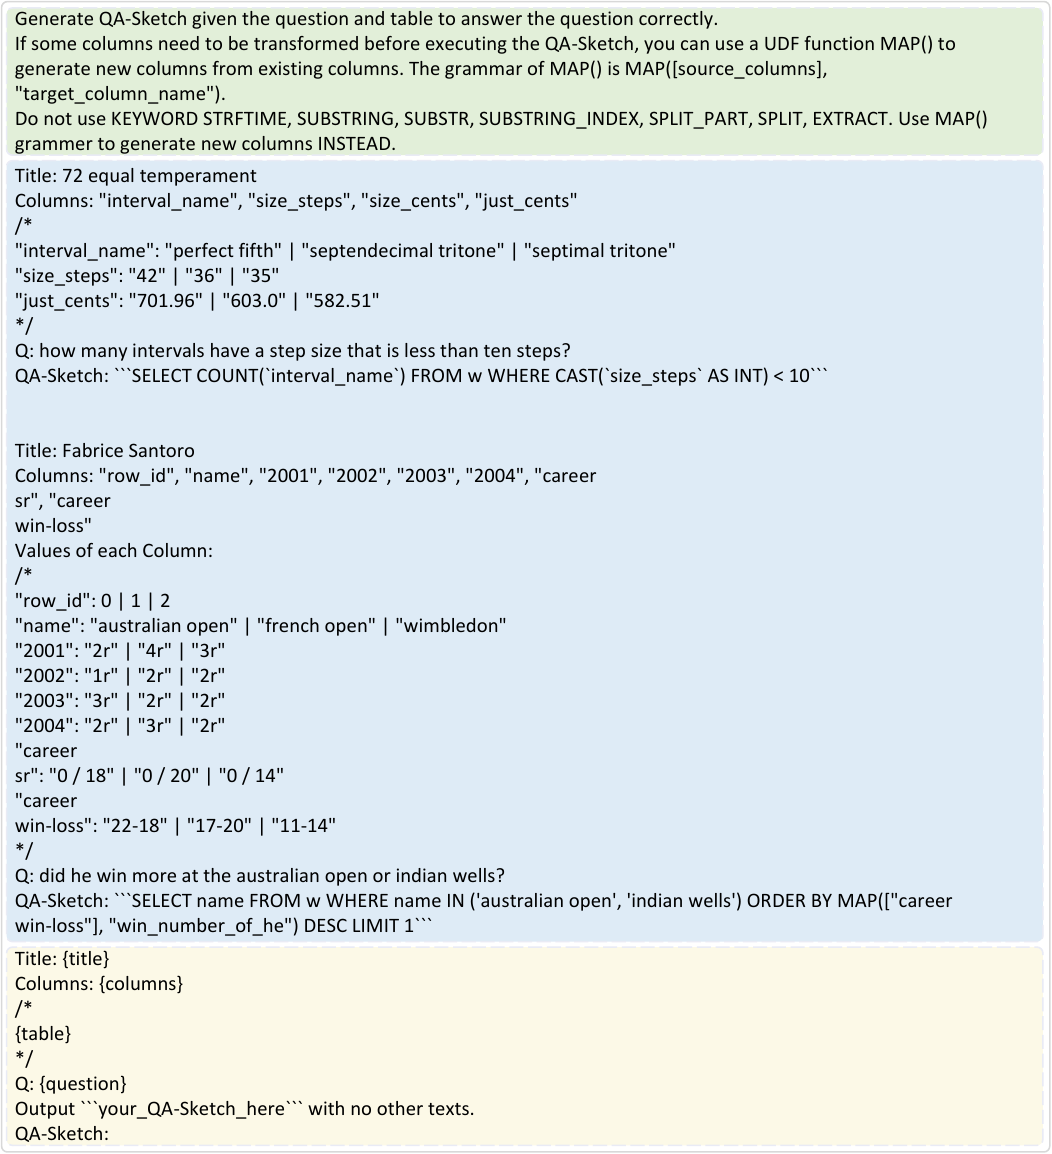}
    \vspace{-1em}
    \caption{Prompt of Planner on generating Analysis Sketch on WikiTQ Dataset.
    %, such as NL2SQL as shown in the figure. \sys decomposes the data prep process into three stages: \textcircled{1} The Planning stage, \textcircled{2} the Programming stage and \textcircled{3} the Executing stage.
    }
    \label{fig:prompt_planner_analysis_sketch_wikitq}
    % \vspace{-1em}
\end{figure*}
%!TEX root = ../../main.tex
\begin{figure*}[!t]
    \centering 
    \includegraphics[width=0.90\textwidth]{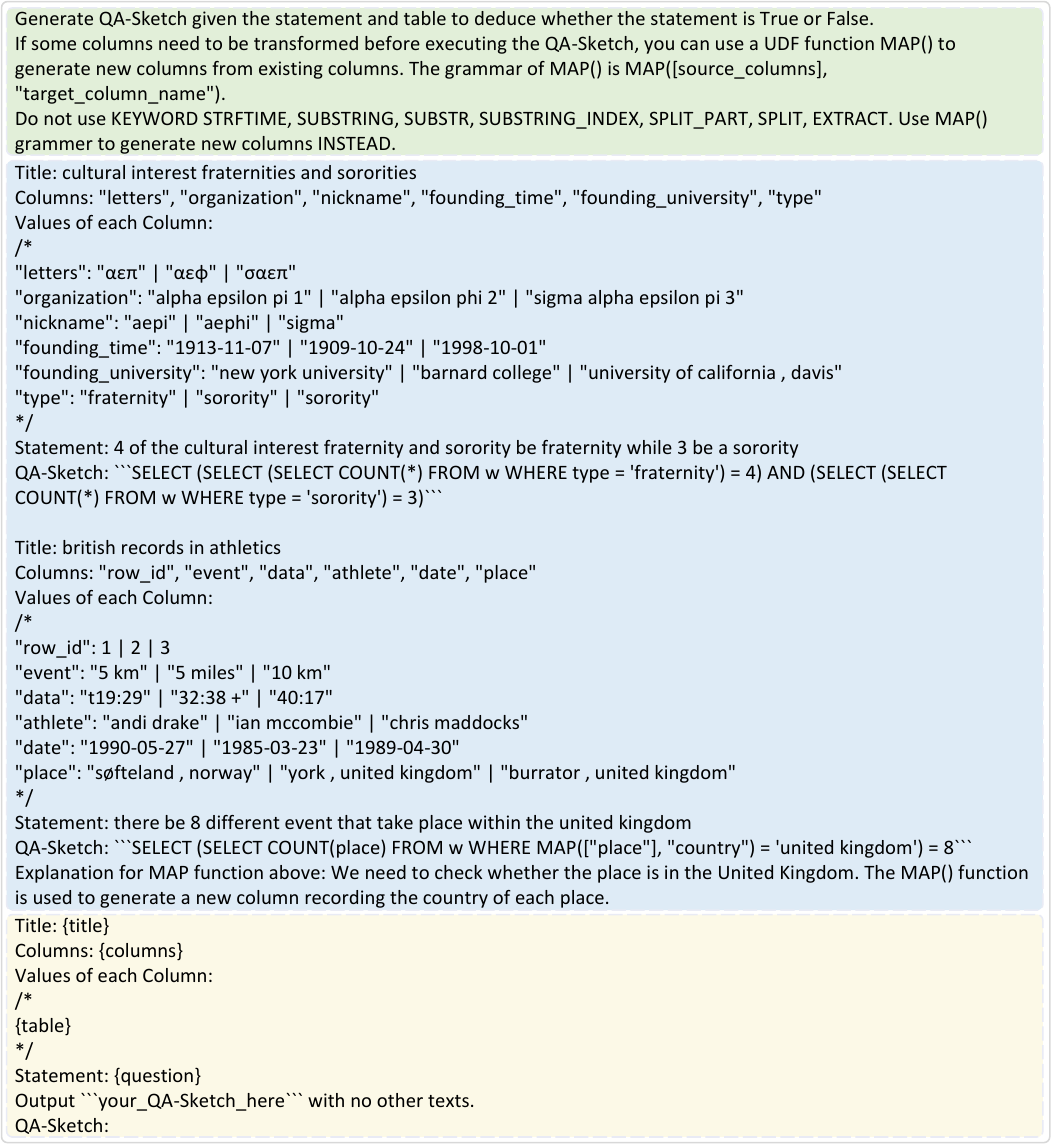}
    \vspace{-1em}
    \caption{Prompt of Planner on generating Analysis Sketch on TabFact Dataset.
    %, such as NL2SQL as shown in the figure. \sys decomposes the data prep process into three stages: \textcircled{1} The Planning stage, \textcircled{2} the Programming stage and \textcircled{3} the Executing stage.
    }
    \label{fig:prompt_planner_analysis_sketch_tabfact}
    % \vspace{-1em}
\end{figure*}

%!TEX root = ../../main.tex
\begin{figure*}[!t]
    \centering 
    \includegraphics[width=0.9\textwidth]{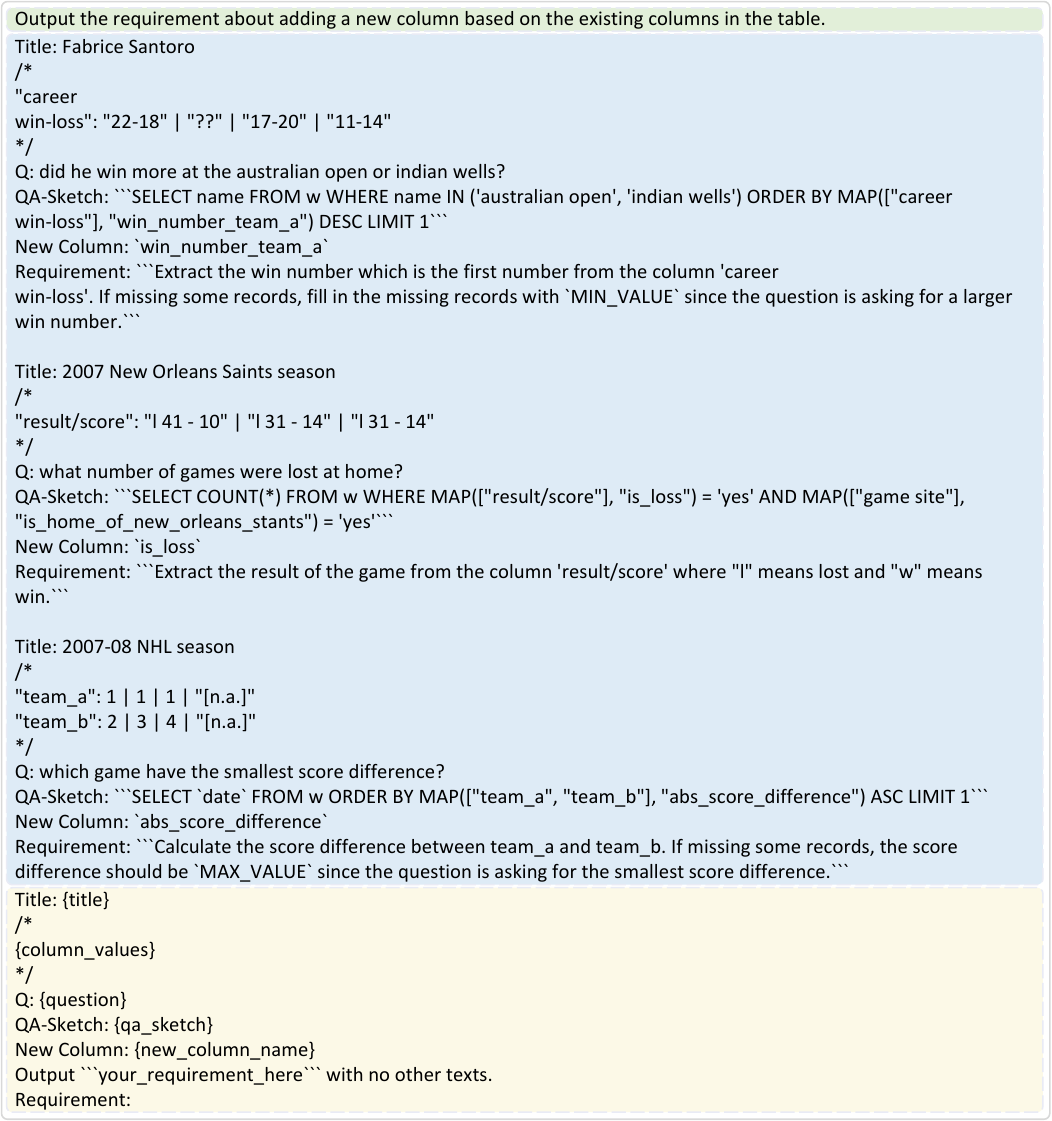}
    \vspace{-1em}
    \caption{Prompt of Planner on generating requirement for Derive Operator.
    %, such as NL2SQL as shown in the figure. \sys decomposes the data prep process into three stages: \textcircled{1} The Planning stage, \textcircled{2} the Programming stage and \textcircled{3} the Executing stage.
    }
    \label{fig:prompt_planner_generate_req_aug}
    % \vspace{-1em}
\end{figure*}
%!TEX root = ../../main.tex
\begin{figure*}[!t]
    \centering 
    \includegraphics[width=0.9\textwidth]{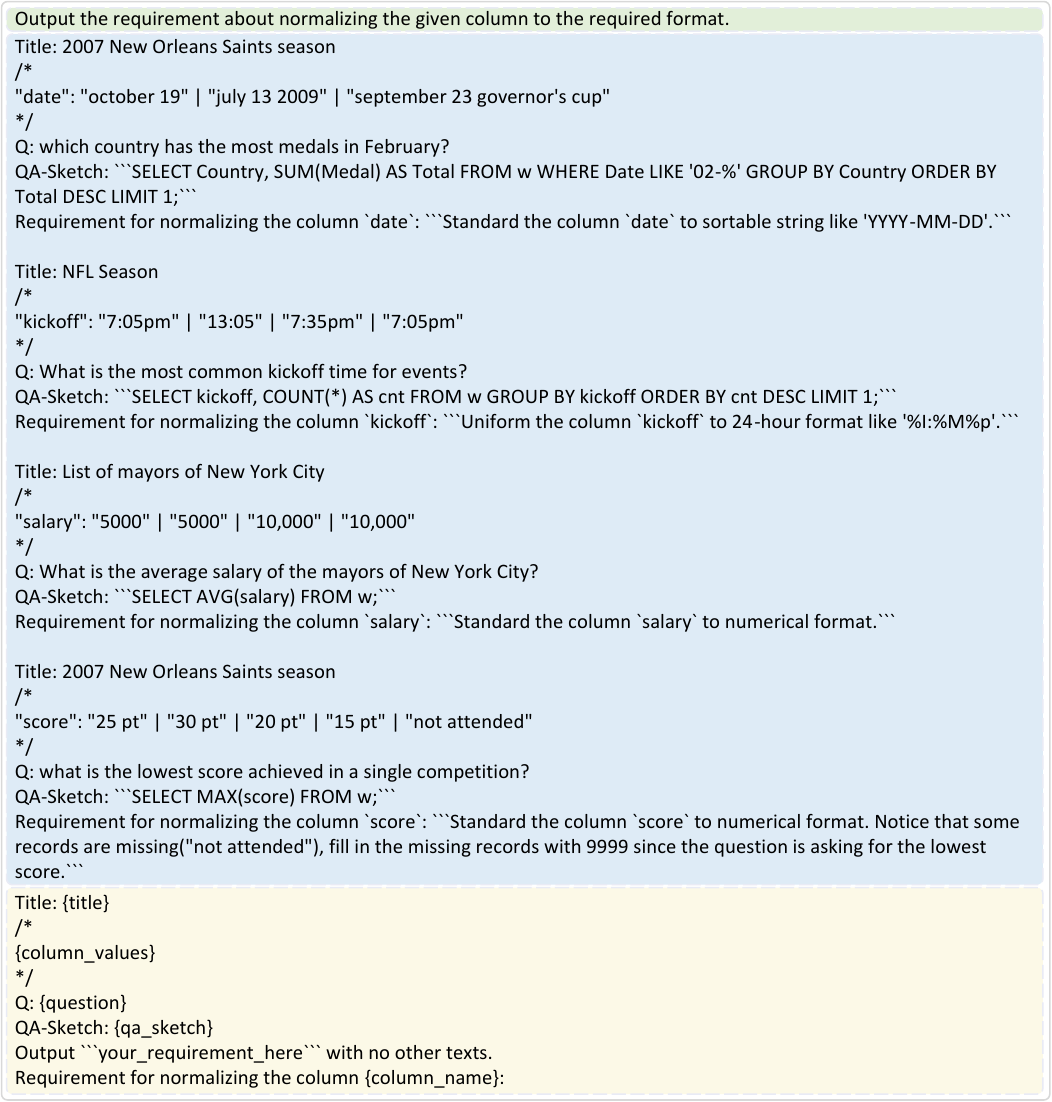}
    \vspace{-1em}
    \caption{Prompt of Planner on generating requirement for Normalize Operator.
    %, such as NL2SQL as shown in the figure. \sys decomposes the data prep process into three stages: \textcircled{1} The Planning stage, \textcircled{2} the Programming stage and \textcircled{3} the Executing stage.
    }
    \label{fig:prompt_planner_generate_req_norm}
    % \vspace{-1em}
\end{figure*}

The \textsc{Planner} aims at generating logical operators in two stages: (1) generate the QA-Sketch. (2) generate specific requirement for Normalize and Derive.

In the first stage, \sys analyzes the table and the question to generate the reasoning process of question answering over table with the assistance of pseudo codes. In this paper, we define the grammar of the pseudo code as SQL with a UDF grammar. The prompts for WikITQ and TabFact datasets are shown in Figure~\ref{fig:prompt_planner_analysis_sketch_wikitq} and Figure~\ref{fig:prompt_planner_analysis_sketch_tabfact}. Next, based on the generated QA-Sketch, we extract each operation clause and provide the related column data in the clause to query LLMs to generate specific requirement of the logical operator. The prompts of generating specific requirement for each type of logical operator are shown in Figure~\ref{fig:prompt_planner_generate_req_aug} and Figure~\ref{fig:prompt_planner_generate_req_norm}. Notice that the Filter operator is generated by analyzing the QA-Sketch and the arguments of Derive operator, which does not need to query LLMs.

\subsection{Prompts in Programmer Agents}

%!TEX root = ../../main.tex
\begin{figure*}[!t]
    \centering 
    \includegraphics[width=0.99\textwidth]{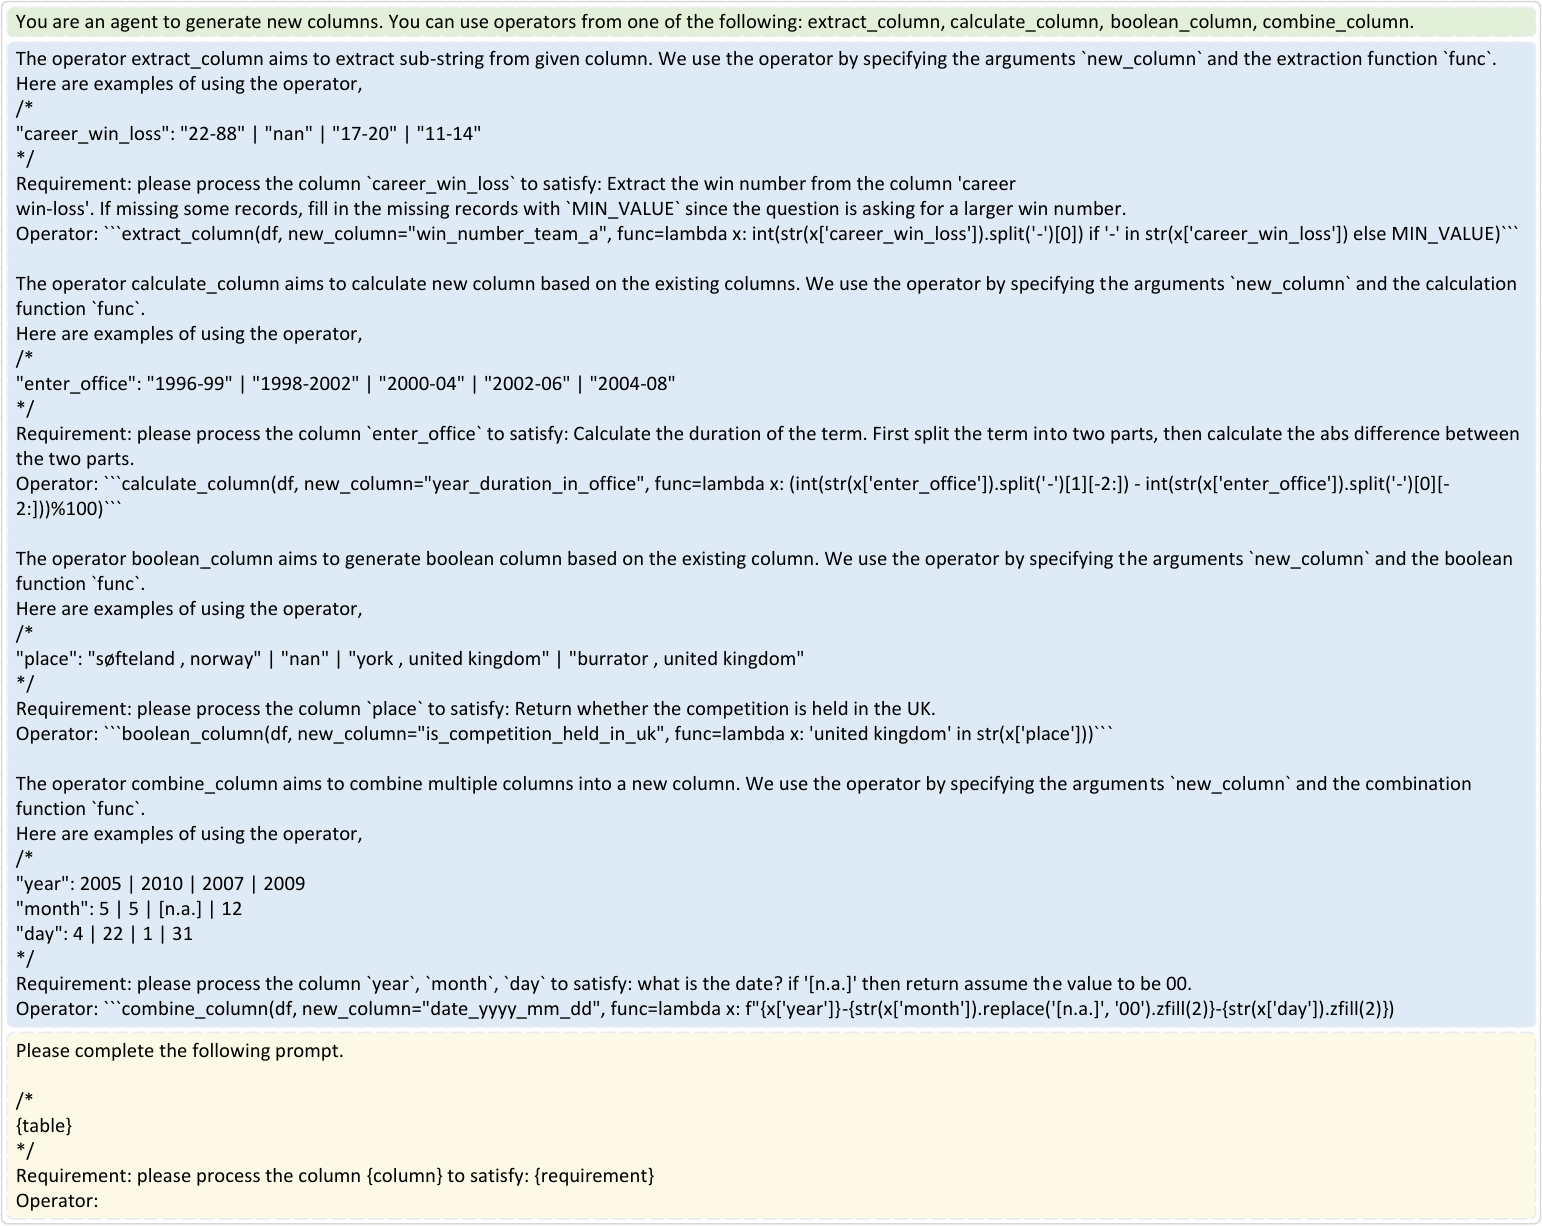}
    \vspace{-1em}
    \caption{Prompt of Derive.
    %, such as NL2SQL as shown in the figure. \sys decomposes the data prep process into three stages: \textcircled{1} The Planning stage, \textcircled{2} the Programming stage and \textcircled{3} the Executing stage.
    }
    \label{fig:prompt_augment}
    % \vspace{-1em}
\end{figure*}
%!TEX root = ../../main.tex
\begin{figure*}[!t]
    \centering 
    \includegraphics[width=0.9\textwidth]{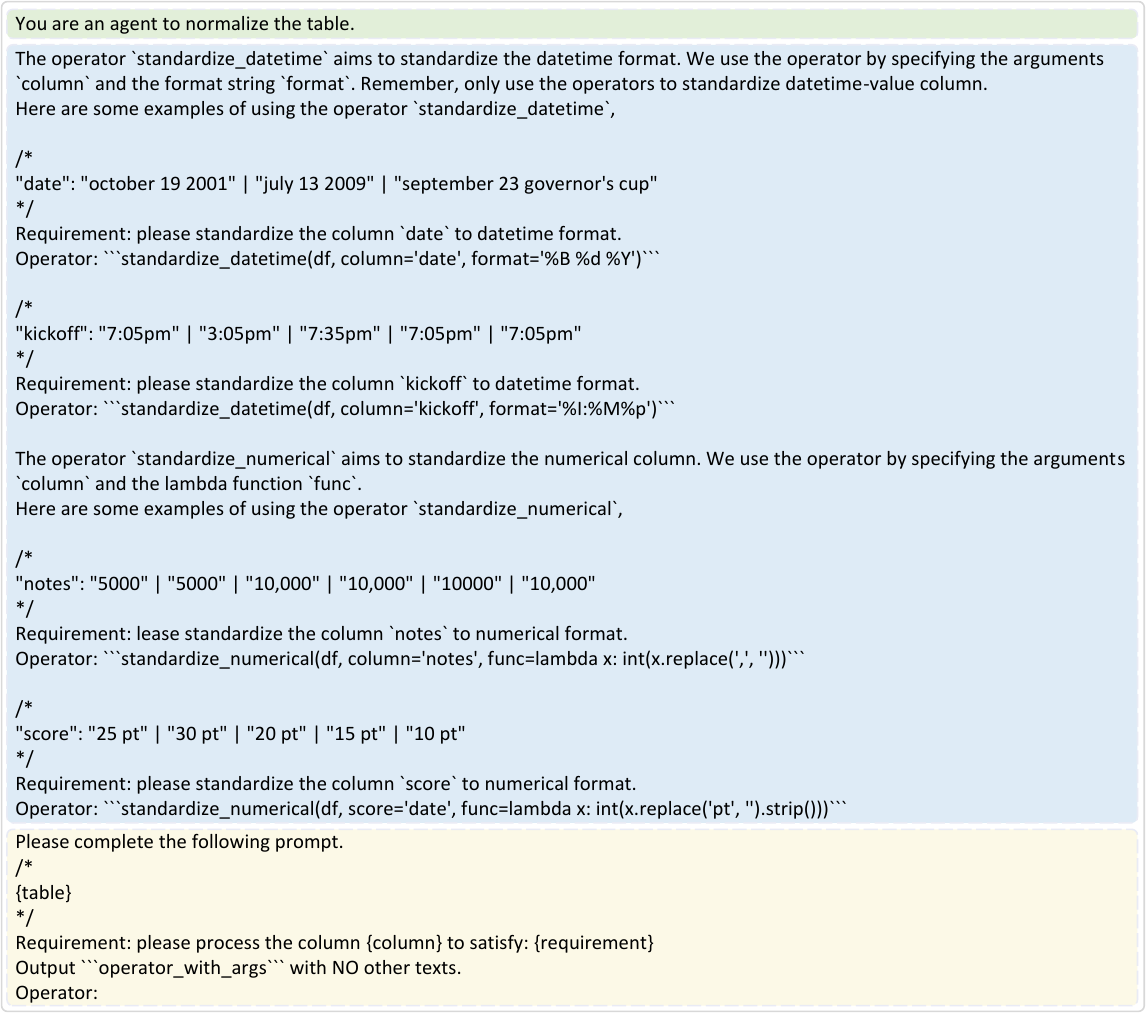}
    \vspace{-1em}
    \caption{Prompt of Normalize.
    %, such as NL2SQL as shown in the figure. \sys decomposes the data prep process into three stages: \textcircled{1} The Planning stage, \textcircled{2} the Programming stage and \textcircled{3} the Executing stage.
    }
    \label{fig:prompt_normalizer}
    % \vspace{-1em}
\end{figure*}
%!TEX root = ../../main.tex
\begin{figure*}[!t]
    \centering 
    \includegraphics[width=0.90\textwidth]{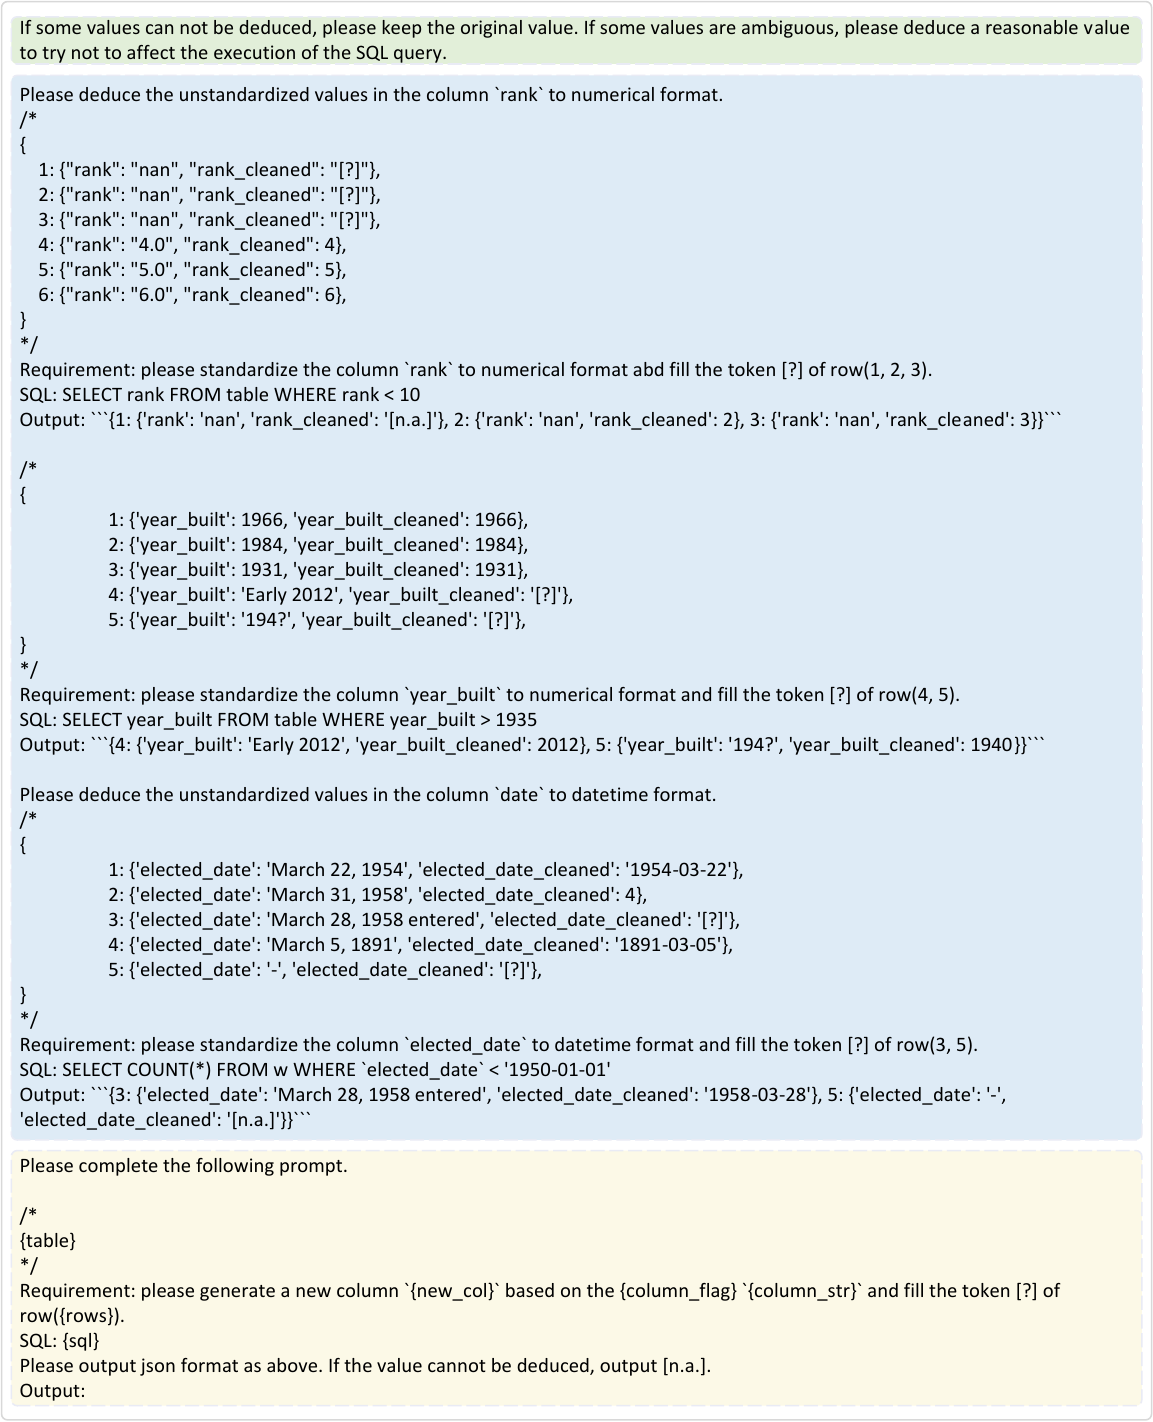}
    \vspace{-1em}
    \caption{Prompt of Imputater.
    %, such as NL2SQL as shown in the figure. \sys decomposes the data prep process into three stages: \textcircled{1} The Planning stage, \textcircled{2} the Programming stage and \textcircled{3} the Executing stage.
    }
    \label{fig:prompt_imputate}
    % \vspace{-1em}
\end{figure*}
%!TEX root = ../../main.tex
\begin{figure*}[!t]
    \centering 
    \includegraphics[width=0.90\textwidth]{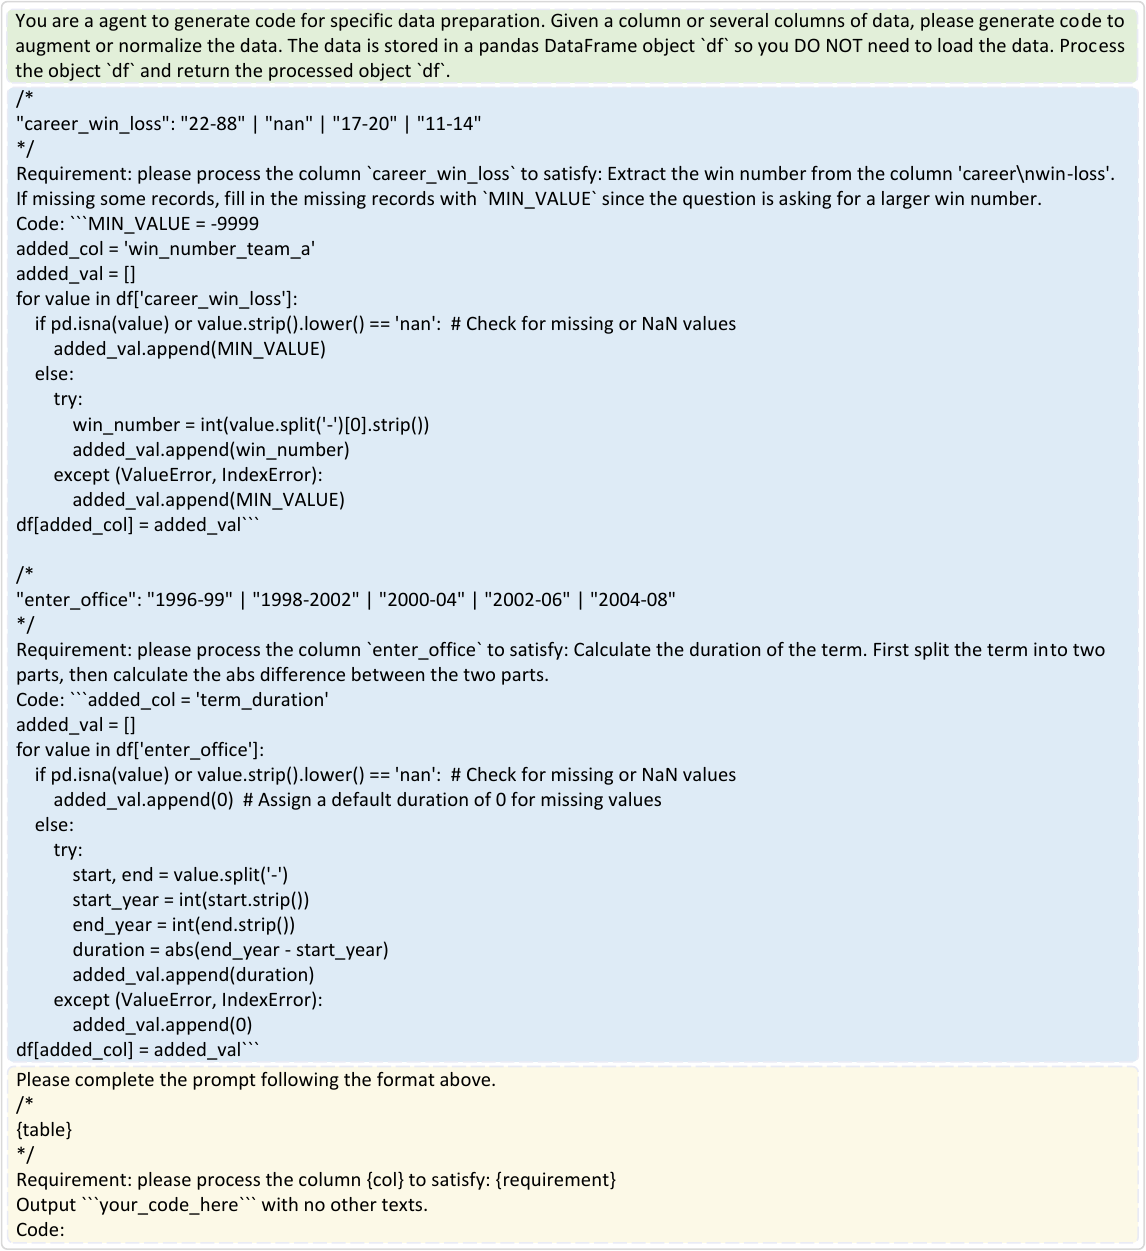}
    \vspace{-1em}
    \caption{Prompt of LLM Coder.
    %, such as NL2SQL as shown in the figure. \sys decomposes the data prep process into three stages: \textcircled{1} The Planning stage, \textcircled{2} the Programming stage and \textcircled{3} the Executing stage.
    }
    \label{fig:prompt_llm_code}
    % \vspace{-1em}
\end{figure*}

Given logical operators with specific requirement and related columns, the programmer agents generate physical operators to implement the logical operators. The prompts of \textsc{Derive} and \textsc{Normalize} are shown in Figure~\ref{fig:prompt_augment} and Figure~\ref{fig:prompt_normalizer}. In addition, if any logical operators can not be implemented with functions in the function pool, we call LLMs to generate Python codes. The prompt of generating Python code is shown in Figure~\ref{fig:prompt_llm_code}. Finally, if any values can not be derived or normalized, we call an Imputater agent to direct infer the correct values. The prompt is shown in Figure~\ref{fig:prompt_imputate}.

\subsection{Prompts in other baselines}

%!TEX root = ../../main.tex
\begin{figure*}[!t]
    \centering 
    \includegraphics[width=0.95\textwidth]{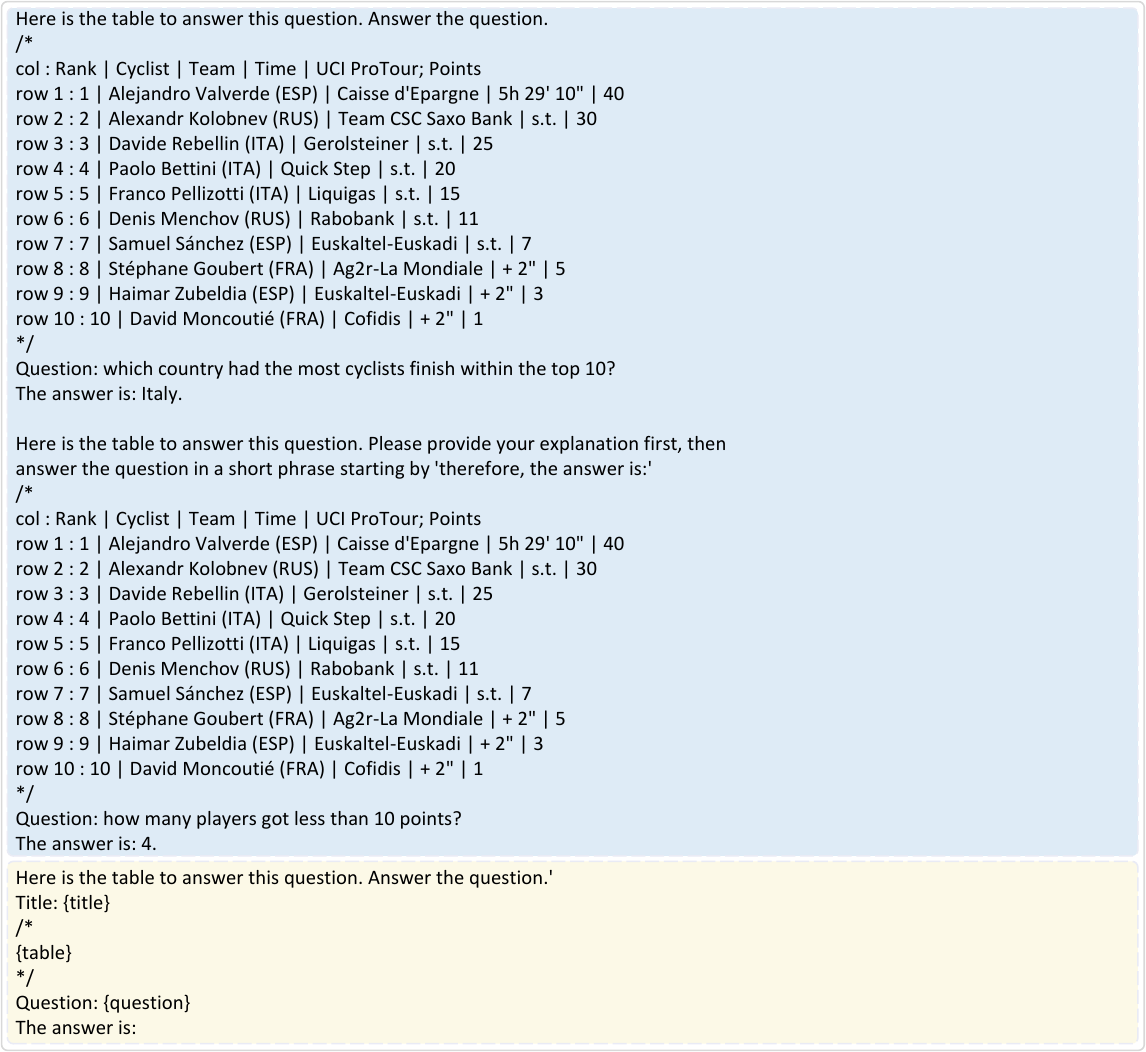}
    \vspace{-1em}
    \caption{Prompt of End2End method on WikiTQ dataset.
    %, such as NL2SQL as shown in the figure. \sys decomposes the data prep process into three stages: \textcircled{1} The Planning stage, \textcircled{2} the Programming stage and \textcircled{3} the Executing stage.
    }
    \label{fig:prompt_end2end_wikitq}
    % \vspace{-1em}
\end{figure*}
%!TEX root = ../../main.tex
\begin{figure*}[!t]
    \centering 
    \includegraphics[width=0.70\textwidth]{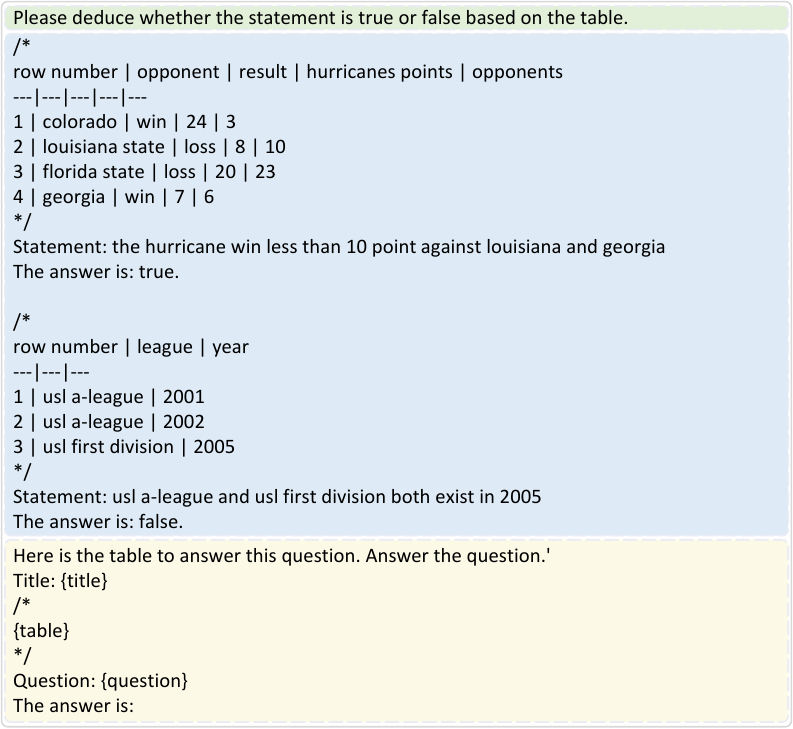}
    \vspace{-1em}
    \caption{Prompt of End2End method on TabFact dataset.
    %, such as NL2SQL as shown in the figure. \sys decomposes the data prep process into three stages: \textcircled{1} The Planning stage, \textcircled{2} the Programming stage and \textcircled{3} the Executing stage.
    }
    \label{fig:prompt_end2end_tabfact}
    % \vspace{-1em}
\end{figure*}

%!TEX root = ../../main.tex
\begin{figure*}[!t]
    \centering 
    \includegraphics[width=0.99\textwidth]{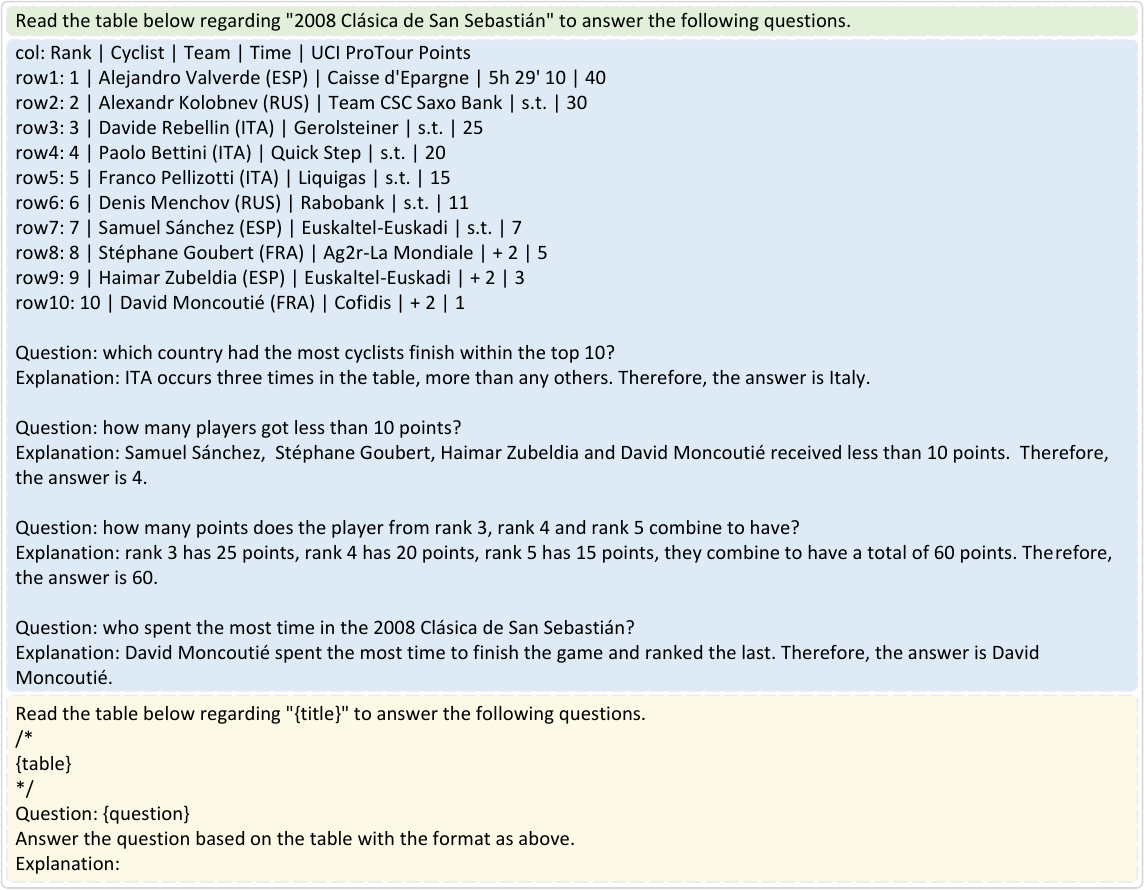}
    \vspace{-1em}
    \caption{Prompt of Chain-of-Thought TQA method on WikiTQ dataset.
    %, such as NL2SQL as shown in the figure. \sys decomposes the data prep process into three stages: \textcircled{1} The Planning stage, \textcircled{2} the Programming stage and \textcircled{3} the Executing stage.
    }
    \label{fig:prompt_cot_wikitq}
    % \vspace{-1em}
\end{figure*}
%!TEX root = ../../main.tex
\begin{figure*}[!t]
    \centering 
    \includegraphics[width=0.85\textwidth]{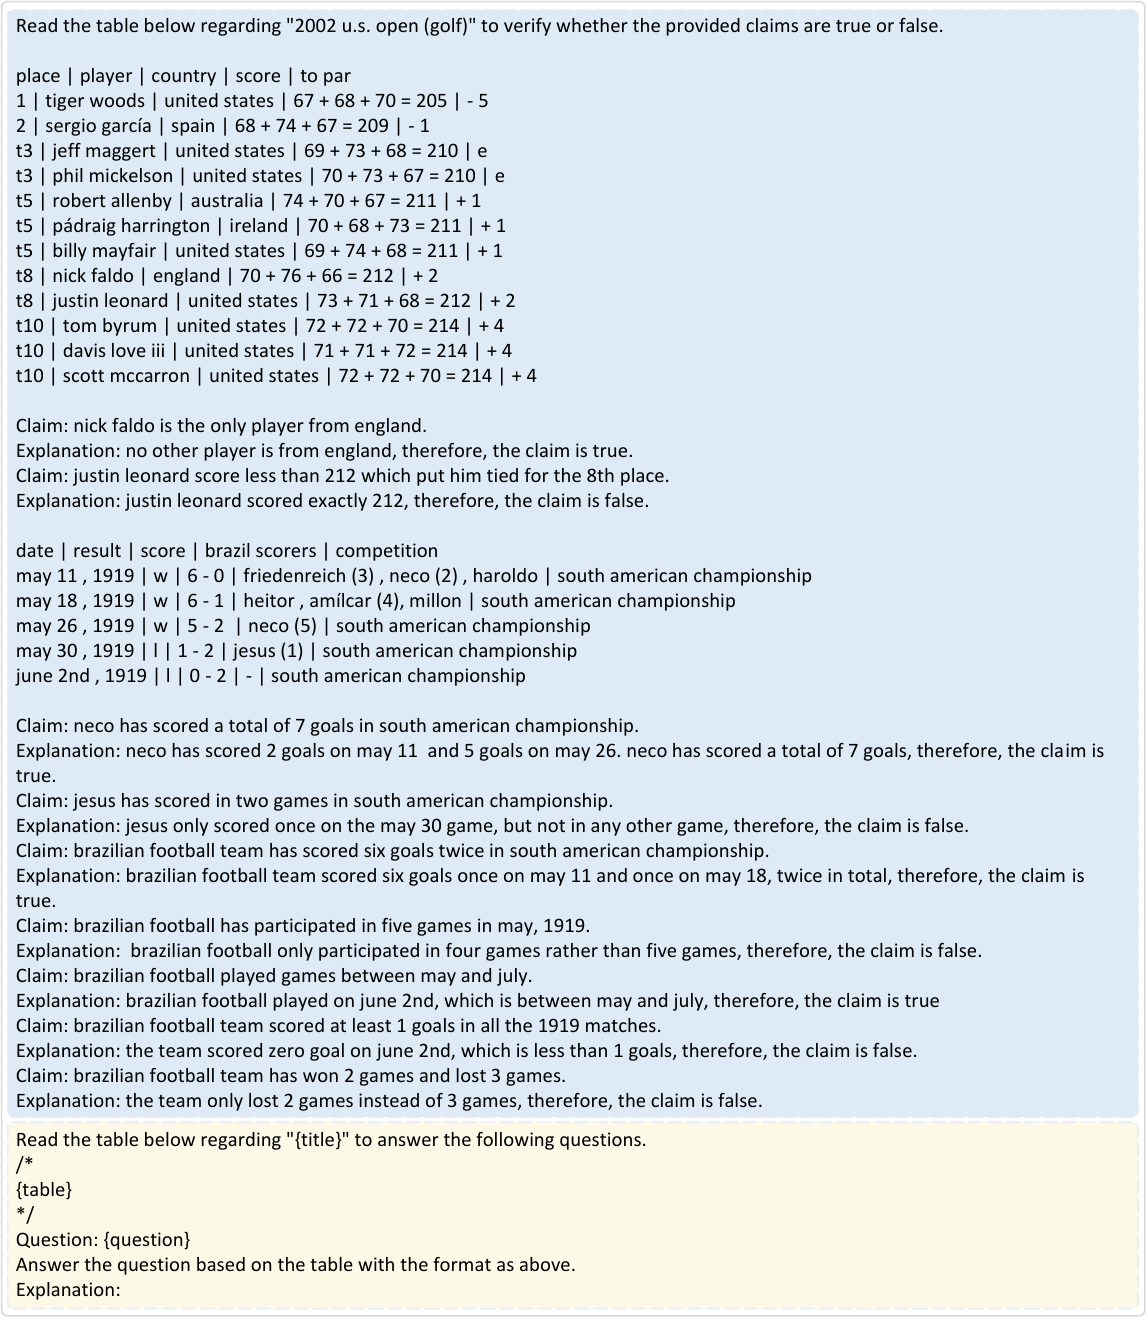}
    \vspace{-1em}
    \caption{Prompt of Chain-of-Thought TQA method on TabFact dataset.
    %, such as NL2SQL as shown in the figure. \sys decomposes the data prep process into three stages: \textcircled{1} The Planning stage, \textcircled{2} the Programming stage and \textcircled{3} the Executing stage.
    }
    \label{fig:prompt_cot_tabfact}
    % \vspace{-1em}
\end{figure*}

%!TEX root = ../../main.tex
\begin{figure*}[!t]
    \centering 
    \includegraphics[width=0.85\textwidth]{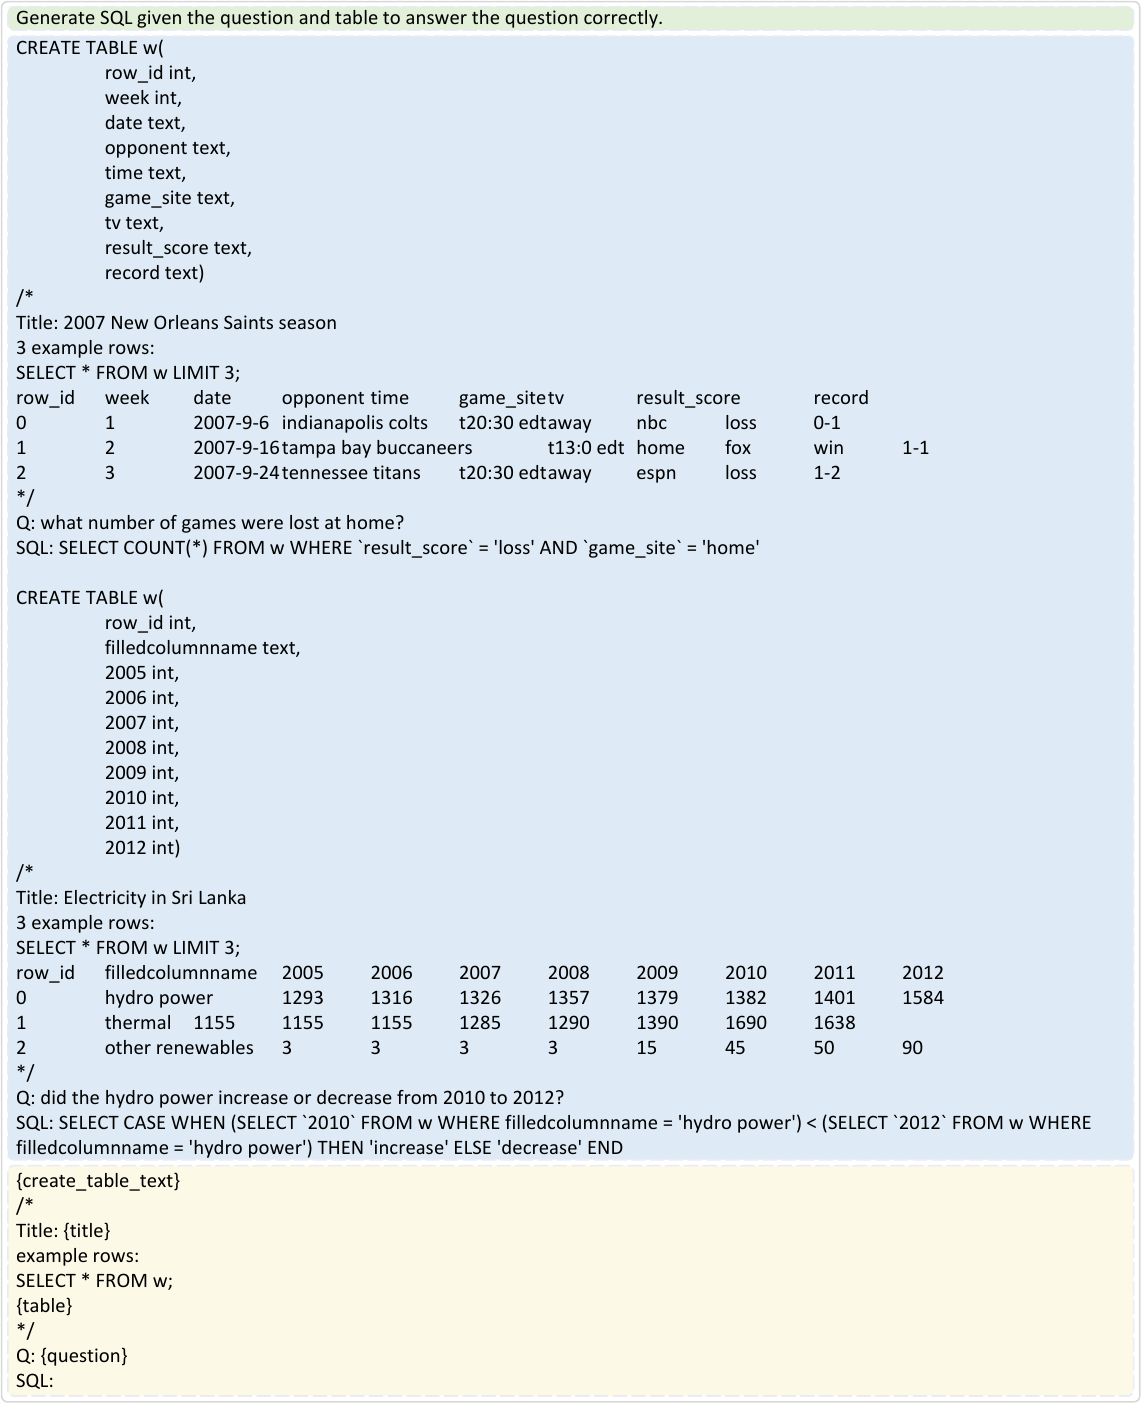}
    \vspace{-1em}
    \caption{Prompt of NL2SQL on WikiTQ dataset.
    %, such as NL2SQL as shown in the figure. \sys decomposes the data prep process into three stages: \textcircled{1} The Planning stage, \textcircled{2} the Programming stage and \textcircled{3} the Executing stage.
    }
    \label{fig:prompt_nl2sql_wikitq}
    % \vspace{-1em}
\end{figure*}
%!TEX root = ../../main.tex
\begin{figure*}[!t]
    \centering 
    \includegraphics[width=0.99\textwidth]{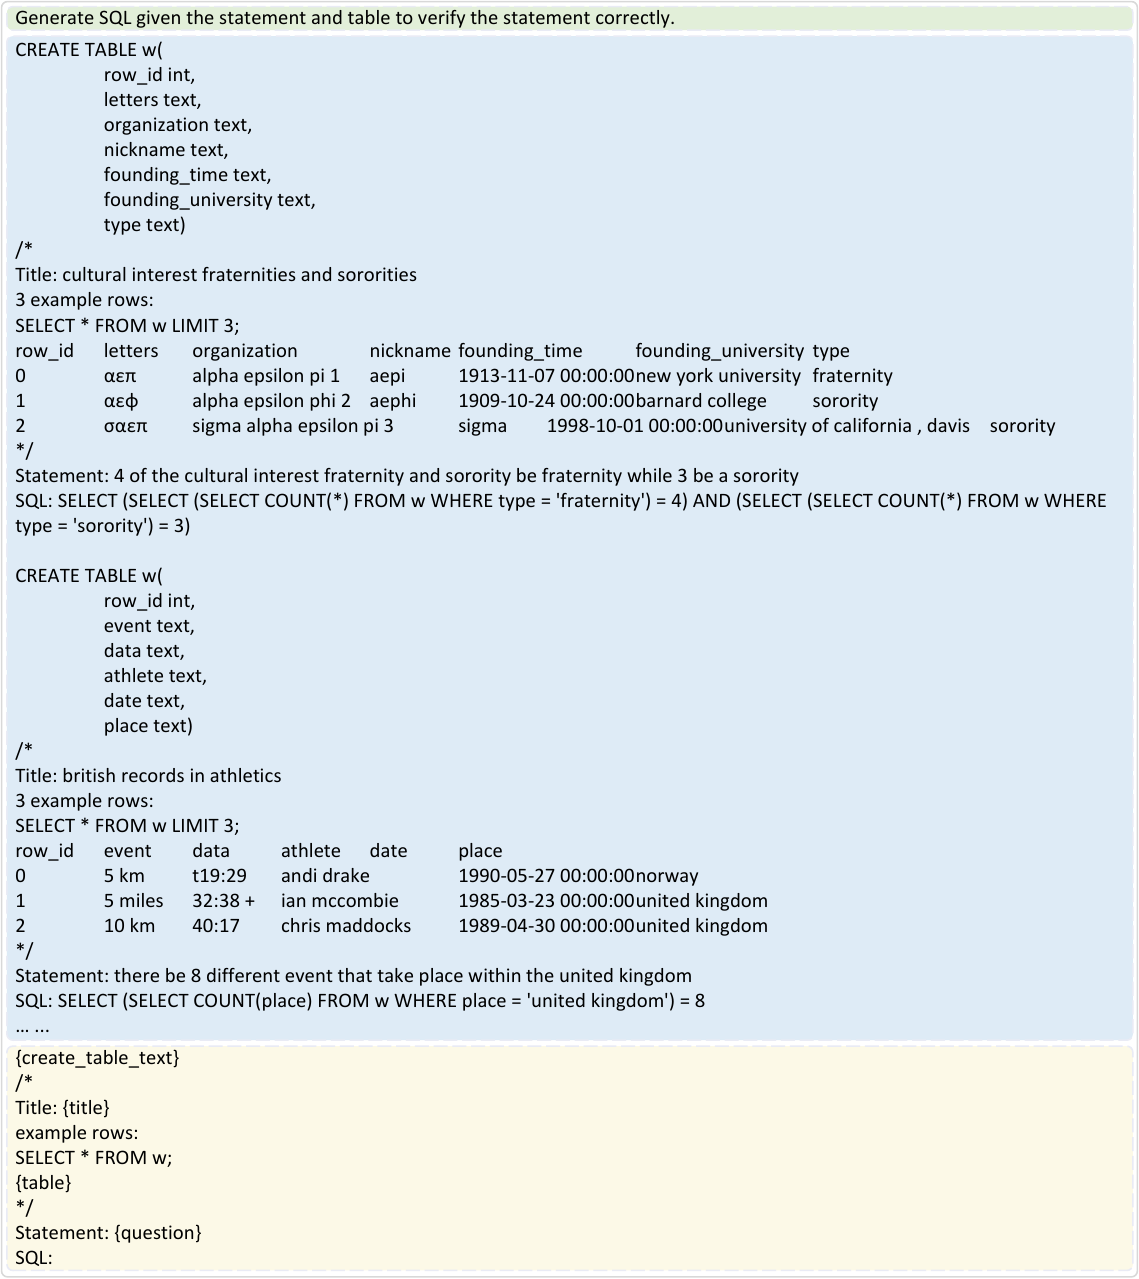}
    \vspace{-1em}
    \caption{Prompt of NL2SQL on TabFact dataset.
    %, such as NL2SQL as shown in the figure. \sys decomposes the data prep process into three stages: \textcircled{1} The Planning stage, \textcircled{2} the Programming stage and \textcircled{3} the Executing stage.
    }
    \label{fig:prompt_nl2sql_tabfact}
    % \vspace{-1em}
\end{figure*}

%!TEX root = ../../main.tex
\begin{figure*}[!t]
    \centering 
    \includegraphics[width=0.99\textwidth]{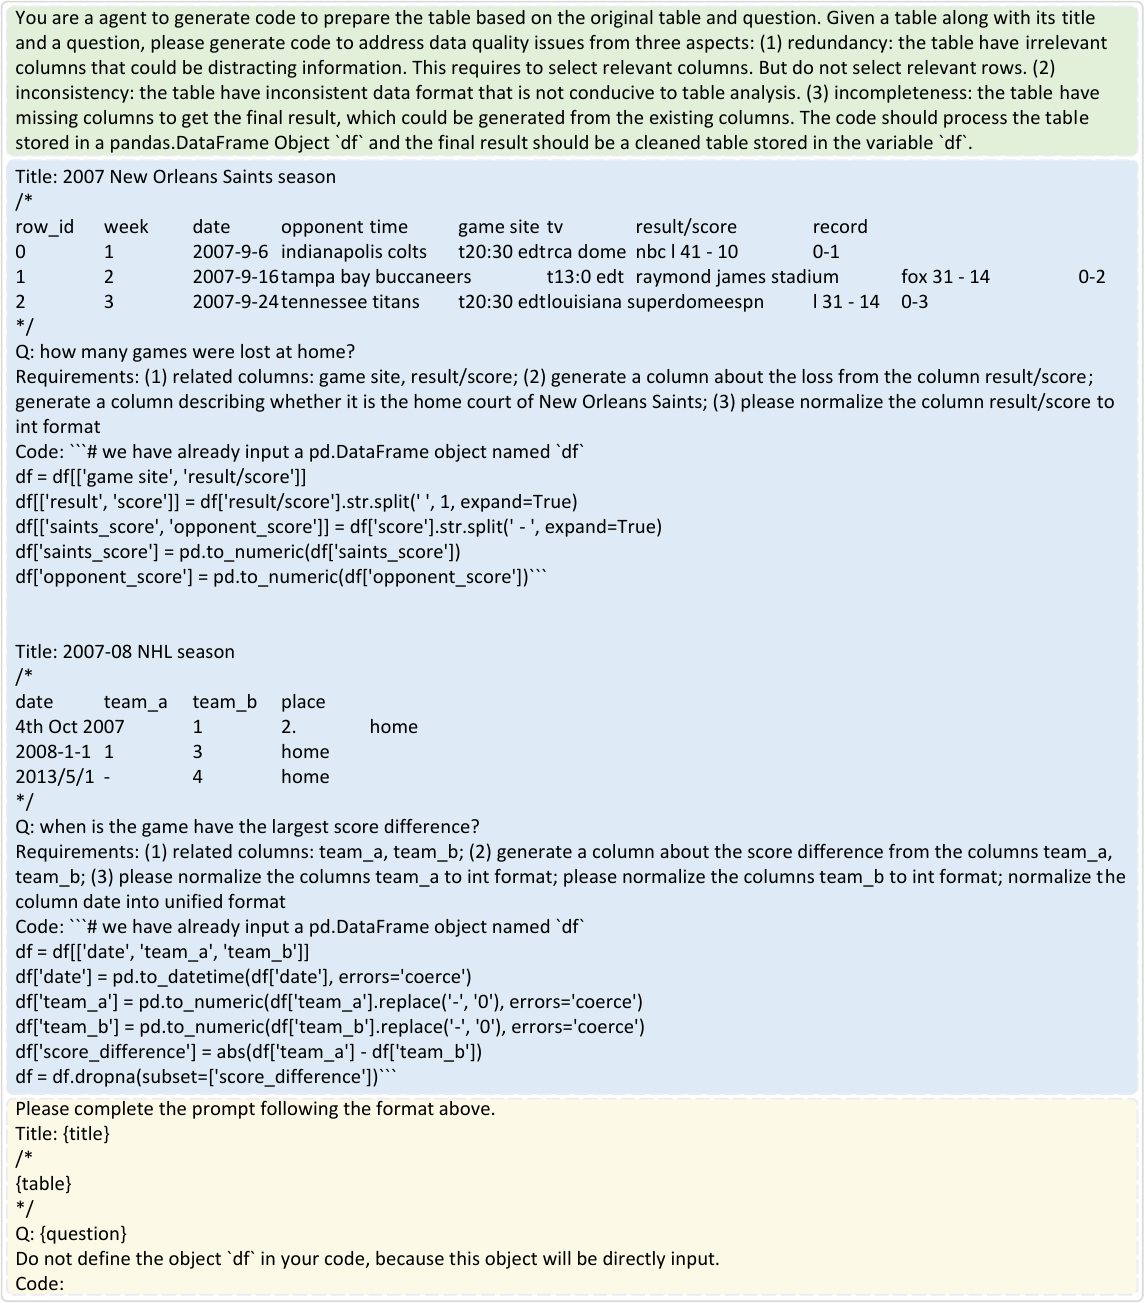}
    \vspace{-1em}
    \caption{Prompt of ICL-Prep on WikiTQ dataset.
    %, such as NL2SQL as shown in the figure. \sys decomposes the data prep process into three stages: \textcircled{1} The Planning stage, \textcircled{2} the Programming stage and \textcircled{3} the Executing stage.
    }
    \label{fig:prompt_iclprep_wikitq}
    % \vspace{-1em}
\end{figure*}
%!TEX root = ../../main.tex
\begin{figure*}[!t]
    \centering 
    \includegraphics[width=0.99\textwidth]{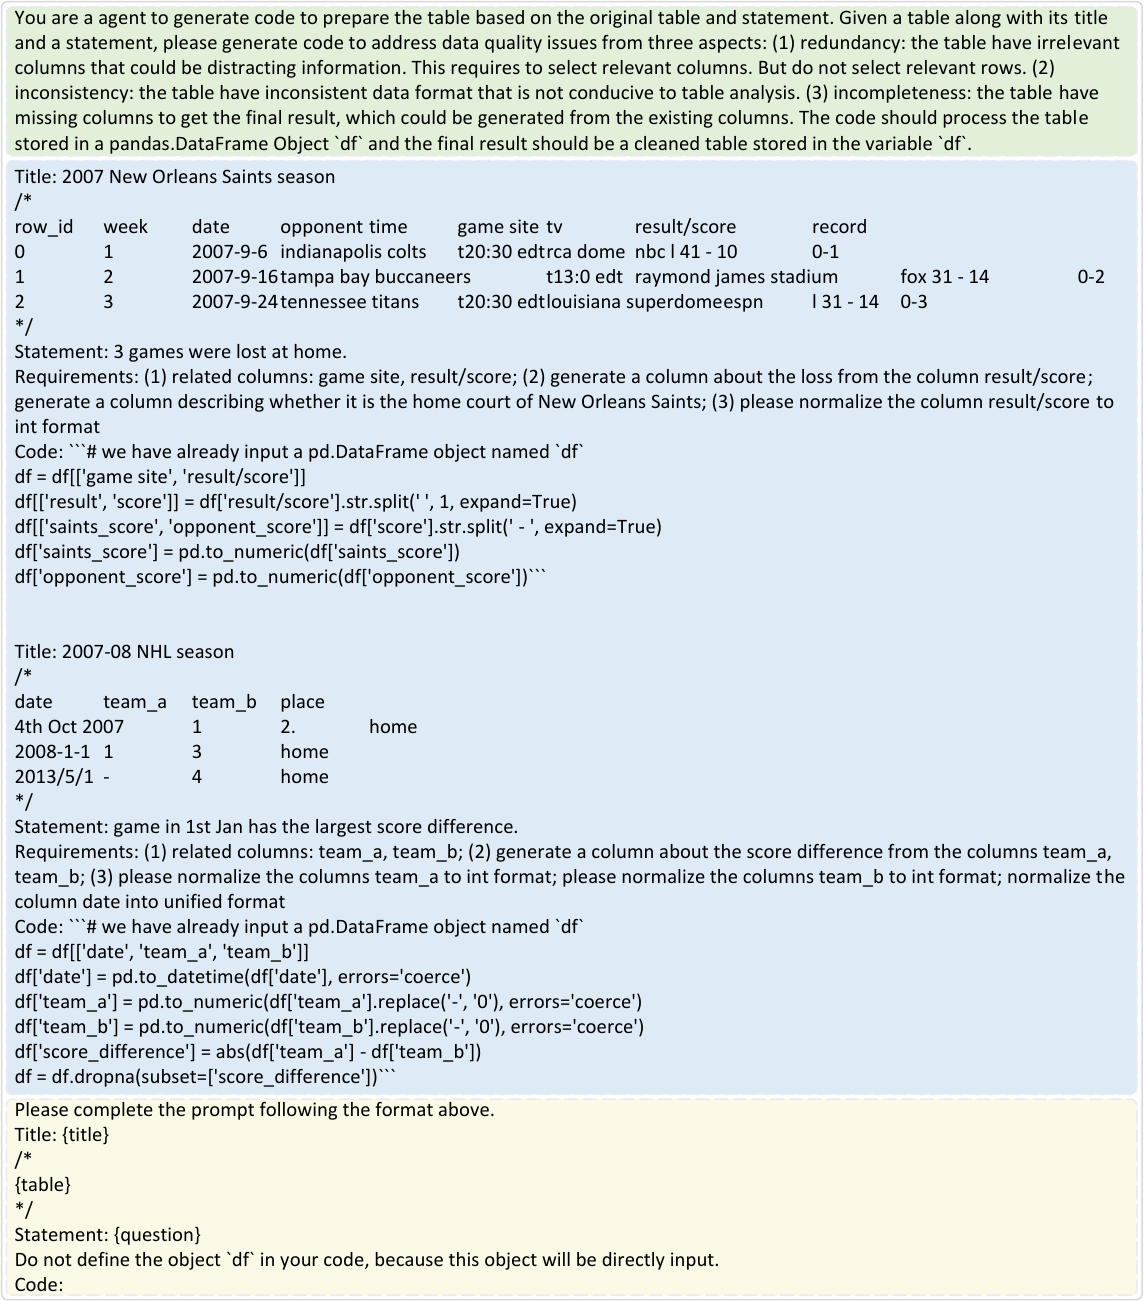}
    \vspace{-1em}
    \caption{Prompt of ICL-Prep on TabFact dataset.
    %, such as NL2SQL as shown in the figure. \sys decomposes the data prep process into three stages: \textcircled{1} The Planning stage, \textcircled{2} the Programming stage and \textcircled{3} the Executing stage.
    }
    \label{fig:prompt_iclprep_tabfact}
    % \vspace{-1em}
\end{figure*}

%!TEX root = ../../main.tex
\begin{figure*}[!t]
    \centering 
    \includegraphics[width=0.99\textwidth]{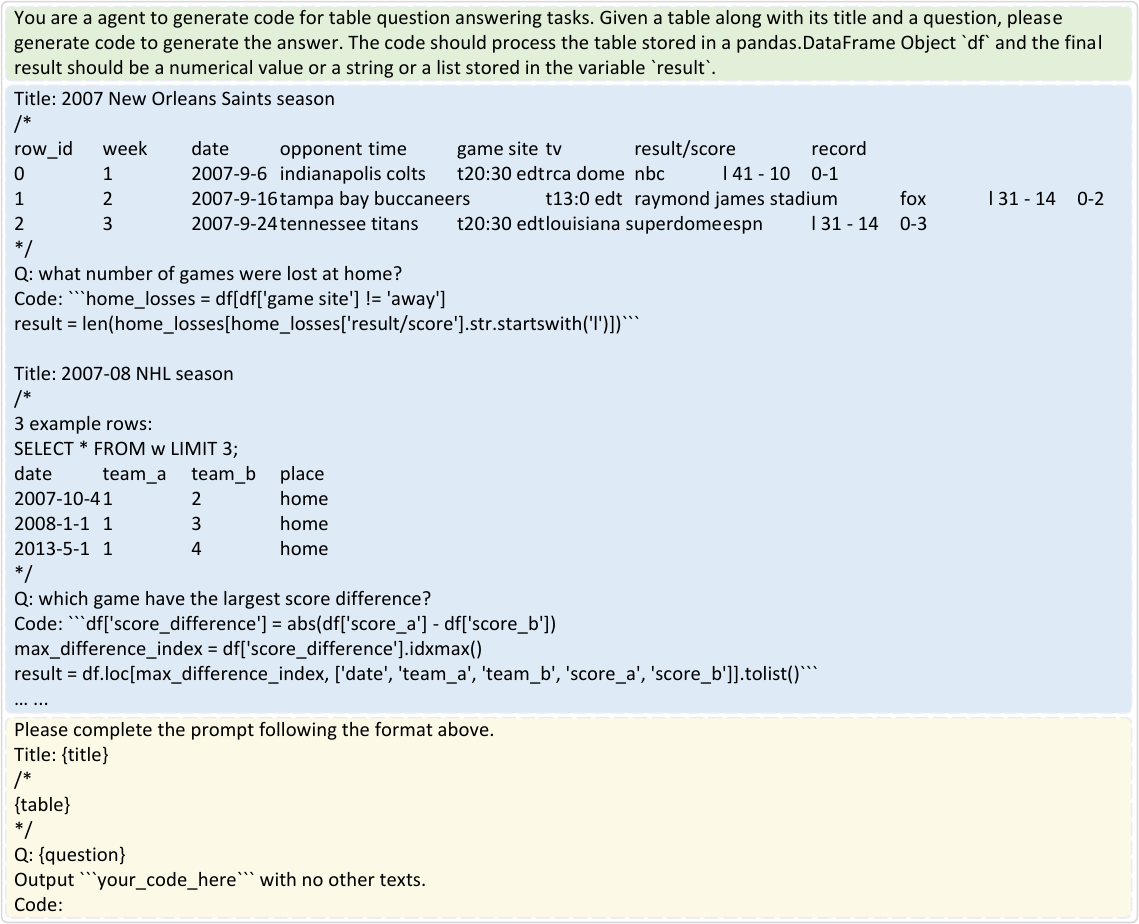}
    \vspace{-1em}
    \caption{Prompt of NL2Py on WikiTQ dataset.
    %, such as NL2SQL as shown in the figure. \sys decomposes the data prep process into three stages: \textcircled{1} The Planning stage, \textcircled{2} the Programming stage and \textcircled{3} the Executing stage.
    }
    \label{fig:prompt_nl2py_wikitq}
    % \vspace{-1em}
\end{figure*}
%!TEX root = ../../main.tex
\begin{figure*}[!t]
    \centering 
    \includegraphics[width=0.99\textwidth]{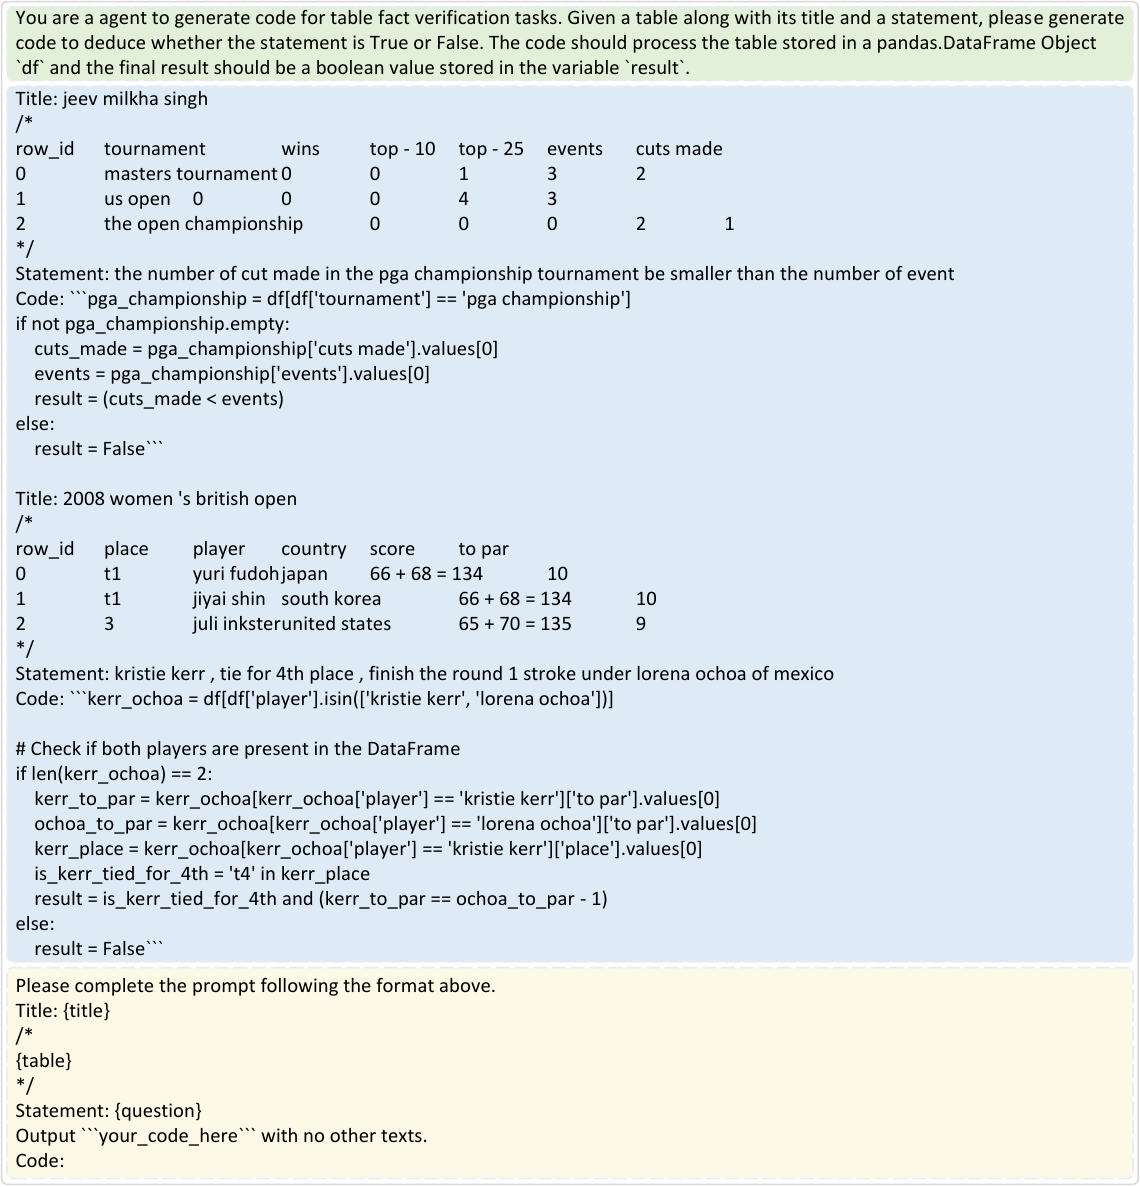}
    \vspace{-1em}
    \caption{Prompt of NL2Py on TabFact dataset.
    %, such as NL2SQL as shown in the figure. \sys decomposes the data prep process into three stages: \textcircled{1} The Planning stage, \textcircled{2} the Programming stage and \textcircled{3} the Executing stage.
    }
    \label{fig:prompt_nl2py_tabfact}
    % \vspace{-1em}
\end{figure*}

We also provide the prompts of implemented baselines, including
End2End (Figure~\ref{fig:prompt_end2end_wikitq} and Figure~\ref{fig:prompt_end2end_tabfact}),
CoT (Figure~\ref{fig:prompt_cot_wikitq} and Figure~\ref{fig:prompt_cot_tabfact}),
NL2SQL (Figure~\ref{fig:prompt_nl2sql_wikitq} and Figure~\ref{fig:prompt_nl2sql_tabfact}), NL2Py (Figure~\ref{fig:prompt_nl2py_wikitq} and Figure~\ref{fig:prompt_nl2py_tabfact})
and ICL-Prep (Figure~\ref{fig:prompt_iclprep_wikitq} and Figure~\ref{fig:prompt_iclprep_tabfact}). Some of the prompts are from existing works~\cite{cheng2023binding,chen2022large} as described in the experimental setup.
