# Supplementary material for: AutoPrep: Natural Language Question-Aware Data Preparation with a Multi-Agent Framework
Source: arXiv:2412.10422 source file (2025-07-09)
Supplement: Supplementary file 2 [file a_running_example_of_autoprep.tex]

\section{A Running Example of AUTOPREP}
\label{sec:appendix_a_running_example_of_autoprep}

\begin{figure*}[t]
    % \vspace{-1em}
    \centering
    \begin{subfigure}{0.48\textwidth}
        \includegraphics[width=\textwidth]{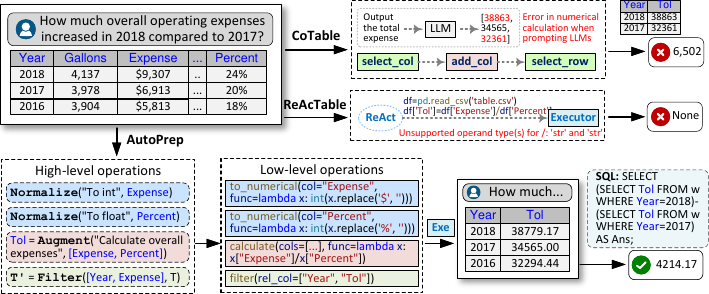}
        % \captionsetup{skip=0.5pt}
        \caption{Case one}
        \label{fig:case_study1}
    \end{subfigure}
    \hspace{-1mm}
    \quad \quad
    \begin{subfigure}{0.48\textwidth}
        \includegraphics[width=\textwidth]{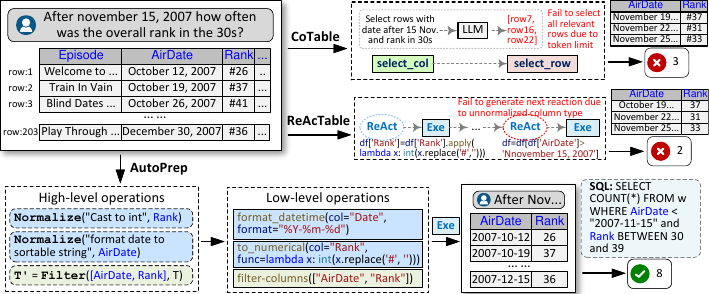}
        % \captionsetup{skip=0.5pt}
        \caption{Case two}
        \label{fig:case_study2}
    \end{subfigure}
    \vspace{-2.5em}
    \caption{{Two case studies selected from TabBench and WikiTQ to qualitatively analyze effectiveness of \sys.}}
    \label{fig:case_study}
    \vspace{-1em}
\end{figure*}

%Based on the experimental results, \sys outperforms the two most powerful TQA methods ReAcTable and CoTable. 

This section presents two illustrative examples from TabBench and WikiTQ to qualitatively analyze effectiveness of \sys. 

To answer the question in Figure~\ref{fig:case_study1}, CoTable generates an operator chain with an ``add\_col'' operator, which is used to generate a new column \term{Tol} based on the division results of two existing columns \term{Expense} and \term{Percent}. This operator directly prompts an LLM to output a list containing all values of the new column, which is a challenging task for previous LLMs. Thus, CoTable generates a new column with two wrong values which leads to a wrong answer. For ReAcTable, although it generates a logically correct Python program, it ignores the types of existing columns which do not support for numerical calculation. Thus, ReAcTable also fails to derive the \term{Tol} column.
\sys addresses this issue by first utilizing a \textsc{Planner} agent to generate logical operators specifying data prep requirements, i.e., two $\mathtt{Normalize}$ to normalize column \term{Expense} and \term{Percent}, a $\mathtt{Derive}$ to generate the overall expenses \term{Tol} and a $\mathtt{Filter}$ to select related columns \term{Year} and \term{Tol}. 
These logical operators are passed to \textsc{Programmer} agents to generate physical operators consisting of a pre-defined Python function. For example, we call $\mathtt{to\mbox{-}numerical}$ function two times to cast \term{Expense} and \term{Percent} to numerical values.
All physical operators are executed to process the original table and output a prepared table. Finally, an \textsc{Analyzer} agent based on NL2SQL method generates a SQL query to extract the correct answer ``4214.17''.

Figure~\ref{fig:case_study2} illustrates a TQA instance involving large tables and inconsistent values. 
%To answer the question, CoTable selects all relevant rows for the question. However, it loses related information due to the maximum input token limitation. Specifically, the table is cropped to include only the first 100 rows to fit within the prompt. Thus, all data in the last 103 rows is lost. Consequently, it generates a sub-table table with incomplete data, resulting in an incorrect answer ``3''. For ReAcTable, it reacts in multiple steps to process the table. When filtering records with \term{Date} after ``november 15, 2007'', it does not transform the \term{Date} into comparable format before using operator ``$>$'' to filter the records. Thus, ReAcTable also generates an error answer.
\sys solves this by splitting the TQA question into two phases, i.e., data prep and data analysis. It first generates logical operators including two $\mathtt{Normalize}$ and one $\mathtt{Filter}$. Next, the \textsc{Programmer} agents implement them with corresponding physical operators, which are executed to produce a prepared table. Based on this, the \textsc{Analyzer} agent extracts the final answer ``8''.
