# Supplementary material for: AutoPrep: Natural Language Question-Aware Data Preparation with a Multi-Agent Framework
Source: arXiv:2412.10422 source file (2025-07-09)
Supplement: Supplementary file 3 [file details_of_the_error_analysis.tex]

%!TEX root = ../../main.tex
\begin{figure}[!t]
    \centering 
    \includegraphics[width=0.99\columnwidth]{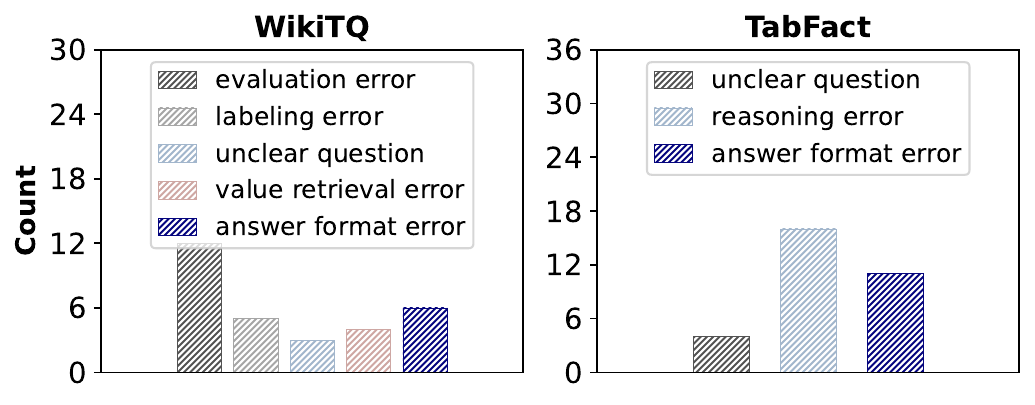}
    \vspace{-1em}
    \caption{{In-depth Analysis of the ``\term{Other}'' Category.}
    %, such as NL2SQL as shown in the figure. \sys decomposes the data prep process into three stages: \textcircled{1} The Planning stage, \textcircled{2} the Programming stage and \textcircled{3} the Executing stage.
    }
    \label{fig:subcategories_in_other}
    % \vspace{-1em}
\end{figure}

\section{Details of the Error Analysis}
\label{sec:appendix_details_of_error_analysis}

This section presents details of the error analysis shown in Figure~\ref{fig:error_instance_record}, which motivates us to study question-aware data prep.

\stitle{TQA Method: NL2SQL Based on GPT-4.}
We adopt NL2SQL~\cite{rajkumar2022evaluating}, a representative TQA baseline that does not perform data prep, as introduced in Section~\ref{subsec:exp-setup}. Specifically, given a natural language question $Q$ and a table $T$, we prompt GPT-4 to generate an SQL query $\term{SQL}$ using a few-shot in-context learning strategy. The query is then executed on $T$ to obtain the final answer $Ans$ for $Q$.

\stitle{Error Categorization.}
We recruite three graduate students from our university's database group to annotate error categories for a randomly sampled set of 500 instances from WikiTQ and TabFact. All annotators have a good understanding of the TQA task and are proficient in SQL syntax.
We instruct the annotators to first identify errors stemming from insufficient data prep, assigning any remaining errors to a default category labeled \term{Other}. For the data prep-related errors, after careful investigation, we further categorize them into the following three types:
(1) \textbf{Missing Semantics:} The table lacks necessary semantic information required to accurately answer the NL question. 
(2) \textbf{Inconsistent Values:} Values within a column are represented inconsistently across different records. 
(3) \textbf{Irrelevant Columns:} The table includes many columns, but only a small subset are actually relevant to the NL question. 

\stitle{In-depth Analysis of the ``\term{Other}'' Category}. 
We report the detailed sub-categories within the ``\term{Other}'' category in Figure~\ref{fig:subcategories_in_other}. As shown, for WikiTQ, more than half of the cases stem from issues inherent to the dataset itself. Notably, 40\% of the errors are due to limitations in the evaluation function, where semantically equivalent but non-identical responses are marked as incorrect, a problem also highlighted in~\cite{cheng2023binding}. Additionally, 20\% of the errors arise from formatting issues in the model’s responses, where the generated SQL logic is correct but the output includes extraneous values from irrelevant columns.
On the other hand, for the TabFact dataset, most errors are attributed to model reasoning failures. Over 50\% result from the model’s inability to generate logically complete and accurate SQL queries. Furthermore, more than 35\% of the errors are due to response formatting issues, where the model returns ambiguous values instead of definitive true/false answers.
