# Supplementary material for: AutoPrep: Natural Language Question-Aware Data Preparation with a Multi-Agent Framework
Source: arXiv:2412.10422 source file (2025-07-09)
Supplement: Supplementary file 5 [file prompt_cot_tabfact.tex]

%!TEX root = ../../main.tex
\begin{figure*}[!t]
    \centering 
    \includegraphics[width=0.85\textwidth]{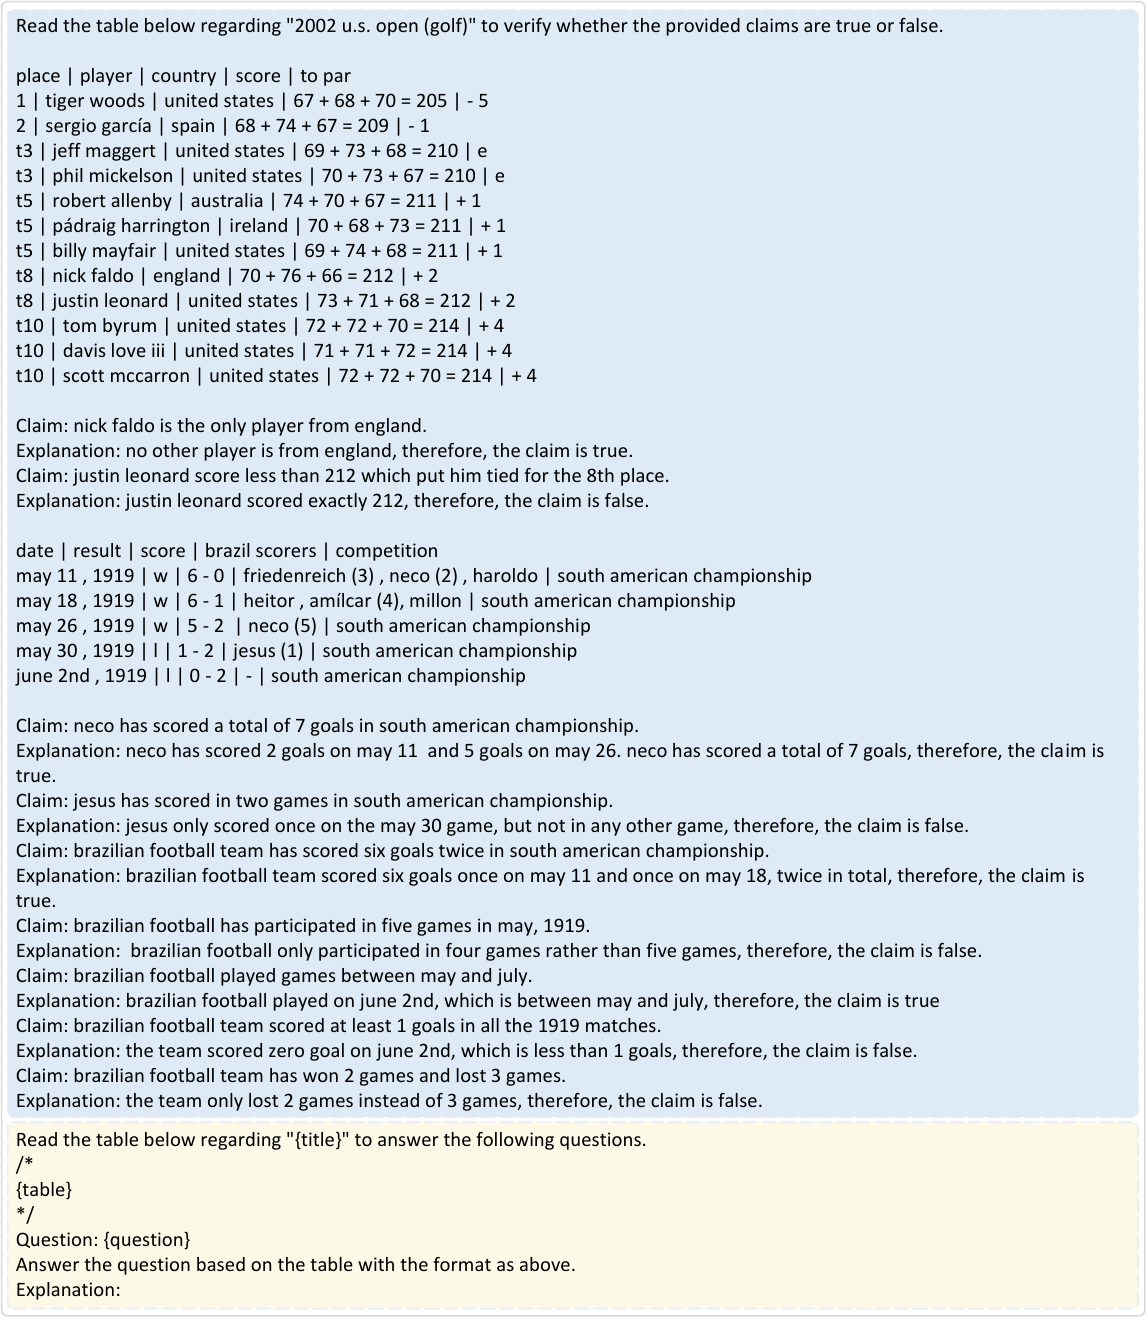}
    \vspace{-1em}
    \caption{Prompt of Chain-of-Thought TQA method on TabFact dataset.
    %, such as NL2SQL as shown in the figure. \sys decomposes the data prep process into three stages: \textcircled{1} The Planning stage, \textcircled{2} the Programming stage and \textcircled{3} the Executing stage.
    }
    \label{fig:prompt_cot_tabfact}
    % \vspace{-1em}
\end{figure*}
