# Supplementary material for: AutoPrep: Natural Language Question-Aware Data Preparation with a Multi-Agent Framework
Source: arXiv:2412.10422 source file (2025-07-09)
Supplement: Supplementary file 20 [file prompt_planner_generate_req_aug.tex]

%!TEX root = ../../main.tex
\begin{figure*}[!t]
    \centering 
    \includegraphics[width=0.9\textwidth]{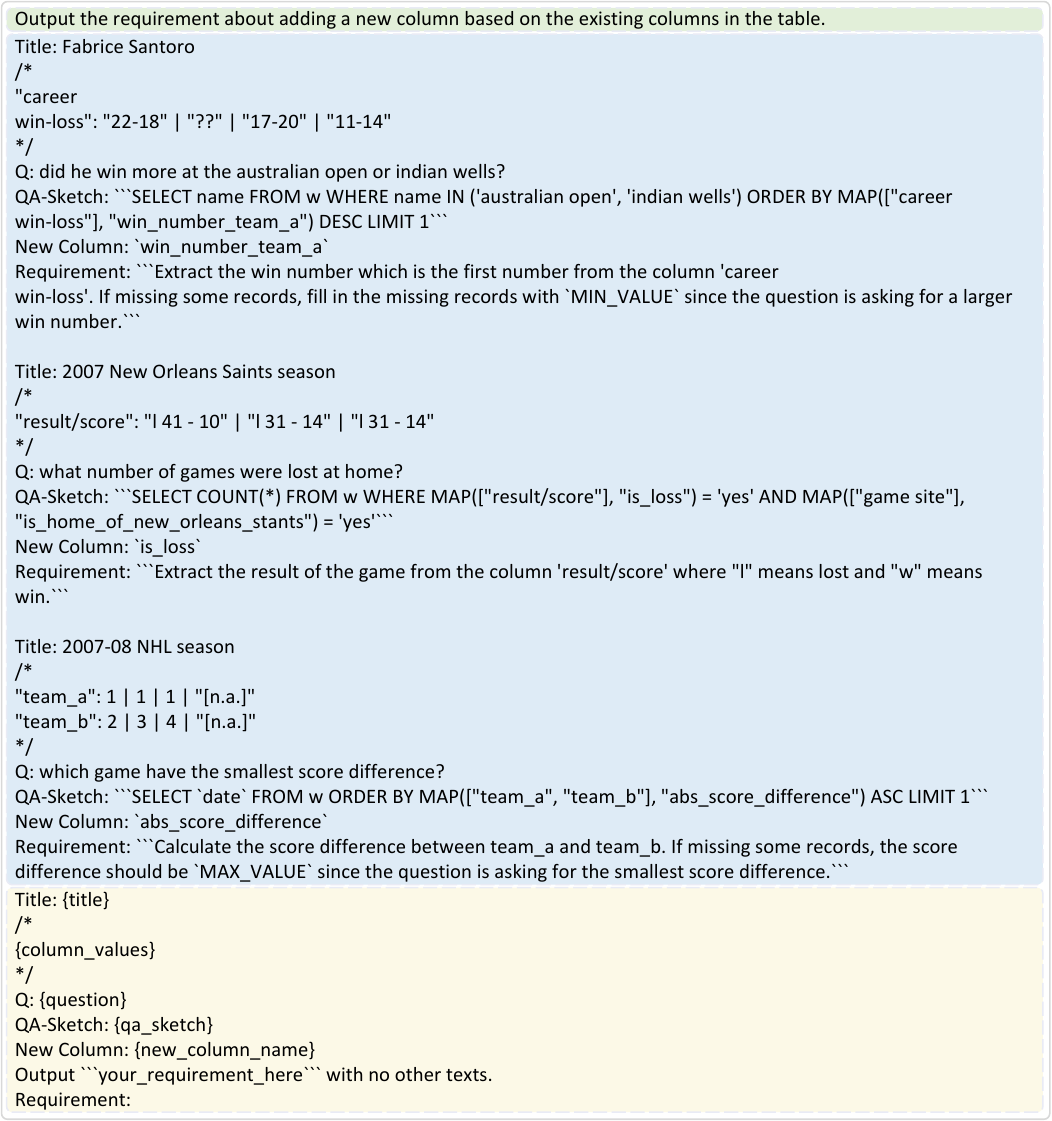}
    \vspace{-1em}
    \caption{Prompt of Planner on generating requirement for Derive Operator.
    %, such as NL2SQL as shown in the figure. \sys decomposes the data prep process into three stages: \textcircled{1} The Planning stage, \textcircled{2} the Programming stage and \textcircled{3} the Executing stage.
    }
    \label{fig:prompt_planner_generate_req_aug}
    % \vspace{-1em}
\end{figure*}
