# Supplementary material for: AutoPrep: Natural Language Question-Aware Data Preparation with a Multi-Agent Framework
Source: arXiv:2412.10422 source file (2025-07-09)
Supplement: Supplementary file 22 [file prompts_in_autoprep.tex]

\section{Prompts in \sys}
\label{appendix:prompts_in_autoprep}

The representative demonstration examples and prompts used by \sys are presented. 

\subsection{Prompts in Planner Agent}

%!TEX root = ../../main.tex
\begin{figure*}[!t]
    \centering 
    \includegraphics[width=0.85\textwidth]{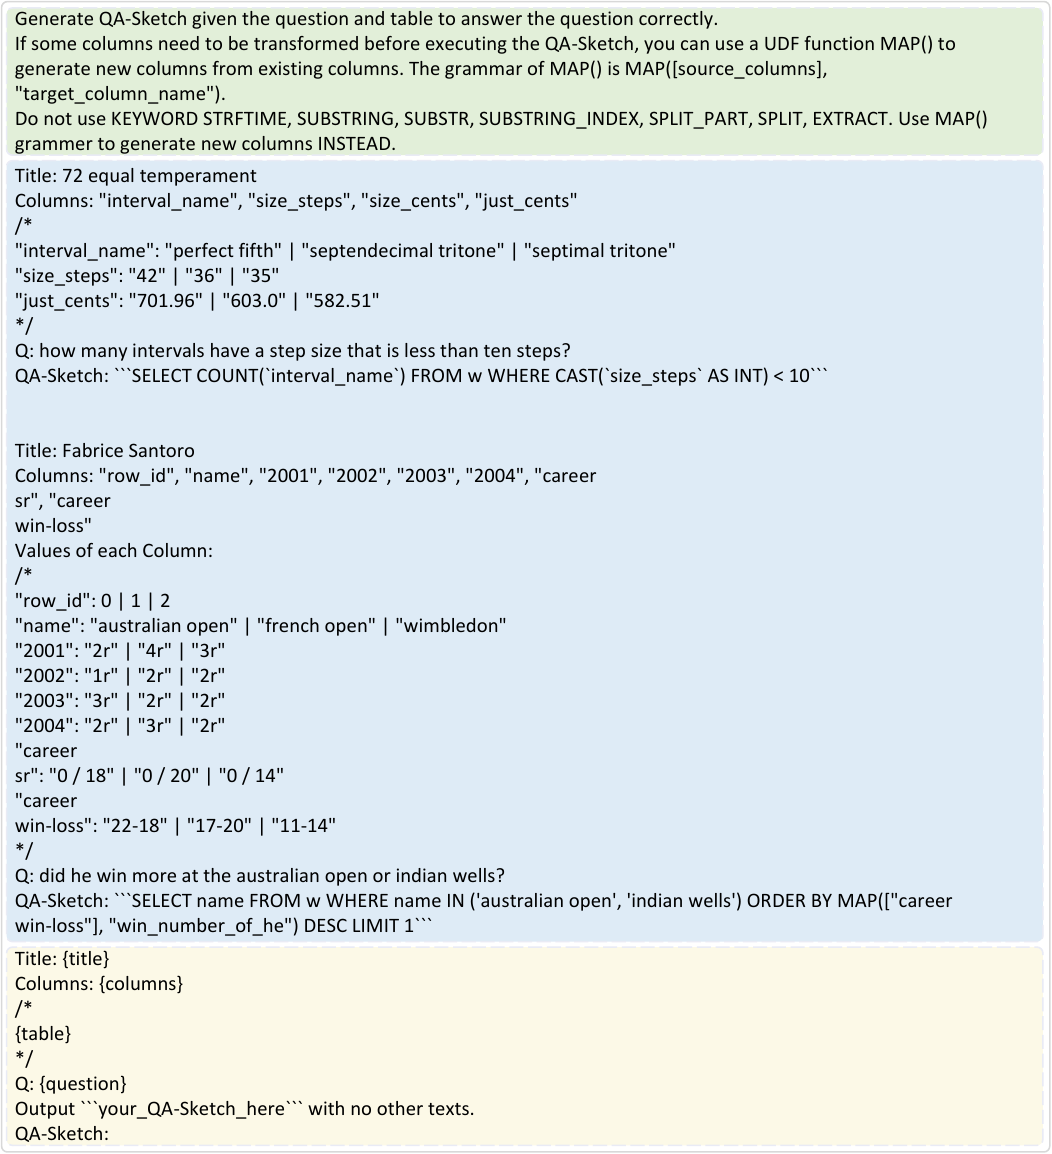}
    \vspace{-1em}
    \caption{Prompt of Planner on generating Analysis Sketch on WikiTQ Dataset.
    %, such as NL2SQL as shown in the figure. \sys decomposes the data prep process into three stages: \textcircled{1} The Planning stage, \textcircled{2} the Programming stage and \textcircled{3} the Executing stage.
    }
    \label{fig:prompt_planner_analysis_sketch_wikitq}
    % \vspace{-1em}
\end{figure*}
%!TEX root = ../../main.tex
\begin{figure*}[!t]
    \centering 
    \includegraphics[width=0.90\textwidth]{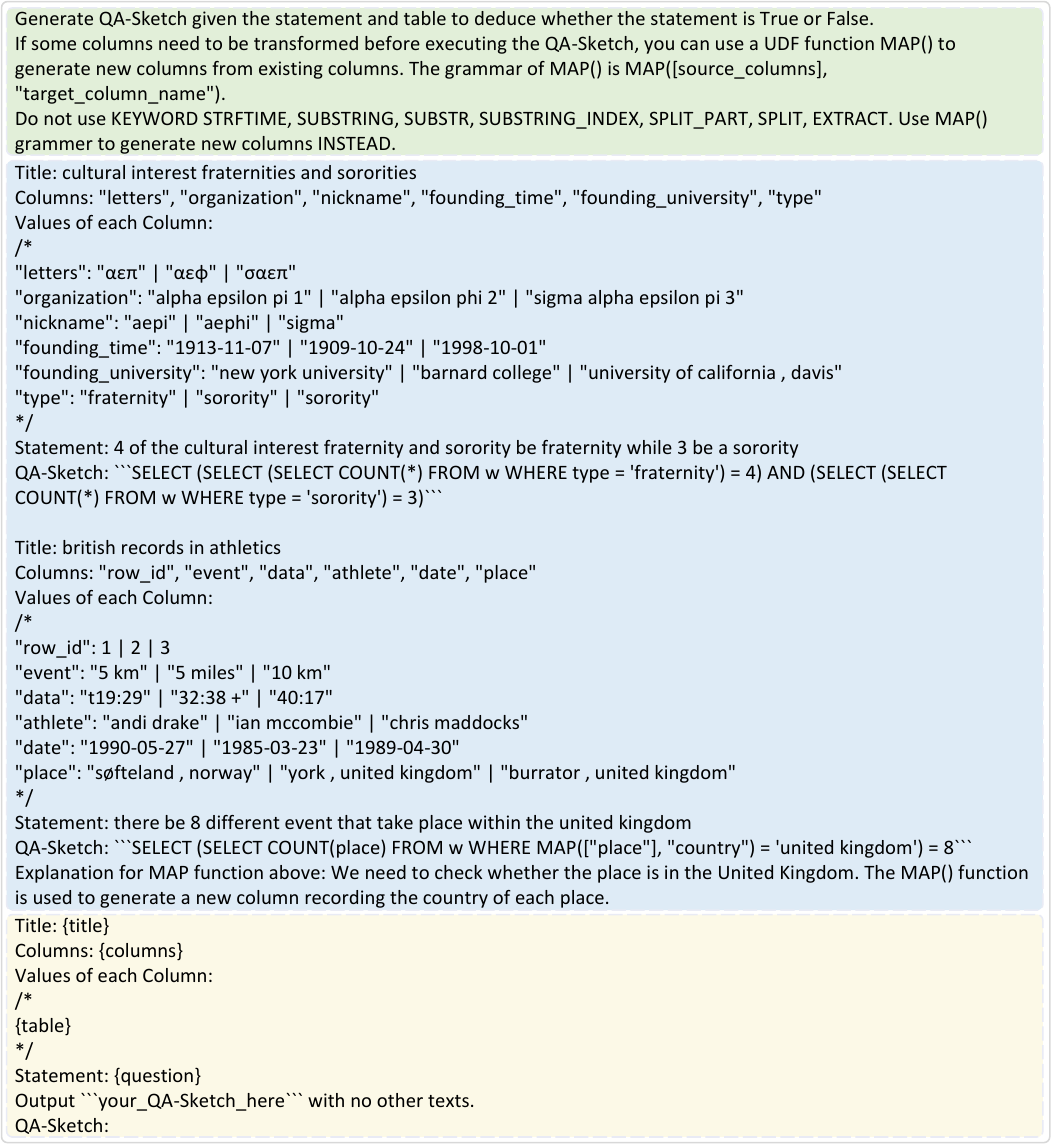}
    \vspace{-1em}
    \caption{Prompt of Planner on generating Analysis Sketch on TabFact Dataset.
    %, such as NL2SQL as shown in the figure. \sys decomposes the data prep process into three stages: \textcircled{1} The Planning stage, \textcircled{2} the Programming stage and \textcircled{3} the Executing stage.
    }
    \label{fig:prompt_planner_analysis_sketch_tabfact}
    % \vspace{-1em}
\end{figure*}

%!TEX root = ../../main.tex
\begin{figure*}[!t]
    \centering 
    \includegraphics[width=0.9\textwidth]{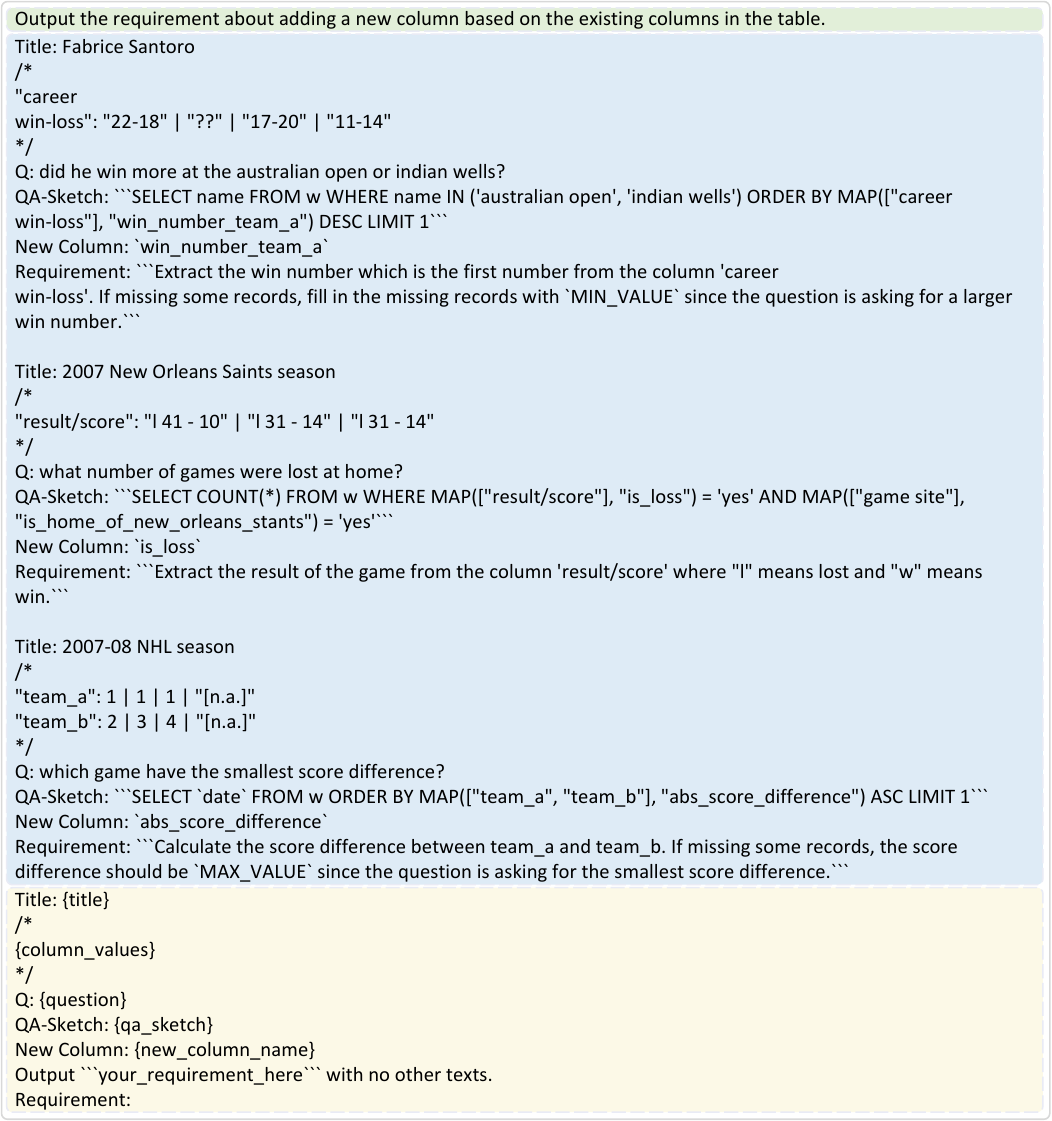}
    \vspace{-1em}
    \caption{Prompt of Planner on generating requirement for Derive Operator.
    %, such as NL2SQL as shown in the figure. \sys decomposes the data prep process into three stages: \textcircled{1} The Planning stage, \textcircled{2} the Programming stage and \textcircled{3} the Executing stage.
    }
    \label{fig:prompt_planner_generate_req_aug}
    % \vspace{-1em}
\end{figure*}
%!TEX root = ../../main.tex
\begin{figure*}[!t]
    \centering 
    \includegraphics[width=0.9\textwidth]{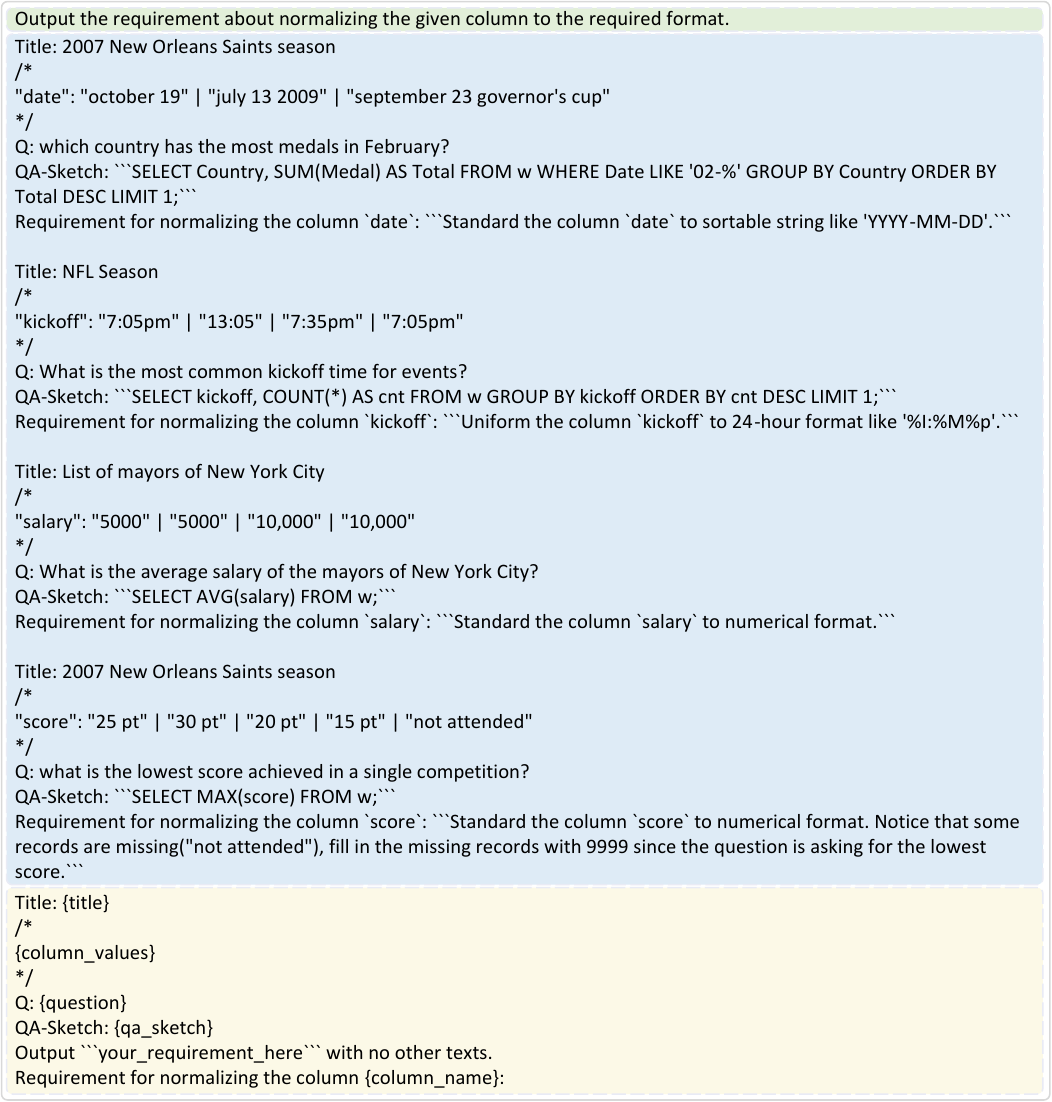}
    \vspace{-1em}
    \caption{Prompt of Planner on generating requirement for Normalize Operator.
    %, such as NL2SQL as shown in the figure. \sys decomposes the data prep process into three stages: \textcircled{1} The Planning stage, \textcircled{2} the Programming stage and \textcircled{3} the Executing stage.
    }
    \label{fig:prompt_planner_generate_req_norm}
    % \vspace{-1em}
\end{figure*}

The \textsc{Planner} aims at generating logical operators in two stages: (1) generate the QA-Sketch. (2) generate specific requirement for Normalize and Derive.

In the first stage, \sys analyzes the table and the question to generate the reasoning process of question answering over table with the assistance of pseudo codes. In this paper, we define the grammar of the pseudo code as SQL with a UDF grammar. The prompts for WikITQ and TabFact datasets are shown in Figure~\ref{fig:prompt_planner_analysis_sketch_wikitq} and Figure~\ref{fig:prompt_planner_analysis_sketch_tabfact}. Next, based on the generated QA-Sketch, we extract each operation clause and provide the related column data in the clause to query LLMs to generate specific requirement of the logical operator. The prompts of generating specific requirement for each type of logical operator are shown in Figure~\ref{fig:prompt_planner_generate_req_aug} and Figure~\ref{fig:prompt_planner_generate_req_norm}. Notice that the Filter operator is generated by analyzing the QA-Sketch and the arguments of Derive operator, which does not need to query LLMs.

\subsection{Prompts in Programmer Agents}

%!TEX root = ../../main.tex
\begin{figure*}[!t]
    \centering 
    \includegraphics[width=0.99\textwidth]{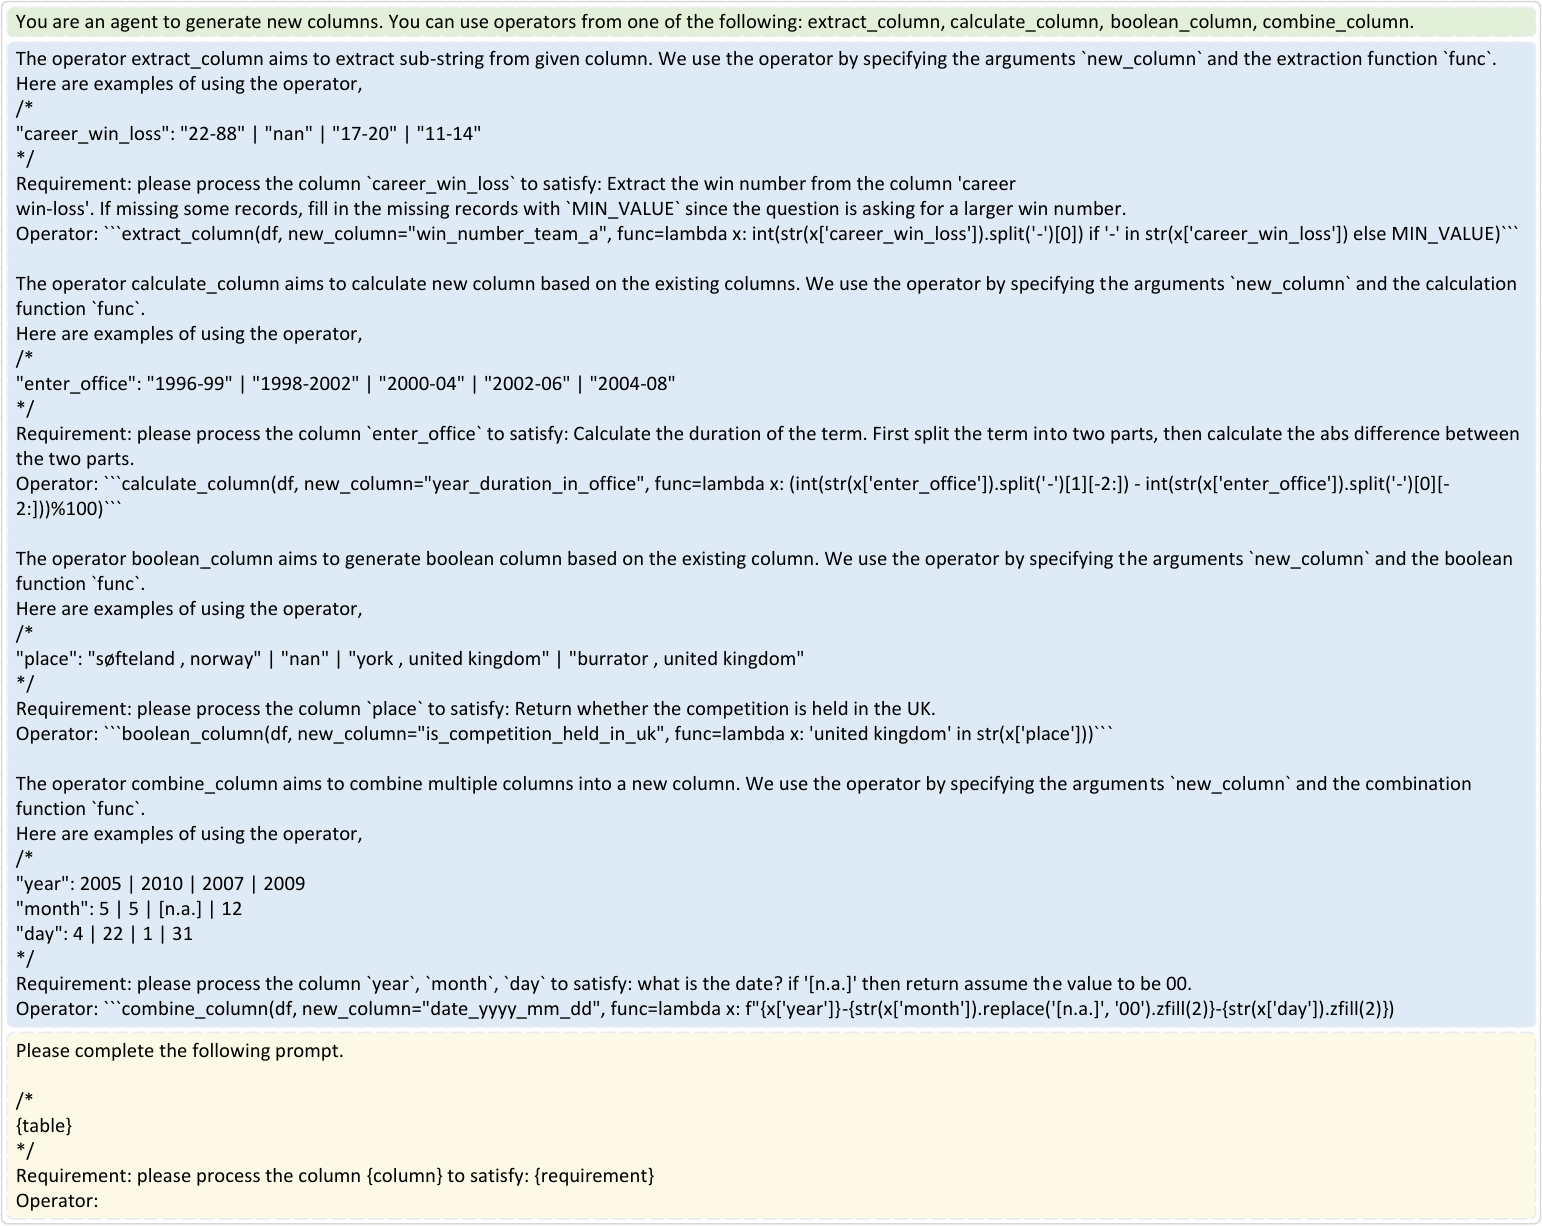}
    \vspace{-1em}
    \caption{Prompt of Derive.
    %, such as NL2SQL as shown in the figure. \sys decomposes the data prep process into three stages: \textcircled{1} The Planning stage, \textcircled{2} the Programming stage and \textcircled{3} the Executing stage.
    }
    \label{fig:prompt_augment}
    % \vspace{-1em}
\end{figure*}
%!TEX root = ../../main.tex
\begin{figure*}[!t]
    \centering 
    \includegraphics[width=0.9\textwidth]{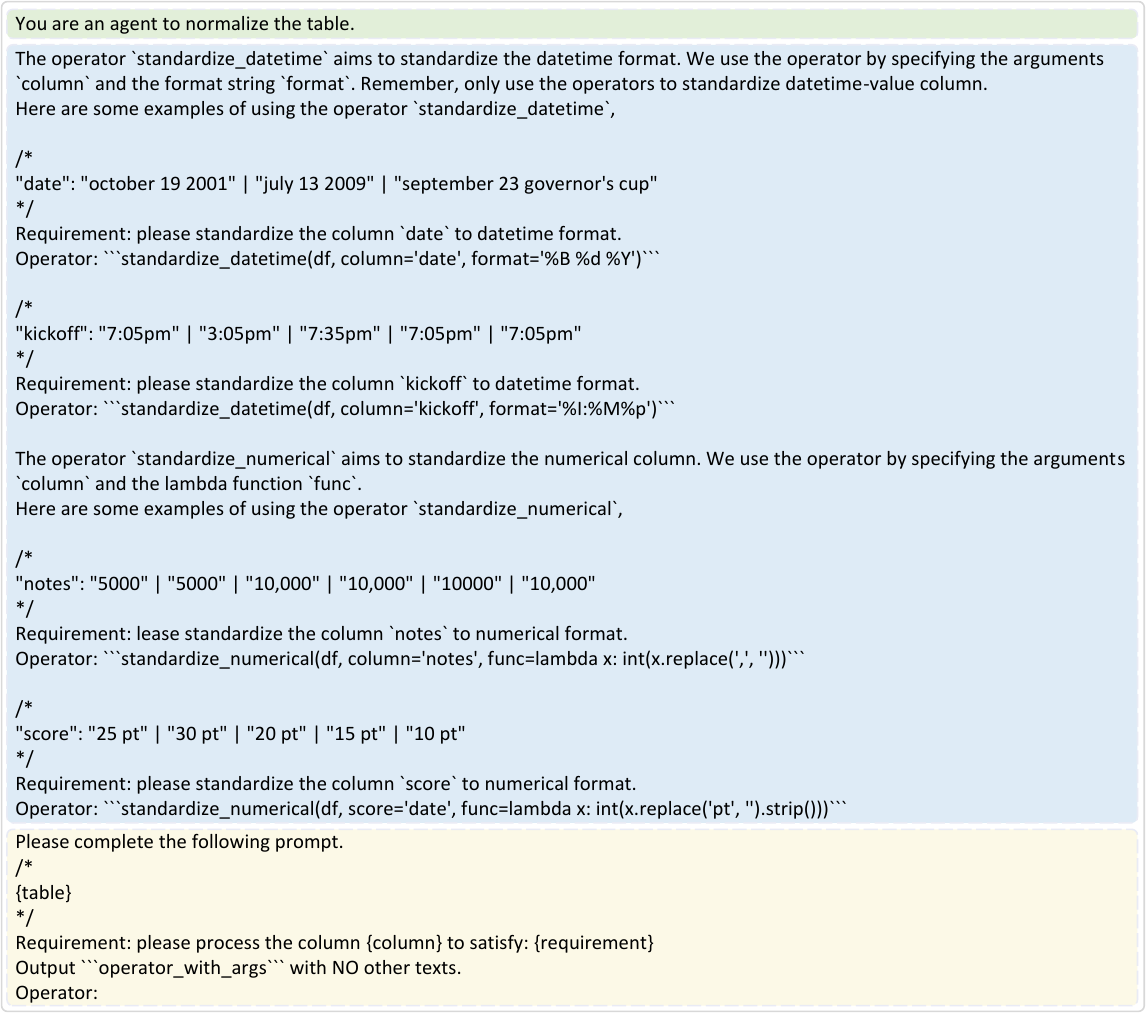}
    \vspace{-1em}
    \caption{Prompt of Normalize.
    %, such as NL2SQL as shown in the figure. \sys decomposes the data prep process into three stages: \textcircled{1} The Planning stage, \textcircled{2} the Programming stage and \textcircled{3} the Executing stage.
    }
    \label{fig:prompt_normalizer}
    % \vspace{-1em}
\end{figure*}
%!TEX root = ../../main.tex
\begin{figure*}[!t]
    \centering 
    \includegraphics[width=0.90\textwidth]{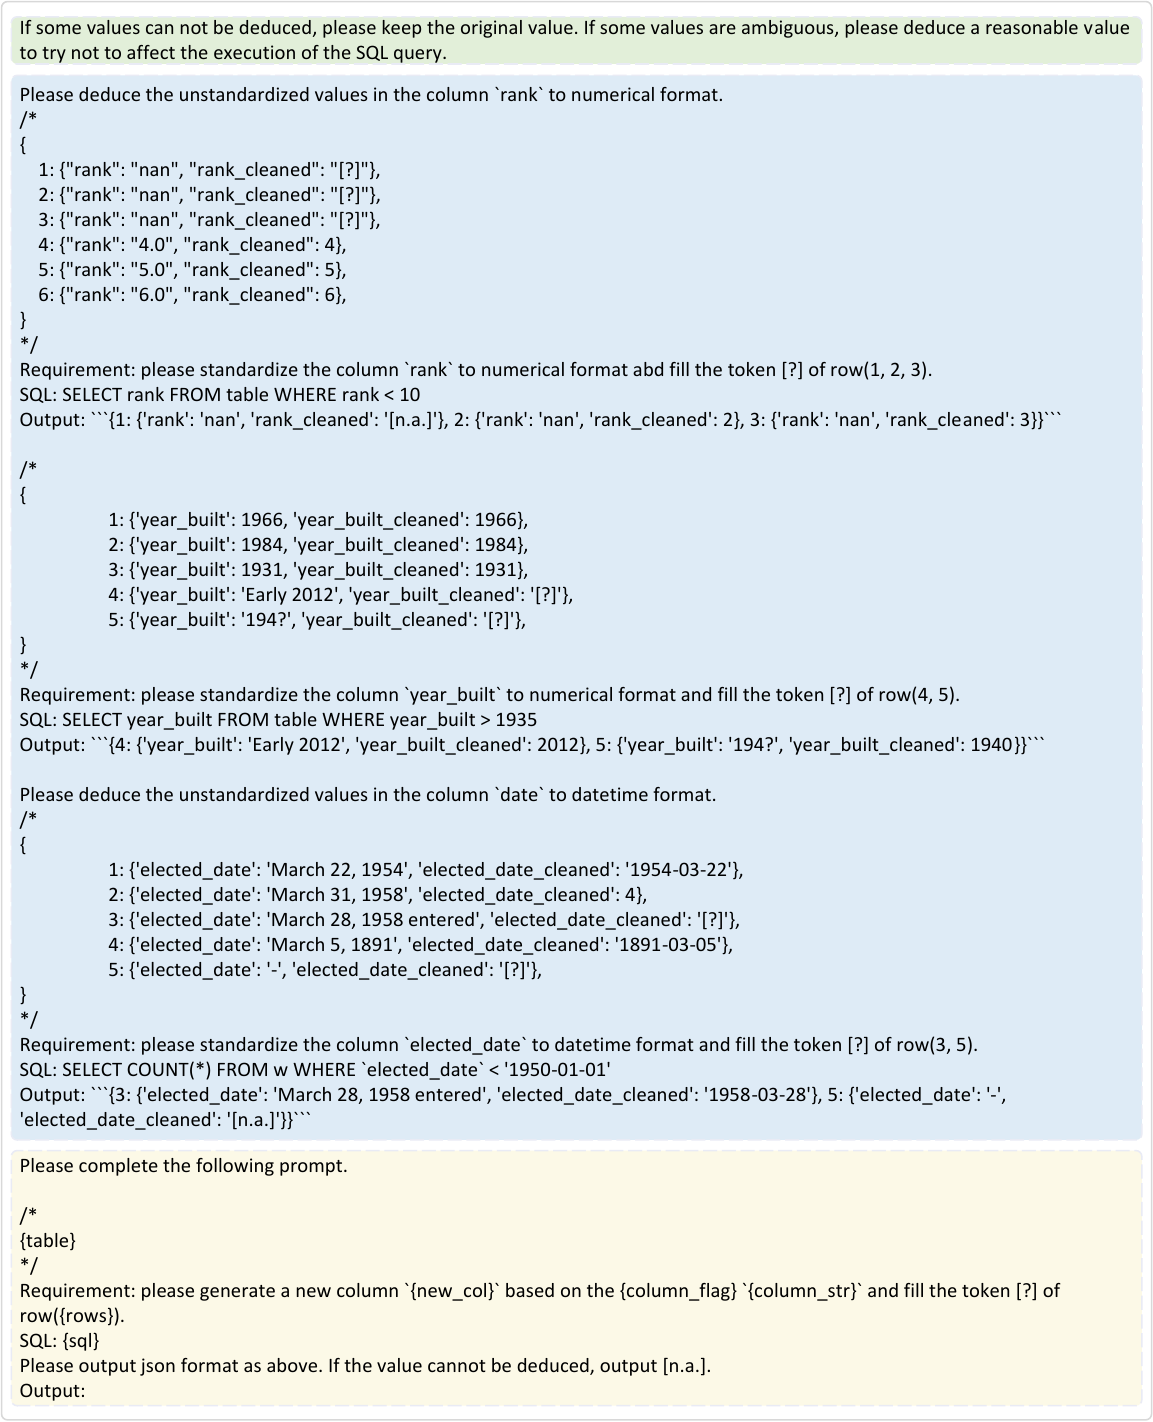}
    \vspace{-1em}
    \caption{Prompt of Imputater.
    %, such as NL2SQL as shown in the figure. \sys decomposes the data prep process into three stages: \textcircled{1} The Planning stage, \textcircled{2} the Programming stage and \textcircled{3} the Executing stage.
    }
    \label{fig:prompt_imputate}
    % \vspace{-1em}
\end{figure*}
%!TEX root = ../../main.tex
\begin{figure*}[!t]
    \centering 
    \includegraphics[width=0.90\textwidth]{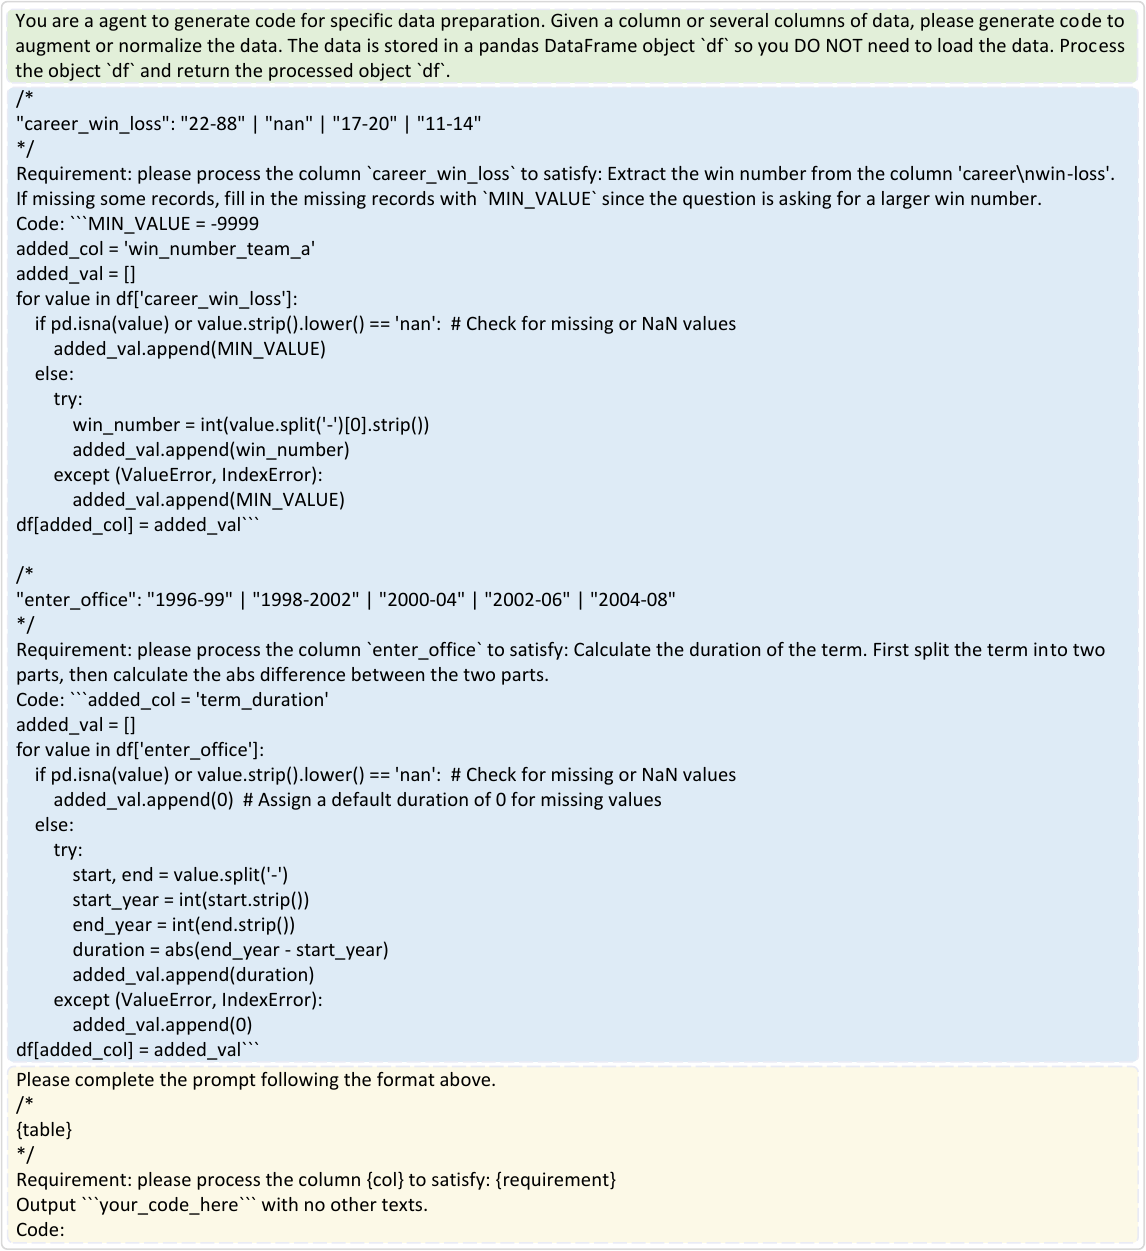}
    \vspace{-1em}
    \caption{Prompt of LLM Coder.
    %, such as NL2SQL as shown in the figure. \sys decomposes the data prep process into three stages: \textcircled{1} The Planning stage, \textcircled{2} the Programming stage and \textcircled{3} the Executing stage.
    }
    \label{fig:prompt_llm_code}
    % \vspace{-1em}
\end{figure*}

Given logical operators with specific requirement and related columns, the programmer agents generate physical operators to implement the logical operators. The prompts of \textsc{Derive} and \textsc{Normalize} are shown in Figure~\ref{fig:prompt_augment} and Figure~\ref{fig:prompt_normalizer}. In addition, if any logical operators can not be implemented with functions in the function pool, we call LLMs to generate Python codes. The prompt of generating Python code is shown in Figure~\ref{fig:prompt_llm_code}. Finally, if any values can not be derived or normalized, we call an Imputater agent to direct infer the correct values. The prompt is shown in Figure~\ref{fig:prompt_imputate}.

\subsection{Prompts in other baselines}

%!TEX root = ../../main.tex
\begin{figure*}[!t]
    \centering 
    \includegraphics[width=0.95\textwidth]{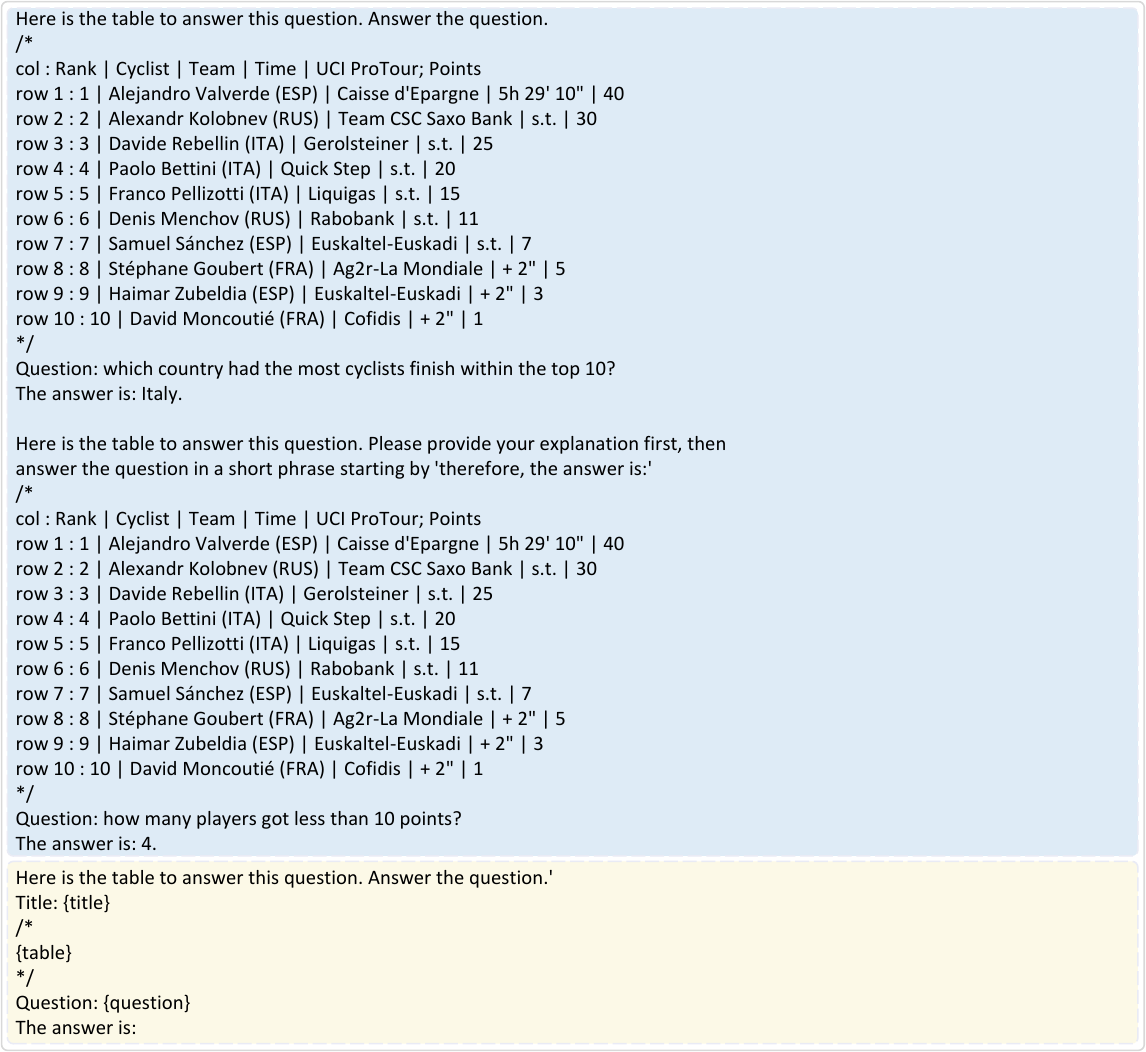}
    \vspace{-1em}
    \caption{Prompt of End2End method on WikiTQ dataset.
    %, such as NL2SQL as shown in the figure. \sys decomposes the data prep process into three stages: \textcircled{1} The Planning stage, \textcircled{2} the Programming stage and \textcircled{3} the Executing stage.
    }
    \label{fig:prompt_end2end_wikitq}
    % \vspace{-1em}
\end{figure*}
%!TEX root = ../../main.tex
\begin{figure*}[!t]
    \centering 
    \includegraphics[width=0.70\textwidth]{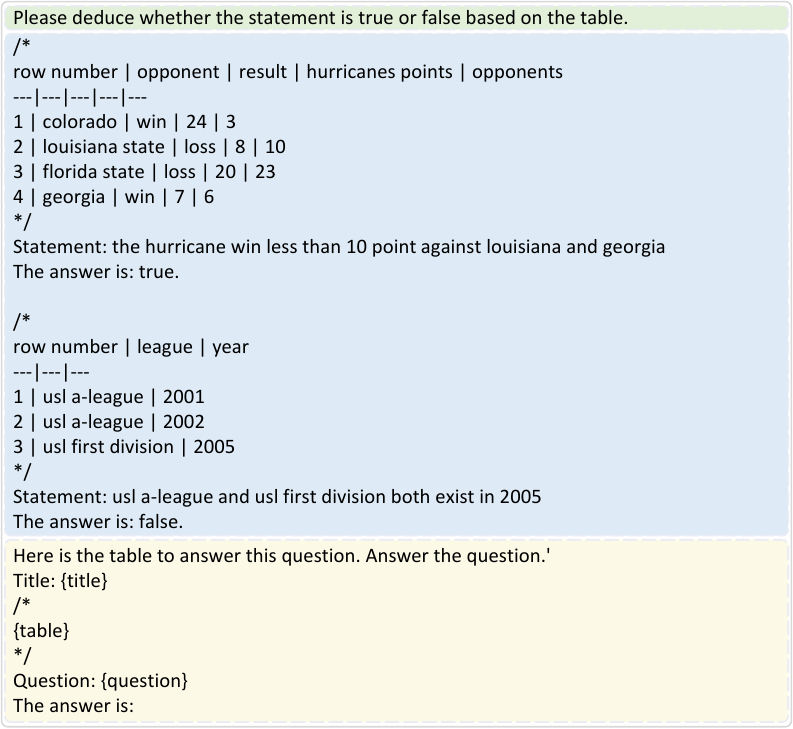}
    \vspace{-1em}
    \caption{Prompt of End2End method on TabFact dataset.
    %, such as NL2SQL as shown in the figure. \sys decomposes the data prep process into three stages: \textcircled{1} The Planning stage, \textcircled{2} the Programming stage and \textcircled{3} the Executing stage.
    }
    \label{fig:prompt_end2end_tabfact}
    % \vspace{-1em}
\end{figure*}

%!TEX root = ../../main.tex
\begin{figure*}[!t]
    \centering 
    \includegraphics[width=0.99\textwidth]{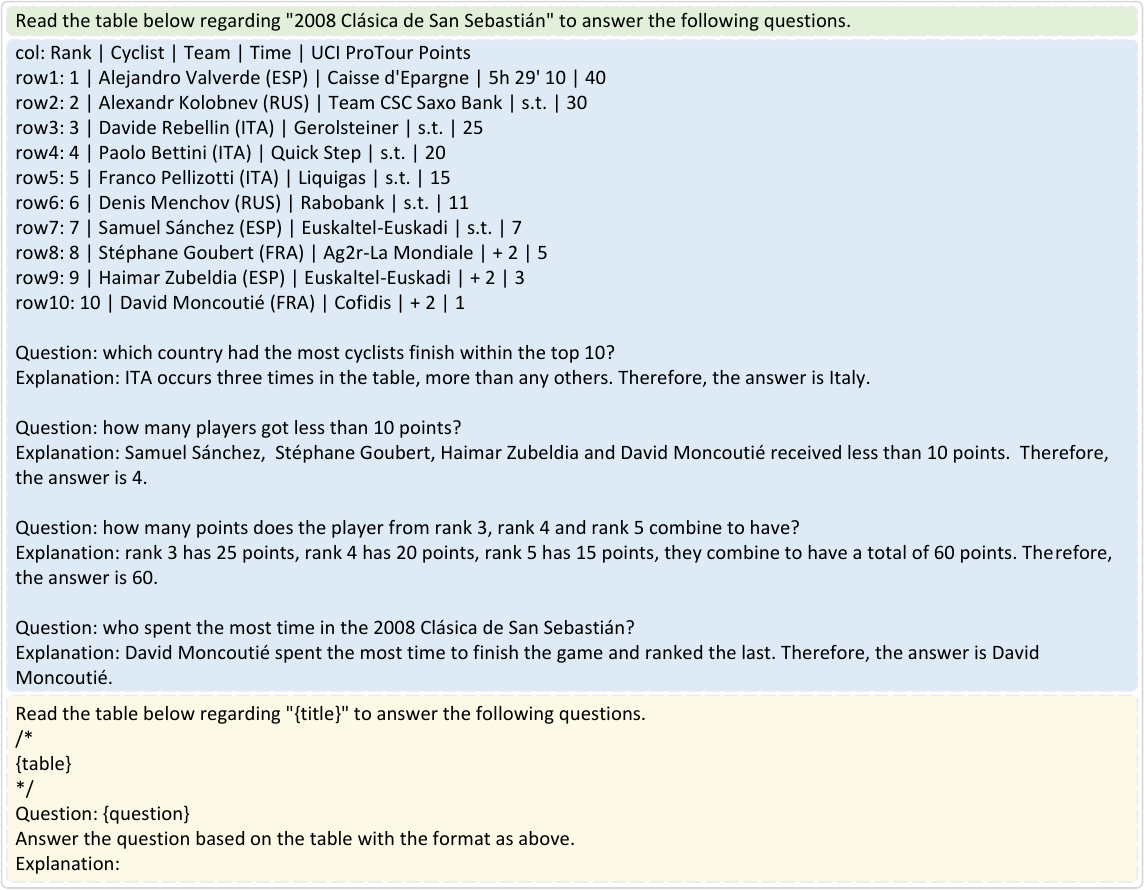}
    \vspace{-1em}
    \caption{Prompt of Chain-of-Thought TQA method on WikiTQ dataset.
    %, such as NL2SQL as shown in the figure. \sys decomposes the data prep process into three stages: \textcircled{1} The Planning stage, \textcircled{2} the Programming stage and \textcircled{3} the Executing stage.
    }
    \label{fig:prompt_cot_wikitq}
    % \vspace{-1em}
\end{figure*}
%!TEX root = ../../main.tex
\begin{figure*}[!t]
    \centering 
    \includegraphics[width=0.85\textwidth]{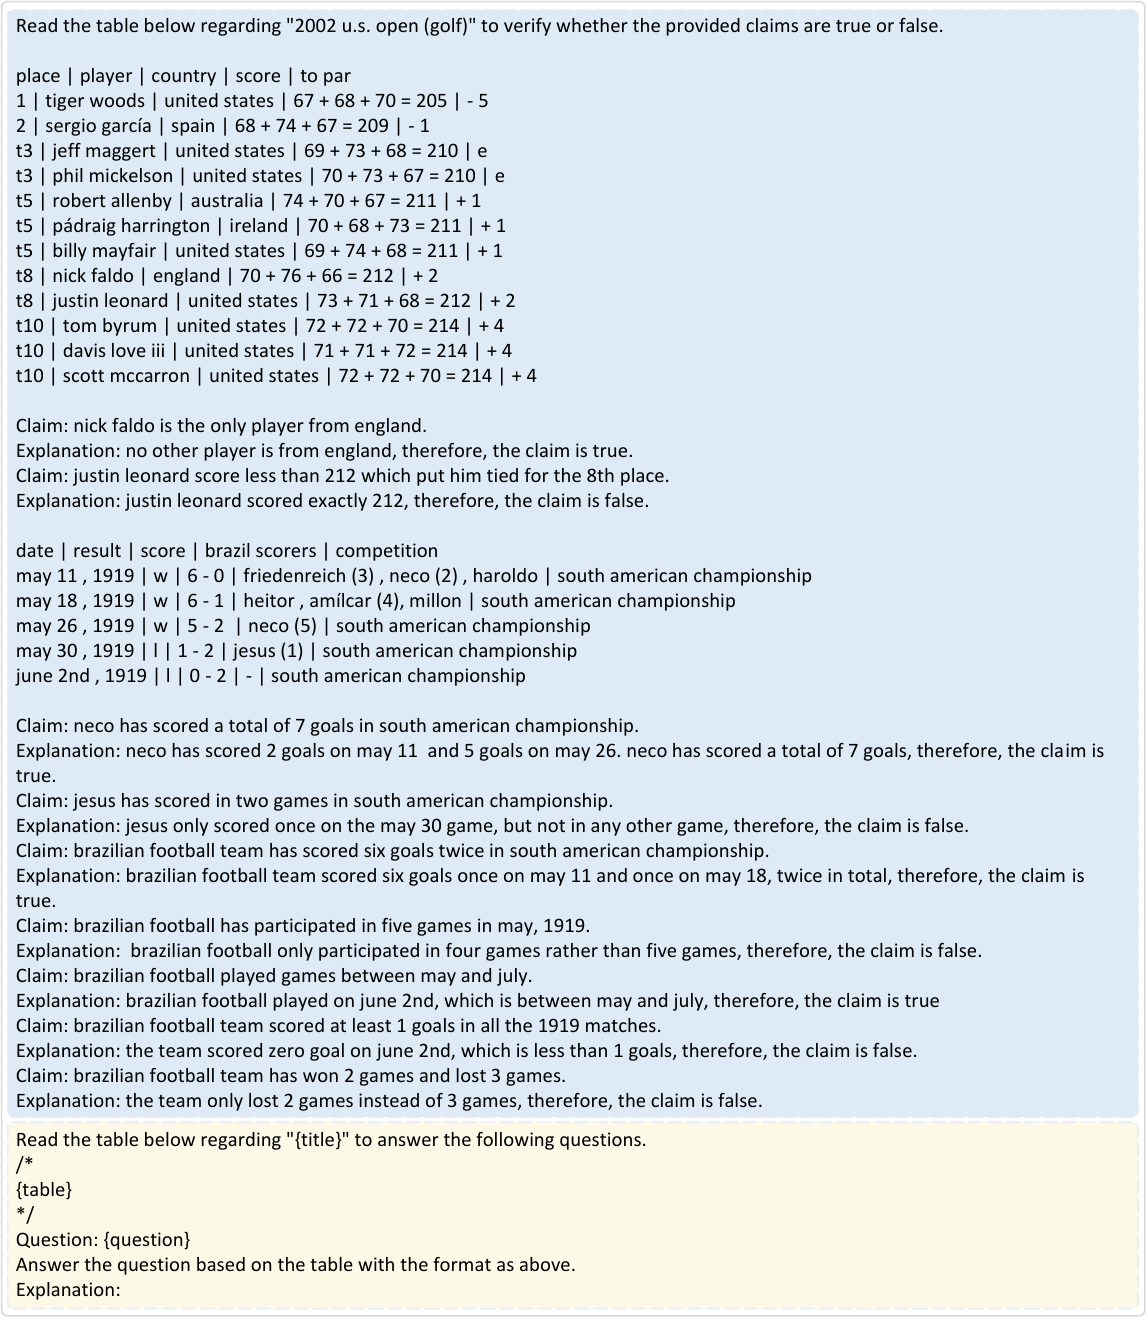}
    \vspace{-1em}
    \caption{Prompt of Chain-of-Thought TQA method on TabFact dataset.
    %, such as NL2SQL as shown in the figure. \sys decomposes the data prep process into three stages: \textcircled{1} The Planning stage, \textcircled{2} the Programming stage and \textcircled{3} the Executing stage.
    }
    \label{fig:prompt_cot_tabfact}
    % \vspace{-1em}
\end{figure*}

%!TEX root = ../../main.tex
\begin{figure*}[!t]
    \centering 
    \includegraphics[width=0.85\textwidth]{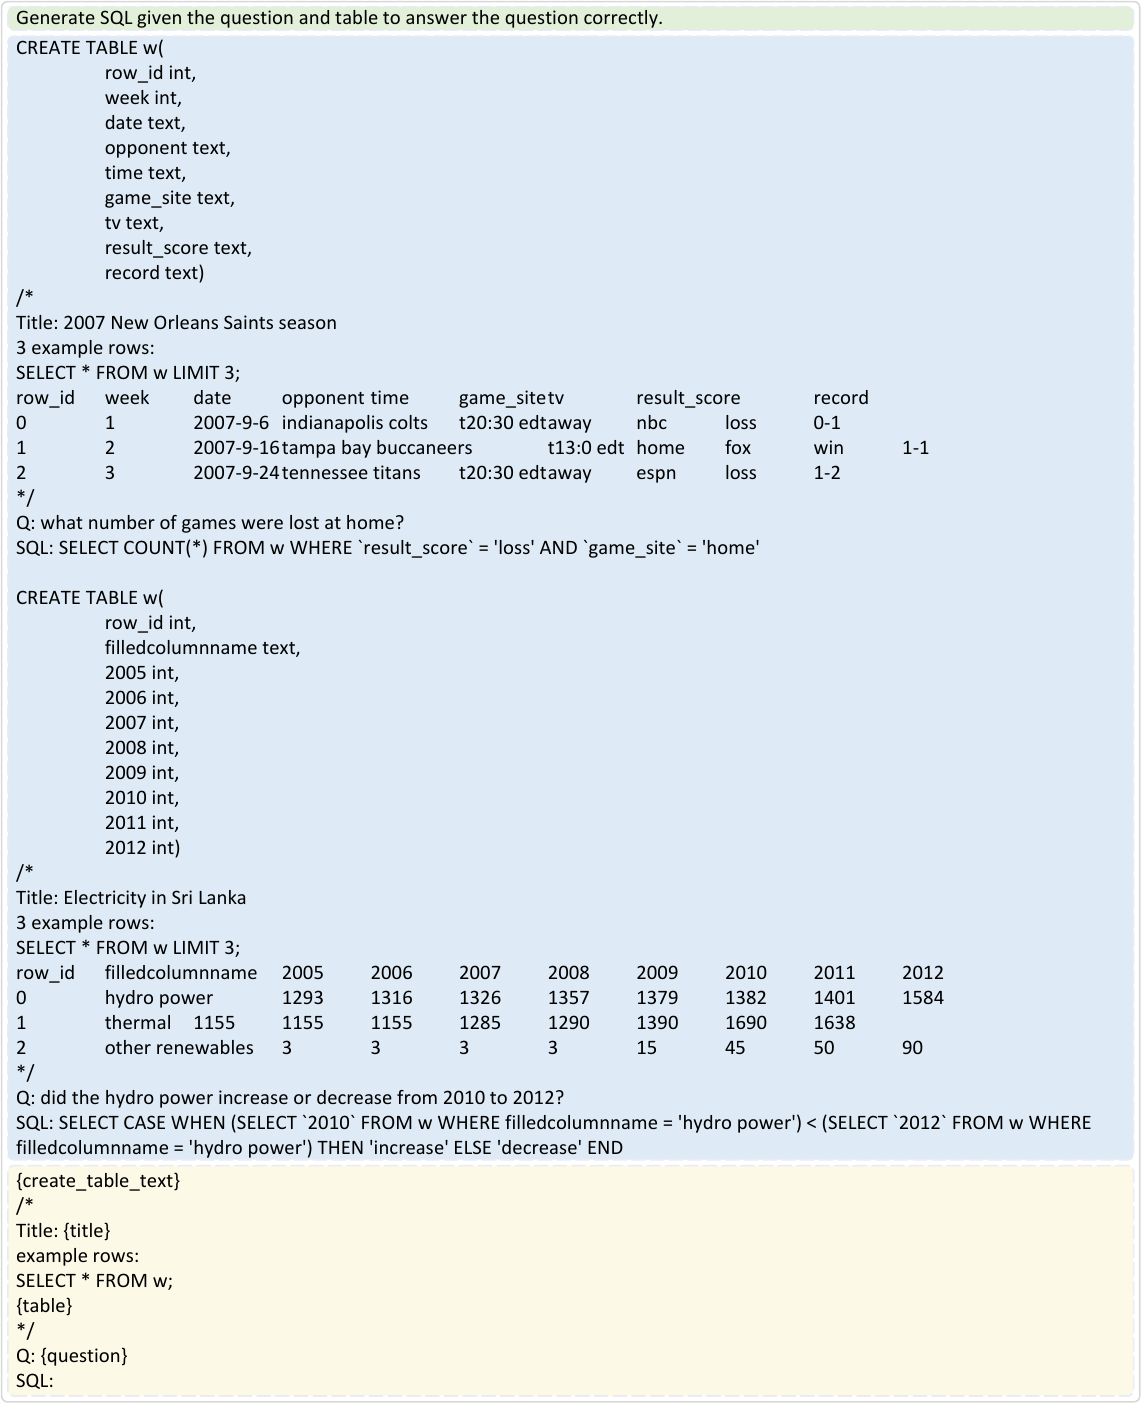}
    \vspace{-1em}
    \caption{Prompt of NL2SQL on WikiTQ dataset.
    %, such as NL2SQL as shown in the figure. \sys decomposes the data prep process into three stages: \textcircled{1} The Planning stage, \textcircled{2} the Programming stage and \textcircled{3} the Executing stage.
    }
    \label{fig:prompt_nl2sql_wikitq}
    % \vspace{-1em}
\end{figure*}
%!TEX root = ../../main.tex
\begin{figure*}[!t]
    \centering 
    \includegraphics[width=0.99\textwidth]{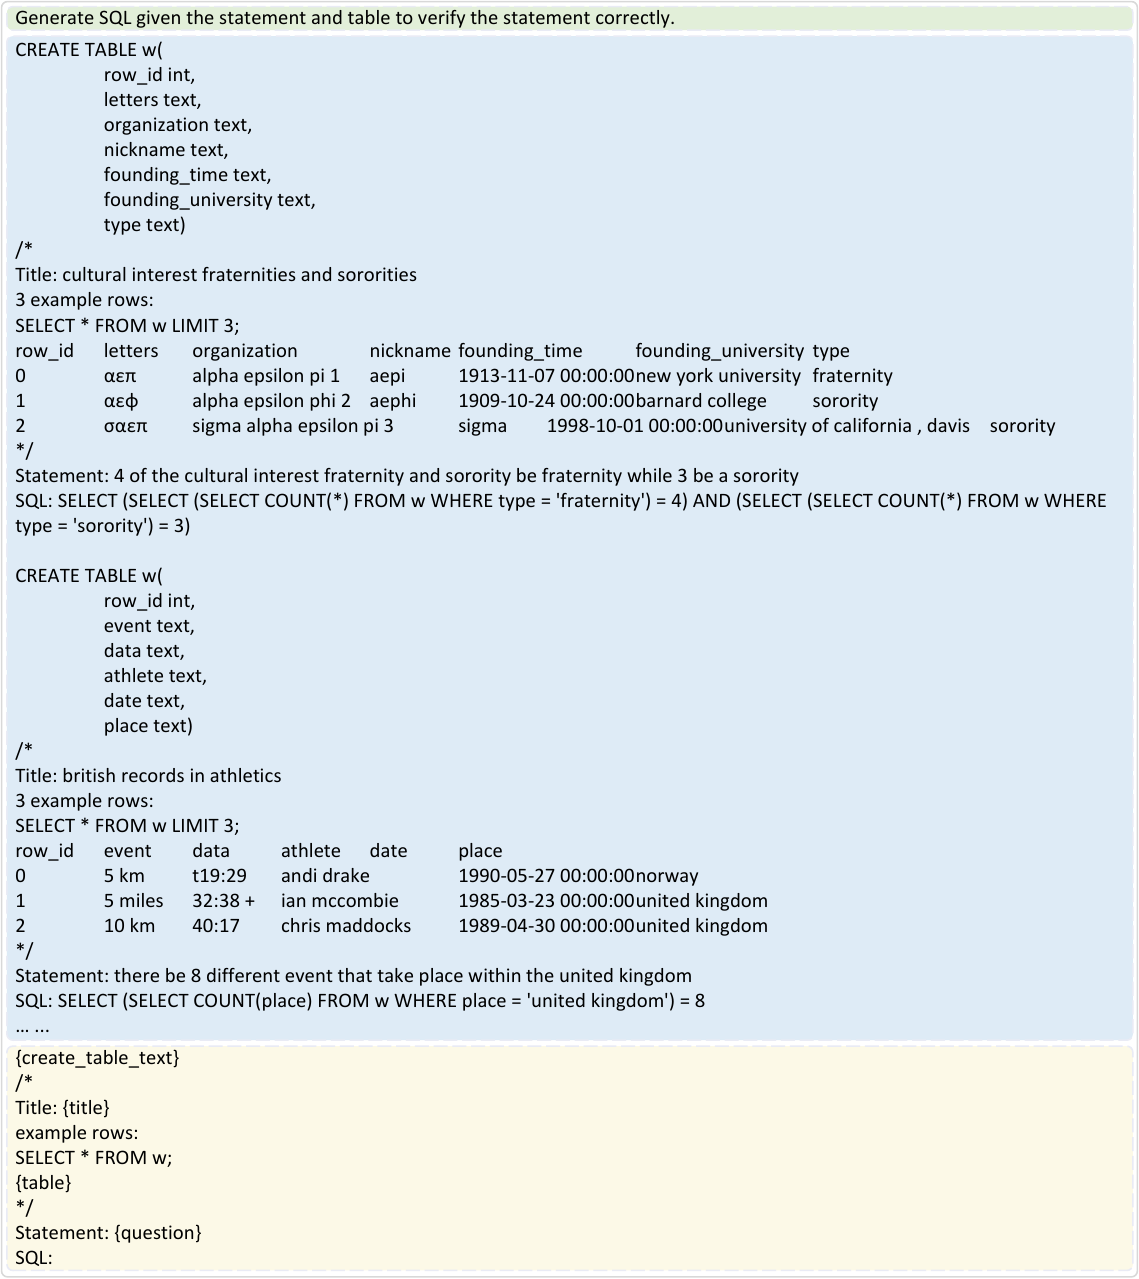}
    \vspace{-1em}
    \caption{Prompt of NL2SQL on TabFact dataset.
    %, such as NL2SQL as shown in the figure. \sys decomposes the data prep process into three stages: \textcircled{1} The Planning stage, \textcircled{2} the Programming stage and \textcircled{3} the Executing stage.
    }
    \label{fig:prompt_nl2sql_tabfact}
    % \vspace{-1em}
\end{figure*}

%!TEX root = ../../main.tex
\begin{figure*}[!t]
    \centering 
    \includegraphics[width=0.99\textwidth]{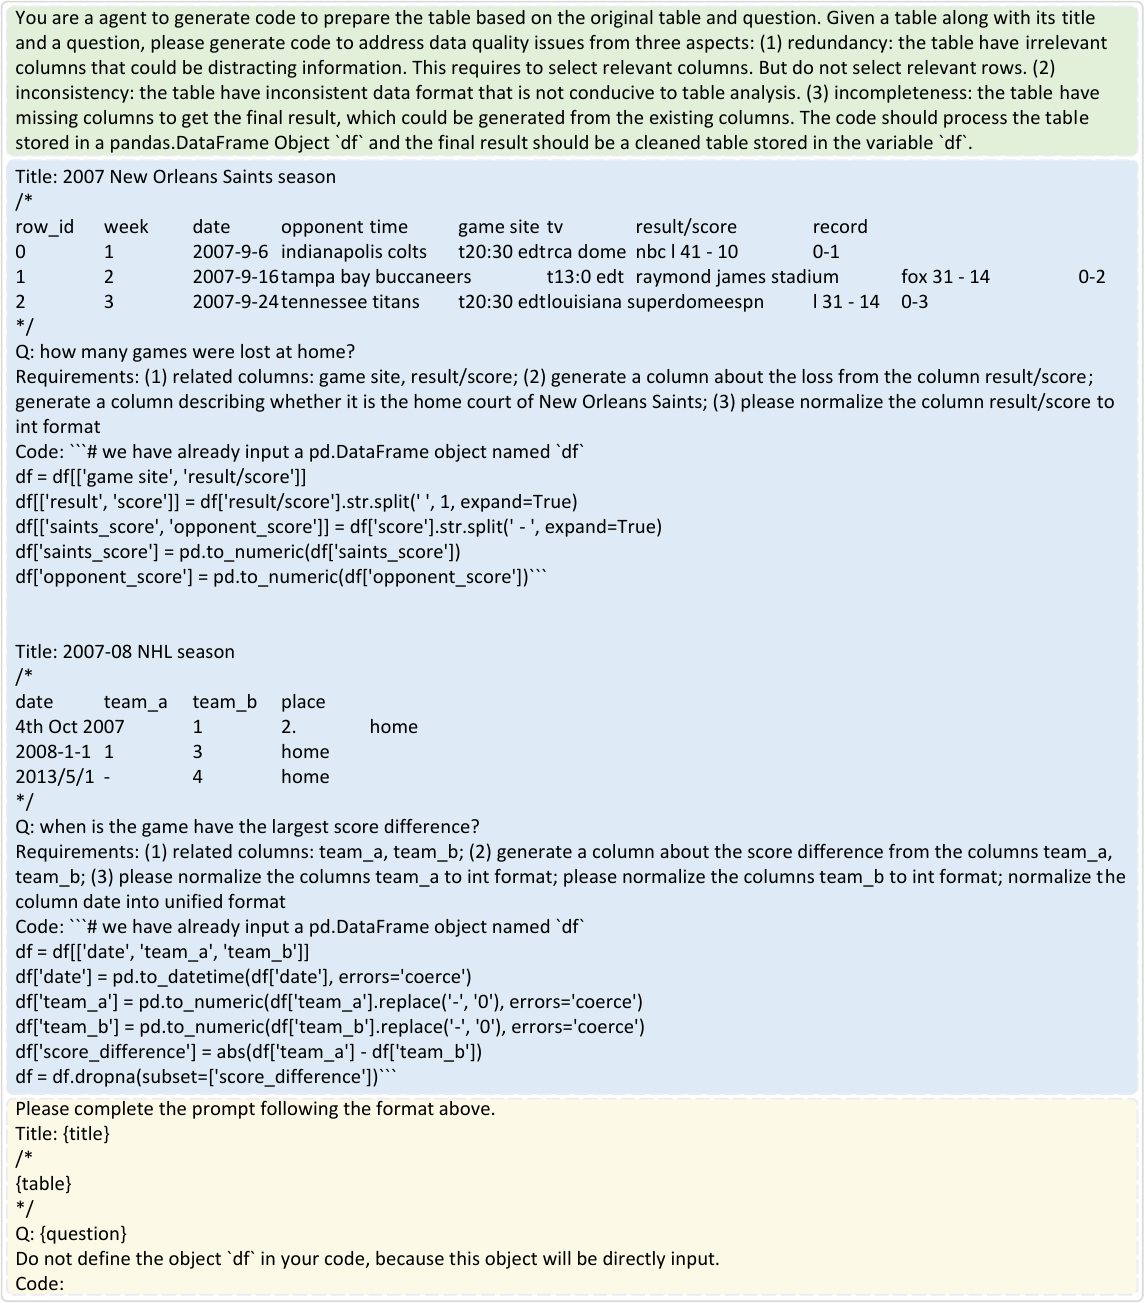}
    \vspace{-1em}
    \caption{Prompt of ICL-Prep on WikiTQ dataset.
    %, such as NL2SQL as shown in the figure. \sys decomposes the data prep process into three stages: \textcircled{1} The Planning stage, \textcircled{2} the Programming stage and \textcircled{3} the Executing stage.
    }
    \label{fig:prompt_iclprep_wikitq}
    % \vspace{-1em}
\end{figure*}
%!TEX root = ../../main.tex
\begin{figure*}[!t]
    \centering 
    \includegraphics[width=0.99\textwidth]{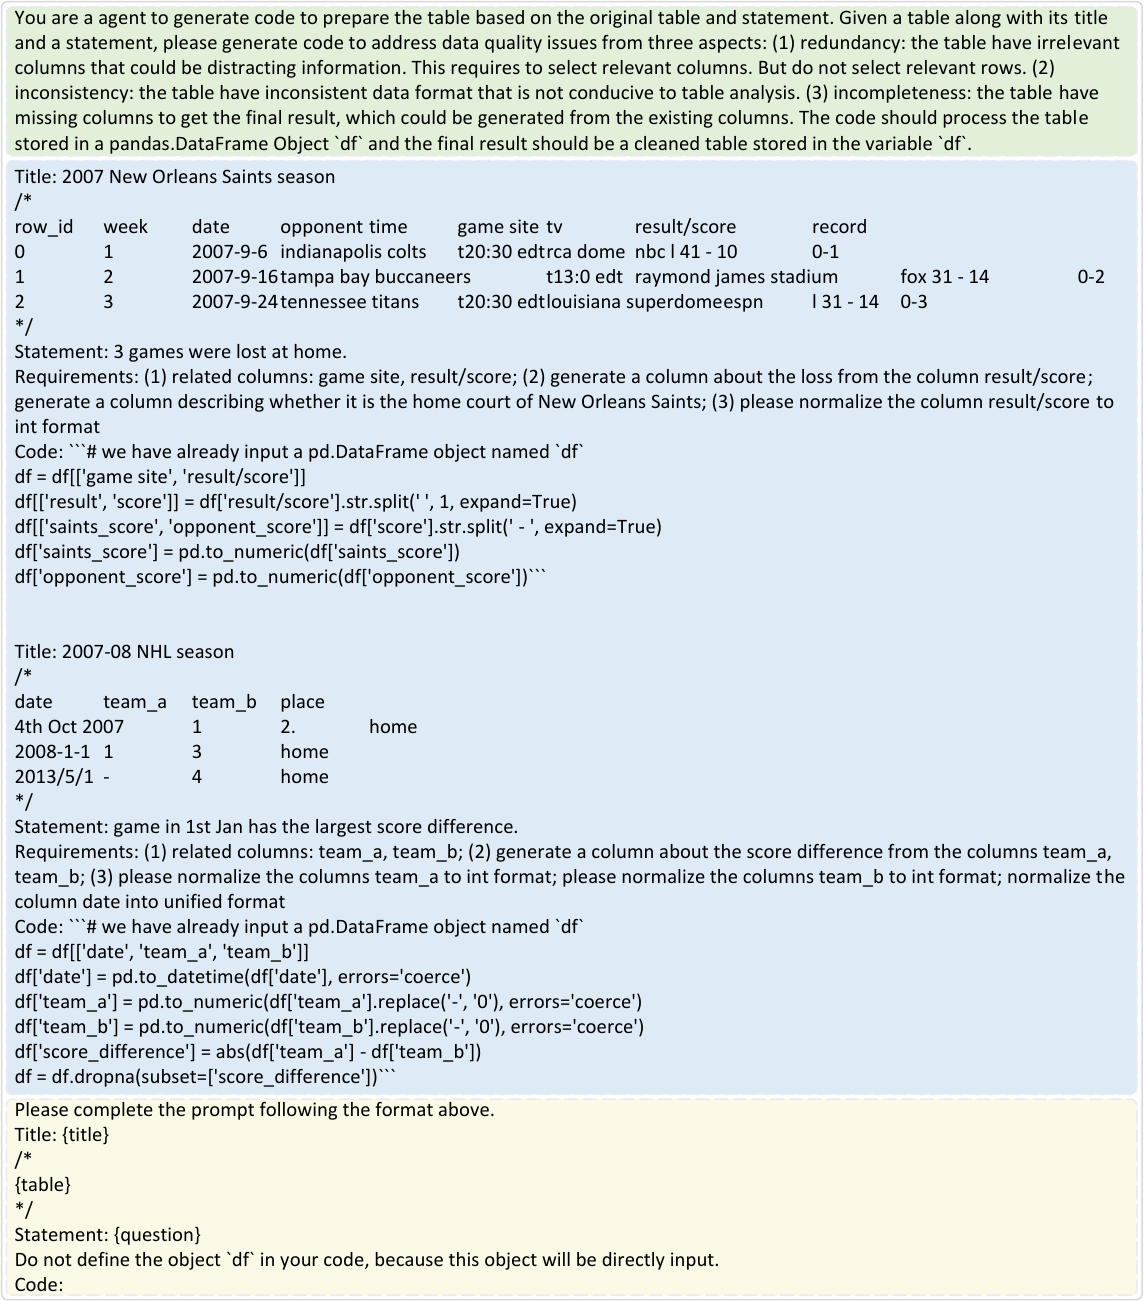}
    \vspace{-1em}
    \caption{Prompt of ICL-Prep on TabFact dataset.
    %, such as NL2SQL as shown in the figure. \sys decomposes the data prep process into three stages: \textcircled{1} The Planning stage, \textcircled{2} the Programming stage and \textcircled{3} the Executing stage.
    }
    \label{fig:prompt_iclprep_tabfact}
    % \vspace{-1em}
\end{figure*}

%!TEX root = ../../main.tex
\begin{figure*}[!t]
    \centering 
    \includegraphics[width=0.99\textwidth]{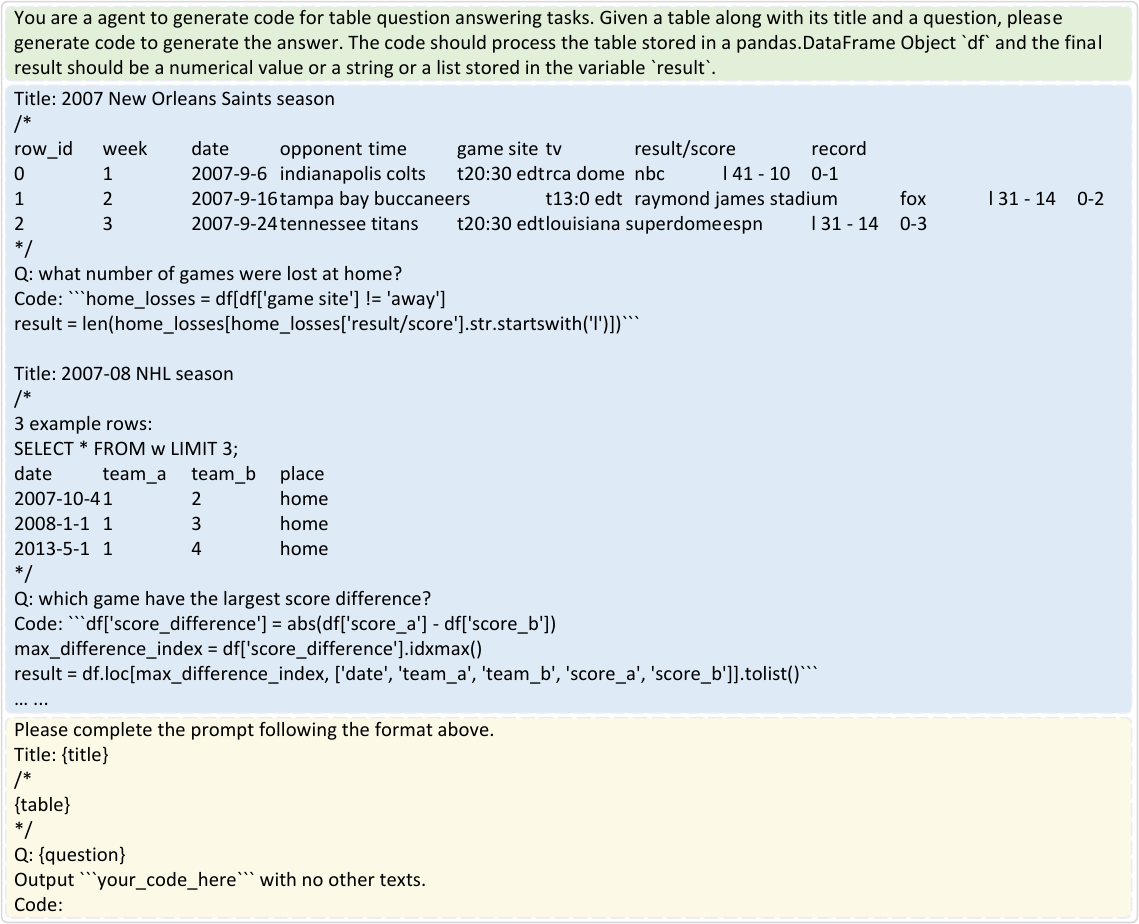}
    \vspace{-1em}
    \caption{Prompt of NL2Py on WikiTQ dataset.
    %, such as NL2SQL as shown in the figure. \sys decomposes the data prep process into three stages: \textcircled{1} The Planning stage, \textcircled{2} the Programming stage and \textcircled{3} the Executing stage.
    }
    \label{fig:prompt_nl2py_wikitq}
    % \vspace{-1em}
\end{figure*}
%!TEX root = ../../main.tex
\begin{figure*}[!t]
    \centering 
    \includegraphics[width=0.99\textwidth]{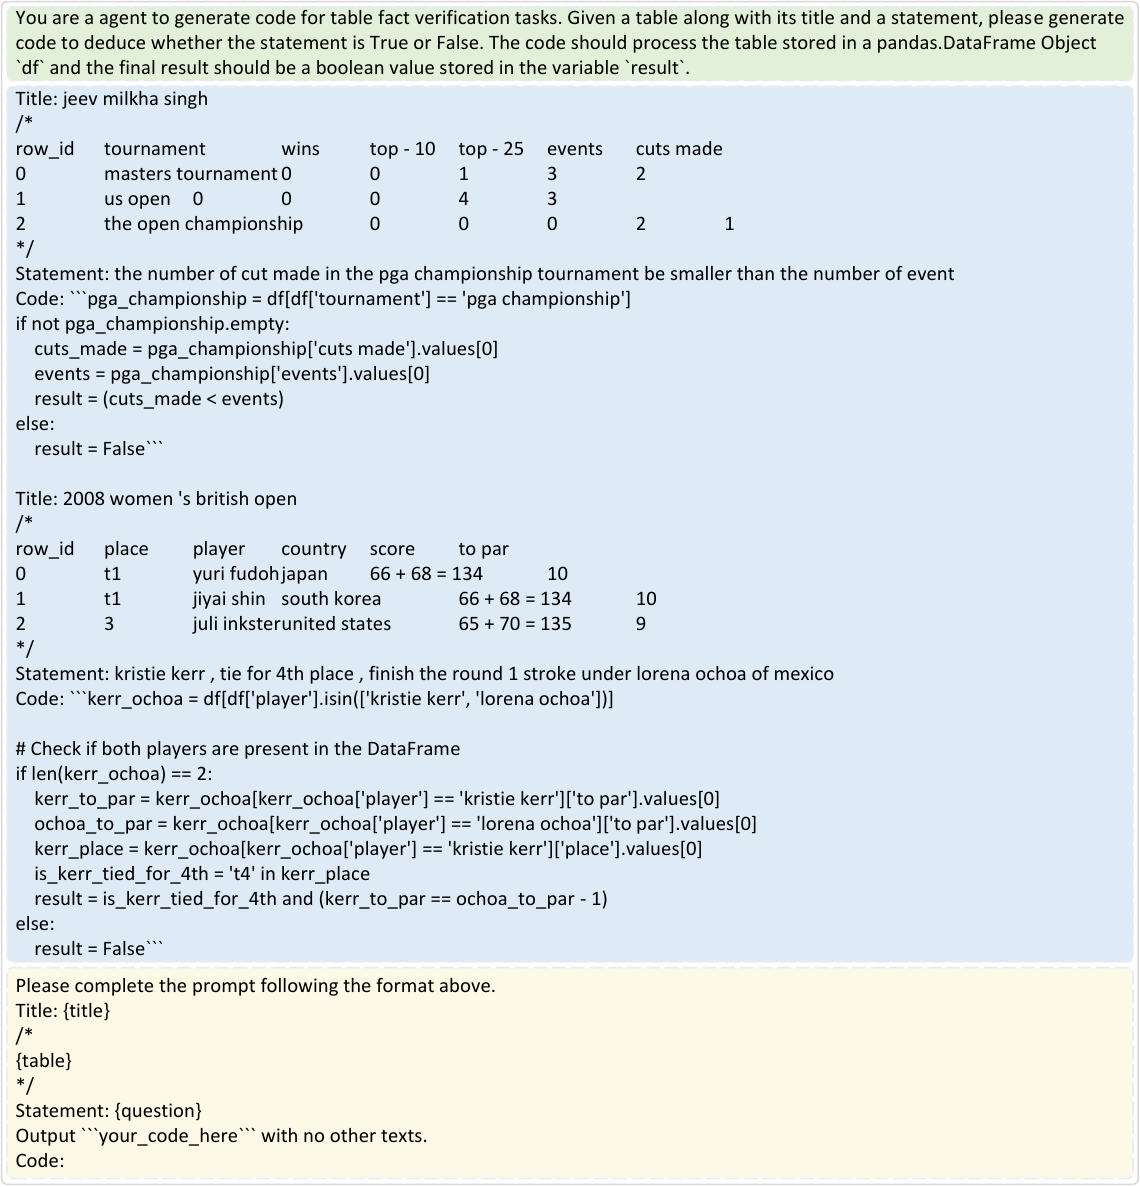}
    \vspace{-1em}
    \caption{Prompt of NL2Py on TabFact dataset.
    %, such as NL2SQL as shown in the figure. \sys decomposes the data prep process into three stages: \textcircled{1} The Planning stage, \textcircled{2} the Programming stage and \textcircled{3} the Executing stage.
    }
    \label{fig:prompt_nl2py_tabfact}
    % \vspace{-1em}
\end{figure*}

We also provide the prompts of implemented baselines, including
End2End (Figure~\ref{fig:prompt_end2end_wikitq} and Figure~\ref{fig:prompt_end2end_tabfact}),
CoT (Figure~\ref{fig:prompt_cot_wikitq} and Figure~\ref{fig:prompt_cot_tabfact}),
NL2SQL (Figure~\ref{fig:prompt_nl2sql_wikitq} and Figure~\ref{fig:prompt_nl2sql_tabfact}), NL2Py (Figure~\ref{fig:prompt_nl2py_wikitq} and Figure~\ref{fig:prompt_nl2py_tabfact})
and ICL-Prep (Figure~\ref{fig:prompt_iclprep_wikitq} and Figure~\ref{fig:prompt_iclprep_tabfact}). Some of the prompts are from existing works~\cite{cheng2023binding,chen2022large} as described in the experimental setup.
