# Supplementary material for: AutoPrep: Natural Language Question-Aware Data Preparation with a Multi-Agent Framework
Source: arXiv:2412.10422 source file (2025-07-09)
Supplement: Supplementary file 23 [file statistics_of_In_depth_analysis.tex]

\section{More Experiments}
\label{sec:statistics_of_in_depth_analysis}

\subsection{Evaluation on Various Table Sizes}

\stitle{Exp:
% \expnum\label{exp:evaluate_on_tables_with_various_sizes}
Evaluation of \sys on tables with various sizes.} 
To further investigate \sys, we analyze its performance across tables of varying sizes.
While all tables in TabFact are small, we categorize the tables in WikiTQ into Small (fewer than 2048 tokens), Medium (2048 to 4096 tokens), and Large (more than 4096 tokens), resulting in 4040 Small
tables, 200 Medium tables, and 104 Large tables.
The results are reported in Figure~\ref{fig:accuracy_on_different_size_tables}.

We observe that all baselines exhibit unstable performance, particularly on larger tables. For instance, although CoTable achieves the highest average accuracy among previous SOTA methods, it suffers an accuracy drop of {\textbf{11.78}} when reasoning over large tables. Likewise, ReAcTable shows relatively stable performance on medium tables (dropping by {\textbf{2.15}}), yet its performance on large tables remains unsatisfactory (dropping by {\textbf{17.53}}).

% %!TEX root = ../../main.tex
% % \begin{figure}[!t]
% %     \centering 
% %     \includegraphics[width=0.99\columnwidth]{plots/plot/comparison_of_methods_on_table_size.pdf}
% %     \vspace{-1em}
% %     \caption{}
% %     \label{fig:comparison_of_methods_on_table_size}
% %     \vspace{-1em}
% % \end{figure}

% \begin{figure}[!t]
%     % \vspace{-1em}
%     \centering
%     \begin{subfigure}{0.32\columnwidth}
%         \includegraphics[width=\textwidth]{plots/plot/accuracy_on_small_tables.pdf}
%         \captionsetup{skip=-0.3pt}
%         \caption{Small}
%         \label{fig:accuracy_on_small_tables}
%     \end{subfigure}
%     \hspace{0.2mm}
%     % \quad
%     \begin{subfigure}{0.32\columnwidth}
%         \includegraphics[width=\textwidth]{plots/plot/accuracy_on_medium_tables.pdf}
%         \captionsetup{skip=-0.3pt}
%         \caption{Medium}
%         \label{fig:accuracy_on_medium_tables}
%     \end{subfigure}
%     \hspace{0.2mm}
%     % \quad
%     \begin{subfigure}{0.32\columnwidth}
%         \includegraphics[width=\textwidth]{plots/plot/accuracy_on_large_tables.pdf}
%         \captionsetup{skip=-0.3pt}
%         \caption{Large}
%         \label{fig:accuracy_on_large_tables}
%     \end{subfigure}
%     \vspace{-2em}
%     \caption{\revise{Comparison of \sys and other data prep methods on tables with different sizes on the WikiTQ dataset.}}
%     \label{fig:comparison_of_methods_on_table_size}
%     \vspace{-1em}
% \end{figure}

%!TEX root = ../../main.tex
\begin{figure}[!t]
    \centering 
    \includegraphics[width=0.99\columnwidth]{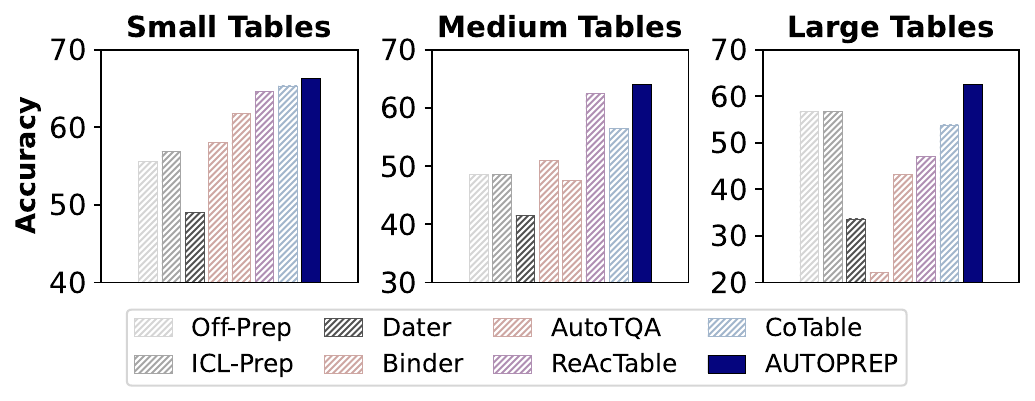}
    \vspace{-1em}
    \caption{{Accuracy on different size of tables in WikiTQ.}
    %, such as NL2SQL as shown in the figure. \sys decomposes the data prep process into three stages: \textcircled{1} The Planning stage, \textcircled{2} the Programming stage and \textcircled{3} the Executing stage.
    }
    \label{fig:accuracy_on_different_size_tables}
    % \vspace{-1em}
\end{figure}

In contrast, \sys achieves the highest and most stable performance across tables of varying sizes. When processing medium and large tables, the accuracy of \sys drops by {\textbf{2.29}} and {\textbf{3.79}}.
The key to its stability is that it employs specialized agents for each data prep task, mitigating the issue of exceeding prompt length limits. Furthermore, each agent generates program-based operators to handle data prep on the entire table, thereby avoiding information loss that occurs when large tables are cropped.

\stitle{Finding:
% \findingnum\label{finding:evaluate_on_tables_with_various_sizes}
By employing multiple agents and program-based operations, \sys maintains stable performance as table size grows, ensuring that each data prep task is handled effectively without overwhelming a single model.}

\subsection{Evaluation on Various Question Difficulties}

%!TEX root = ../main.tex
\begin{table}[t!]
  \centering
  \caption{\bf{In-depth Analysis of \sys and all baselines when varying question difficulties on WikiTQ and TabFact.}}
  \vspace{-0.5em}
  \scalebox{0.88} {
    \begin{tabular}{|c||c|c|c|c|}
      \hline
      \multirow{2}{*}{\textbf{Method}} & \multicolumn{2}{c|}{\textbf{WikiTQ}} & \multicolumn{2}{c|}{\textbf{TabFact}} \\ \cline{2-5}
                              & \textbf{Simple}                                                         & \textbf{Complex}    & \textbf{Simple}                                                         & \textbf{Complex}     \\
      \hline \hline
      End2End                 & ${57.80}$                                                    & ${55.68}$                                                               & $86.51$  & $77.07$             \\ \hline
      CoT                     & $56.85$                                                                & $55.33$                                                               & ${84.92}$                                                             & ${79.13}$            \\ \hline
      NL2Py                 & ${61.87}$                                                                & ${57.21}$                                                       & $70.83$                                                    & $65.45$  \\ \hline
      NL2SQL                  & $57.02$                                                                & $49.13$                                                               & $70.83$                                                    & $69.59$    \\
      \hline \hline
      ICL-Prep                & ${59.51}$                                                                & ${54.02}$                                                     & $82.64$                                                             & ${78.44}$     \\\hline
	  Dater                   & $51.33$                                                                & $45.77$                                                             & $88.39$ & $77.76$ 														           \\ \hline
      Binder                  & $62.02$                                                                & $52.04$                                                               & $89.29$                                                             & $76.38$                      \\ \hline
      ReAcTable               & ${66.98}$                                                                & ${61.71}$                                                   & ${90.48}$                                                 & ${79.72}$  \\ \hline
      CoTable                 & ${66.88}$                                                                & ${62.53}$                                                     & ${90.58}$                                                    & ${81.89}$     \\ 
      \hline \hline
      AP {\small + End2End}			 & $66.58$ 
								{\scriptsize \textcolor{cadmiumgreen}{($+8.78$)}}   
								& $60.23$ 
								{\scriptsize \textcolor{cadmiumgreen}{($+4.55$)}}             
								& $\underline{87.20}$ 
								{\scriptsize \textcolor{cadmiumgreen}{($+0.69$)}}           
								& $77.07$ 
								{\scriptsize \textcolor{cadmiumgreen}{($+0.00$)}}           
								\\ \hline
      {\small + CoT    }        & $64.12$ 
								{\scriptsize \textcolor{cadmiumgreen}{($+7.27$)}}   
								& $58.57$ 
								{\scriptsize \textcolor{cadmiumgreen}{($+5.24$)}}               
								& $84.52$ 
								{\scriptsize \textcolor{dropred}{($-0.40$)}}           
								& $80.02$ 
								{\scriptsize \textcolor{cadmiumgreen}{($+0.89$)}}             
								\\ \hline
      {\small + NL2Py}       		 & $\underline{68.09}$ 
								{\scriptsize \textcolor{cadmiumgreen}{($+6.22$)}}   
								& $\textbf{63.97}$ 
								{\scriptsize \textcolor{cadmiumgreen}{($+6.76$)}}     
								  & $\textbf{90.77}$ 
								  {\scriptsize \textcolor{cadmiumgreen}{($+19.94$)}} 
								  & $\underline{83.96}$ 
								  {\scriptsize \textcolor{cadmiumgreen}{($+18.51$)}}  
								  \\ \hline
      {\small + NL2SQL }         & $\textbf{69.17}$ 
								{\scriptsize \textcolor{cadmiumgreen}{($+11.97$)}}   
								& $\underline{63.50}$ 
								{\scriptsize \textcolor{cadmiumgreen}{($+14.37$)}}   
							  & $\textbf{90.77}$ 
							  {\scriptsize \textcolor{cadmiumgreen}{($+19.94$)}} 
							  & $\textbf{84.94}$ 
							  {\scriptsize \textcolor{cadmiumgreen}{($+15.35$)}}
							  \\
      \hline
    \end{tabular}
  }
   % \vspace{-1em}  
  \label{tbl:indepth_analysis_question_difficulty}
\end{table}

Also, following previous work~\cite{ye2023large,wang2024chain}, we compare \sys and all baseline models on questions with different difficulties.

\noindent
\textbf{Exp: How does \sys and other baselines perform on question with different difficulties?} We divide the TabFact dataset based on officially provided question difficulty labels. 
Since WikiTQ does not provide difficulty labels, we divide the dataset based on question length following previous work~\cite{ye2023large}.

As shown in Table~\ref{tbl:indepth_analysis_question_difficulty}, CoTable achieves the best performance among all baselines on both Simple and Complex questions, indicating its abilities of complex reasoning abilities over tables. While \sys still outperforms CoTable, especially on Complex questions. Specifically, \sys outperforms CoTable by 0.21\% on Simple questions and 3.72\% on Complex questions.

Moreover, notice that trivial performance improvement is achieved by \sys for Direct Prompting methods. Especially for CoT on Simple questions, the performance of CoT has been dropped by 0.47\% when integrated with \sys. This is because tables of TabFact are all small tables, data prep operations of \sys fail to bring obvious benefit for Direct Prompting methods. While for Code Generation methods, data quality is a critical problem. Thus, NL2Code and NL2SQL have achieved obvious performance gains on prepared tables.

\subsection{Impact of LLM-Based $\mathtt{CustomCode}$}

\begin{table}[t]
    \centering
    \caption{\bf{Analyzing LLM generated code for logical operator.}}
    \label{tbl:llm_code_for_op_analysis}
    \vspace{-0.5em}
    \resizebox{0.65\linewidth}{!}{
    \begin{tabular}{|c||c|}
        \hline
        \textbf{Method} & ~\textbf{WikiTQ}~  \\ \hline \hline
        $\mathtt{CustomCode}$ ratio & ${1.08\%}$  \\ \hline
        $\mathtt{CustomCode}$ accuracy & ${55.32\%}$ \\ \hline \hline
        
        \sys w. $\mathtt{CustomCode}$ & $\textbf{66.09}$\\ \hline
        \sys w.o. $\mathtt{CustomCode}$ & ${65.63}$  \\ 
        \hline
    \end{tabular}
    }
\end{table}

% 47 个case调用$\mathtt{CustomCode}$

\noindent
\stitle{Exp
% \expnum\label{exp:generalization_exp_new_physical_op}
: How does LLM-based $\mathtt{CustomCode}$ help \sys generalize to cases requiring new physical operations?} As discussed in Section~\ref{subsec:prog-idea}, we prompt the LLM to write code to implement the logical operation if no suitable function in the function pool can meet the requirement, which we denote as $\mathtt{CustomCode}$. We quantify the usage frequency of $\mathtt{CustomCode}$ and evaluate whether $\mathtt{CustomCode}$ produces the correct code on WikiTQ.
%its input and output using a powerful LLM DeepSeek-V3, calculating its accuracy. 
We also evaluate the performance of \sys without $\mathtt{CustomCode}$ design. 

As shown in Table~\ref{tbl:llm_code_for_op_analysis}, 
The results show that $\mathtt{CustomCode}$ is invoked in 1.08\% of cases, achieving an accuracy of 55.32\%. Notably, removing $\mathtt{CustomCode}$ leads to a performance drop of \textbf{0.46}  points (from 66.09 to 65.63). These results indicate that, despite its relatively low invocation frequency and moderate accuracy, $\mathtt{CustomCode}$ improves generalization of \sys, particularly in handling new or unforeseen physical operations.

%As shown in Table~\ref{tbl:llm_code_for_op_analysis}, \sys uses $\mathtt{CustomCode}$ with a frequency of 1.08\% and an accuracy of 55.32\% on WikiTQ. In addition, when ablating the $\mathtt{CustomCode}$, the performance of \sys on WikiTQ drops by 0.46. The experimental results show that the despite relatively low usage frequency and accuracy of $\mathtt{CustomCode}$, it still enhances the system's generalization especially in cases that require new physical operators.

\stitle{Finding 
% \findingnum\label{finding:generalization_exp_new_physical_op}
: $\mathtt{CustomCode}$ improves the generalization of \sys on cases requiring new physical operations.}

% \subsection{Evaluation on Generalizability}

% \input{tables/indepth_analysis_generalization}

\subsection{Analysis on Other Data Quality Issues}
\label{subsec_appendix:analysis_on_other_data_quality_issues}

We have conducted a \textbf{new experiment} to analyze the impact of missing values and duplication in TQA tasks on the WikiTQ dataset.
% (our main change \textbf{M\ref{modify:new-exps} (7)}). 

Specifically, for duplication, we first examine all tables containing duplicated records using a heuristic method from~\cite{fan2024cost} on the WikiTQ dataset, and only obtain 24 such instances. Then, we manually remove the duplicate records and re-evaluate \sys’s performance on the updated dataset. The results remain unchanged (accuracy: 70.83\% for both the original and de-duplicated datasets), suggesting that duplication is not a critical issue on existing TQA benchmarking datasets. Similarly, for missing values, we prompt LLMs to impute the missing entries based on the available data for all tables and then re-evaluate \sys on the imputated dataset. The results also show insignificant difference (65.00\% w/o imputation vs. 64.33\% with imputation), indicating that missing values have limited impact.

These above results suggest that such data preparation issues are uncommon and have little effect on existing TQA benchmarking datasets. This is largely due to the way of constructing the datasets. Specifically, during dataset construction~\cite{chen2019tabfact, pasupat2015compositional, wu2024tablebench}, annotators are instructed to first generate natural language questions based on a given table and then derive the corresponding answers directly from the same table. This construction paradigm implicitly ensures data completeness and consistency, as annotators tend to avoid crafting questions around missing or duplicating information. As a result, common data quality issues such as missing values and duplicate records are naturally excluded from the dataset, making them less relevant in the context of existing TQA tasks.

Nevertheless, we acknowledge that issues such as missing values and duplicates are common in real-world datasets, we leave the exploration of these broader data prep challenges to future work.

\stitle{Finding 
% \findingnum\label{finding:generalization_exp_new_physical_op}
: While issues such as missing values and duplicates are common in real-world datasets, they are significantly less prevalent than the three highlighted challenges in existing TQA benchmarks.}
